# Supplementary material for: Double Equivariance for Inductive Link Prediction for Both New Nodes and New Relation Types
Source: arXiv:2302.01313 source file (2025-01-14)
Supplement: Supplementary file 1 [file additinal_result.tex]

\subsubsection{\OurTask over FB237 and NELL}

We then modify link prediction task over solely new nodes to construct a real-world task to simulate the scenario when new nodes and new relation types are invented to existing {\ourgraphease}s. In our construction, we first pick a dataset with sufficient amount of relations from 12 benchmarks of link prediction over solely new nodes; Then, we uniformly discard 10\% relations from its training and validation triplets (remove triplets with those relations); Finally, in the test stage, we still keep all 100\% relations in observed triplets, but only keep test triplets with discarded 10\% relations. In our experiments, those hidden relations are $2\% \sim 11\%$ of original test inputs, and are $3\% \sim 14\%$ of original test target. The (Node \& Relation) Hits@10 result are shown in \Cref{tab:exp-discard}. %
For the naming of the dataset, as an example, we call our modified dataset FB237-V1 as FB237-V1-Discard to describe we discard $10\%$ of the relations in the training.

Our model \OurModel consistently and significantly perform better than other baselines, and is capable of performing such hard \ourtask on widely-used FB237 and NELL995 datasets with modifications.
One more finding is that pairwise baseline NBFNet* is mostly worse than a simple node-equivariant baseline GraphConv. We suppose the reason is that the unattributed link prediction knowledge learned from 90\% training relations does not always fit for the hidden 10\% relations, thus a more powerful baseline will more easily overfit on training, and may not perform well on test.

\begin{table}
\centering
\caption{{\bf (Node \& Relation) Hits@10 of training with 90\% relations, where test asks to predict the triplets over the discarded 10\% relations.} The suffix ``Discard'' means that some relations are discarded in training. ISDEA is consistently better than other baselines.}
\resizebox{0.8\linewidth}{!}{
\begin{tabular}{l|c|cccc|c}
    \hline
    {Dataset} & {Rand} & GAT & GIN & GraphConv  & NBFNet* & \OurModel \\
    \hline
    FB237-V1-Discard & 20.00 & 13.79{\scriptsize $\pm 00.01$} &20.11{\scriptsize $\pm 04.06$} & \underline{25.86}{\scriptsize $\pm 01.41$} & 22.77{\scriptsize $\pm 02.21$} & \textbf{59.20} {\scriptsize $\pm 06.50$} \\
    FB237-V2-Discard & 20.00 & 14.81{\scriptsize $\pm 02.36$} & 24.54{\scriptsize $\pm 04.29$}& \underline{24.54}{\scriptsize $\pm 02.36$}& 17.69 {\scriptsize $\pm 00.50$} & \textbf{57.87} {\scriptsize $\pm 01.31$} \\
    NELL995-V2-Discard & 20.00 & 11.90{\scriptsize $\pm 04.45$} &26.19{\scriptsize $\pm 04.45$} & \underline{27.38}{\scriptsize $\pm 08.42$} & 15.36{\scriptsize $\pm 01.93$} & \textbf{48.81} {\scriptsize $\pm 03.37$} \\
    NELL995-V3-Discard & 20.00 & 18.92{\scriptsize $\pm 02.92$} & 28.60{\scriptsize $\pm 04.82$}& \underline{34.23}{\scriptsize $\pm 02.49$}& 19.22 {\scriptsize $\pm 00.53$} & \textbf{73.42} {\scriptsize $\pm 05.64$} \\

    NELL995-V4-Discard & 20.00 & 11.11{\scriptsize $\pm 04.16$} & 20.00{\scriptsize $\pm 05.44$}& \underline{27.78}{\scriptsize $\pm 07.86$}& 16.07 {\scriptsize $\pm 00.16$} & \textbf{50.00} {\scriptsize $\pm 04.71$} \\

    \hline

\end{tabular}
}
\vspace{5pt}
\label{tab:exp-discard}
\vspace{-10pt}
\end{table}
