# Supplementary material for: Double Equivariance for Inductive Link Prediction for Both New Nodes and New Relation Types
Source: arXiv:2302.01313 source file (2025-01-14)
Supplement: Supplementary file 2 [file additional_theory.tex]

\section{Additional Theoretical Concepts}
\label{appd:add-theory}

In \Cref{def:rel-graph-iso} we defined isomorphisms between {\ourgraphs} via node and relation permutations, and in \Cref{def:rel-graph-repr} we defined \ourequiv\ \ourgraphease representations that are equivariant to such permutations. It is important to point out, for the completeness of the theory, that the successful application of \ourequiv representations to \ourtask task hinges upon the assumption that the underlying {\ourgrapheases} possess what we call the \ourexchngnoun property:
\begin{definition}[Double exchangeability for {\ourgraphs}]
\label{def:rel-graph}
We define a double exchangeable \ourgraph $\adjwild$ to be a \ourgraph (\Cref{subsec:taskdef}) $\adjwild \in \sA$ sampled as $\adjwild \sim \mu$, where $\mu$ is some unknown data distribution such that $\mu(\adj^{(G)} = \mu(\adj^{(H)})$ for any isomorphic \ourgraph $\adj^{(G)}$ and $\adj^{(H)}$ ($\adj^{(G)}\simeq_\text{RL} \adj^{(H)}$ as in \Cref{def:rel-graph-iso}).
In this paper we denote this property of $\mu$ as {\em \ourexchngnoun}.   
\end{definition}

In other words, a double exchangeable \ourgraph is a graph where its isomorphic version is just as likely to appear from the real-world data distribution as itself. For example, one can say the {\ourgraphs} in the \ourdata dataset~(\Cref{sec:exp}) are (roughly) double exchangeable, e.g., the EN graph (English version of DBPedia) and the FR graph (French version of DBPedia) are (roughly) isomorphic and have the same data likelihood because they describe essentially the same graph (DBPedia), albeit using entity and relation labels in different languages.
