# Supplementary material for: Double Equivariance for Inductive Link Prediction for Both New Nodes and New Relation Types
Source: arXiv:2302.01313 source file (2025-01-14)
Supplement: Supplementary file 3 [file compare_with_transductive.tex]

\paragraph{Compare with Transductive performance} We are also interested in exploring the performance of inductive \ourtask compared to transductive link prediction in our data \ourdata. In the inductive scenario, we train the model on one graph and test it on another graph for each pairs of the graph in our dataset. However, in the transductive scenario, we train a model on a specific graph and test its performance on the same graph. Here we would like to investigate how the performance of the model differs between these two scenarios. We present the results in \Cref{tab:pediatypes-trans}, where EN-FR Ind means training on EN and test on FR, and Trans means training on FR and test on FR. The same rule applies to other dataset names.

As we can see from the \Cref{tab:pediatypes-trans}, our model ISDEA achieves very close results from \ourtask to transductive, which showcase the capability of our model to perform the \ourtask on both new nodes and new relations. An interesting observation is that the performance of \OurModel %
over the same relational data with different languages (e.g., EN-DE) achieves closer results to transductive than over different databases (e.g., WD-DB), which indicates that the underlying multigraphs of different languages on DBPedia have more similar strutural relations than between the multigraphs of DBPedia and YAGO.

\begin{figure}
\begin{minipage}{1\textwidth}
\centering
{
\vspace{-10pt}
\subcaption{{\bf { PediaTypes Version 1}}}
\resizebox{0.7\linewidth}{!}{
\begin{tabular}{l|l|cccc}
    \hline
    \multicolumn{2}{c|}{Dataset}  & MRR & Hits@1 & Hits@5 & Hits@10    \\
    \hline
    \multirow{2}{*}{EN-FR} & Ind & 58.57{\scriptsize $\pm 00.52$} & 49.02{\scriptsize $\pm 00.22$} & 68.42{\scriptsize $\pm 00.87$} & 78.91{\scriptsize $\pm 01.26$} \\
    & Trans & 58.35{\scriptsize $\pm 00.91$} & 48.43{\scriptsize $\pm 00.89$} & 69.34{\scriptsize $\pm 01.05$} & 80.09{\scriptsize $\pm 02.18$}
    \\
\hline
    \multirow{2}{*}{FR-EN} & Ind & 56.53{\scriptsize $\pm 01.21$} & 46.20{\scriptsize $\pm 01.02$} & 66.95{\scriptsize $\pm 02.18$} & 78.30{\scriptsize $\pm 02.12$} \\
    & Trans & 59.25{\scriptsize $\pm 00.77$} & 49.13{\scriptsize $\pm 00.80$} & 70.30{\scriptsize $\pm 00.93$} & 79.86{\scriptsize $\pm 01.48$}
    \\
\hline
    \multirow{2}{*}{EN-DE} & Ind & 60.31{\scriptsize $\pm$ 01.50} & 44.27{\scriptsize $\pm$ 01.84} & 80.95{\scriptsize $\pm$ 00.90} & 87.32{\scriptsize $\pm$ 00.70} \\
    & Trans & 62.28{\scriptsize $\pm$ 00.96} & 47.04{\scriptsize $\pm$ 00.65} & 81.51{\scriptsize $\pm$ 01.66} & 89.75{\scriptsize $\pm$ 01.77}
    \\
\hline
    \multirow{2}{*}{DE-EN} & Ind & 62.92{\scriptsize $\pm$ 01.12} & 46.78{\scriptsize $\pm$ 00.95} & 84.24{\scriptsize $\pm$ 01.51} & 91.98{\scriptsize $\pm$ 00.84} \\
    & Trans & 63.20{\scriptsize $\pm$ 00.50} & 46.61{\scriptsize $\pm$ 00.88} & 85.42{\scriptsize $\pm$ 00.37} & 92.22{\scriptsize $\pm$ 00.68} 
    \\
\hline
    \multirow{2}{*}{DB-WD} & Ind & 44.21{\scriptsize $\pm$ 09.18} & 33.41{\scriptsize $\pm$ 09.07} & 53.98{\scriptsize $\pm$ 09.60} & 66.65{\scriptsize $\pm$ 09.21}  \\
    & Trans & 54.08{\scriptsize $\pm$ 00.85} & 44.17{\scriptsize $\pm$ 01.08} & 63.36{\scriptsize $\pm$ 01.12} & 72.84{\scriptsize $\pm$ 02.90} 
    \\
\hline
    \multirow{2}{*}{WD-DB} & Ind & 57.07{\scriptsize $\pm$ 00.91} & 46.25{\scriptsize $\pm$ 00.39} & 69.24{\scriptsize $\pm$ 02.40} & 76.91{\scriptsize $\pm$ 02.92}  \\
    & Trans & 56.96{\scriptsize $\pm$ 01.39} & 45.58{\scriptsize $\pm$ 02.17} & 69.55{\scriptsize $\pm$ 00.92} & 80.39{\scriptsize $\pm$ 00.85}
    \\
\hline
    \multirow{2}{*}{DB-YG} & Ind & 53.38{\scriptsize $\pm$ 01.72} & 38.11{\scriptsize $\pm$ 02.39} & 75.42{\scriptsize $\pm$ 00.65} & 85.46{\scriptsize $\pm$ 00.31} \\
    & Trans & 50.09{\scriptsize $\pm$ 02.29} & 33.12{\scriptsize $\pm$ 02.78} & 74.34{\scriptsize $\pm$ 01.20} & 86.32{\scriptsize $\pm$ 01.49}
    \\
\hline
    \multirow{2}{*}{YG-DB} & Ind & 45.33{\scriptsize $\pm$ 02.39} & 32.87{\scriptsize $\pm$ 02.48} & 59.33{\scriptsize $\pm$ 03.09} & 66.45{\scriptsize $\pm$ 03.98}  \\
    & Trans & 51.80{\scriptsize $\pm$ 00.73} & 40.30{\scriptsize $\pm$ 00.72} & 65.51{\scriptsize $\pm$ 01.18} & 73.02{\scriptsize $\pm$ 01.67}
    \\
\hline

\end{tabular}
}
}
\\
\vspace{-5pt}
{
\subcaption{{\bf { PediaTypes Version 2}}}
\resizebox{0.7\linewidth}{!}{
\begin{tabular}{l|l|cccc}
    \hline
    \multicolumn{2}{c|}{Dataset}  & MRR & Hits@1 & Hits@5 & Hits@10    \\
    \hline
    \multirow{2}{*}{EN-FR} & Ind & 57.20{\scriptsize $\pm$ 00.64} & 47.69{\scriptsize $\pm$ 00.43} & 66.16{\scriptsize $\pm$ 01.16} & 76.45{\scriptsize $\pm$ 02.79}  \\
    & Trans & 56.85{\scriptsize $\pm$ 00.05} & 47.37{\scriptsize $\pm$ 00.43} & 65.63{\scriptsize $\pm$ 00.54} & 74.90{\scriptsize $\pm$ 02.27}
    \\
\hline
    \multirow{2}{*}{FR-EN} & Ind & 55.74{\scriptsize $\pm$ 00.34} & 44.53{\scriptsize $\pm$ 00.41} & 66.87{\scriptsize $\pm$ 00.46} & 76.57{\scriptsize $\pm$ 02.04}  \\
    & Trans & 58.57{\scriptsize $\pm$ 00.18} & 48.50{\scriptsize $\pm$ 00.37} & 68.36{\scriptsize $\pm$ 00.58} & 78.30{\scriptsize $\pm$ 02.76}
    \\
\hline
    \multirow{2}{*}{EN-DE} & Ind & 56.77{\scriptsize $\pm$ 03.01} & 40.52{\scriptsize $\pm$ 04.30} & 78.42{\scriptsize $\pm$ 00.95} & 88.23{\scriptsize $\pm$ 00.69} \\
    & Trans & 59.77{\scriptsize $\pm$ 00.60} & 44.74{\scriptsize $\pm$ 00.77} & 79.52{\scriptsize $\pm$ 00.25} & 88.07{\scriptsize $\pm$ 00.10}
    \\
\hline
    \multirow{2}{*}{DE-EN} & Ind & 59.00{\scriptsize $\pm$ 00.57} & 44.24{\scriptsize $\pm$ 00.51} & 78.10{\scriptsize $\pm$ 00.64} & 89.22{\scriptsize $\pm$ 01.51}  \\
    & Trans & 56.14{\scriptsize $\pm$ 03.75} & 40.31{\scriptsize $\pm$ 04.41} & 76.81{\scriptsize $\pm$ 02.61} & 90.13{\scriptsize $\pm$ 00.67} 
    \\
\hline
    \multirow{2}{*}{DB-WD} & Ind & 41.76{\scriptsize $\pm$ 07.29} & 30.10{\scriptsize $\pm$ 07.51} & 53.30{\scriptsize $\pm$ 07.76} & 66.29{\scriptsize $\pm$ 06.55}   \\
    & Trans & 50.37{\scriptsize $\pm$ 00.64} & 39.52{\scriptsize $\pm$ 00.40} & 61.64{\scriptsize $\pm$ 01.07} & 73.59{\scriptsize $\pm$ 01.80}
    \\
\hline
    \multirow{2}{*}{WD-DB} & Ind & 54.59{\scriptsize $\pm$ 01.03} & 43.44{\scriptsize $\pm$ 01.57} & 66.99{\scriptsize $\pm$ 01.02} & 75.66{\scriptsize $\pm$ 00.97}  \\
    & Trans & 58.16{\scriptsize $\pm$ 00.25} & 47.70{\scriptsize $\pm$ 00.12} & 70.04{\scriptsize $\pm$ 00.97} & 79.05{\scriptsize $\pm$ 00.40} 
    \\
\hline
    \multirow{2}{*}{DB-YG} & Ind & 47.94{\scriptsize $\pm$ 01.29} & 32.24{\scriptsize $\pm$ 01.71} & 66.91{\scriptsize $\pm$ 00.63} & 83.88{\scriptsize $\pm$ 01.36}  \\
    & Trans & 48.14{\scriptsize $\pm$ 00.14} & 33.08{\scriptsize $\pm$ 00.13} & 66.70{\scriptsize $\pm$ 00.77} & 83.49{\scriptsize $\pm$ 00.49}
    \\
\hline
    \multirow{2}{*}{YG-DB} & Ind & 47.62{\scriptsize $\pm$ 04.39} & 33.02{\scriptsize $\pm$ 04.61} & 65.45{\scriptsize $\pm$ 03.95} & 78.45{\scriptsize $\pm$ 02.96}   \\
    & Trans & 54.56{\scriptsize $\pm$ 00.30} & 40.53{\scriptsize $\pm$ 00.63} & 72.45{\scriptsize $\pm$ 00.15} & 84.65{\scriptsize $\pm$ 00.59} 
    \\
\hline

\end{tabular}
}
}
\captionof{table}{
{\bf (Node \& Relation) Performance on \OurTask tasks against Transductive task over \ourdata for ISDEA.} %
The dataset name ``$X$-$Y$'' Ind means training on graph $X$ and test on graph $Y$, and Trans means training on graph $Y$ and test on graph $Y$.
\OurModel achieves close results in \ourtask compared to the transductive results. %
}
\label{tab:pediatypes-trans}
\vspace{-5pt}
\end{minipage}
\end{figure}
