# Supplementary material for: Double Equivariance for Inductive Link Prediction for Both New Nodes and New Relation Types
Source: arXiv:2302.01313 source file (2025-01-14)
Supplement: Supplementary file 4 [file exp_doubly_task.tex]

\subsection{\Ourtask task over both new nodes and new relation types}
In this section, we provide more detailed experiment results and analysis for our method on inductively \ourtask on both new nodes and new relation types. 
%Different from the previous task, \ourtask on both new nodes and new relation types will ensure test relation types are different from training relation types.

{\bf Datasets.}
To the best of our knowledge, there are no existing real-world benchmarks that are specially designed to test a model's extrapolation capability for \ourtask task by training the model on one graph and testing it on another completely new graph coming from different domains and distributions. 
Existing datasets %where the set of node and relation types in test are disjoint from those in training, 
such as NL-100, WK-100, and FB-100 from~\citet{ingram} are typically created by randomly splitting a larger graph (e.g. NELL-995~\citep{xiong2018one}, Wikidata68K~\citep{gesese2022raild}, FB15K237~\citep{toutanova2015observed}) into disjoint node and relation sets, implying that the test and training graphs still come from the same distribution. %possess similar characteristics. 
In contrast, we purposefully create two \ourtask benchmark datasets: \ourdata and WikiTopics, sampled respectively from the OpenEA library~\citep{OpenEA} and WikiData-5M~\citep{wang2021kepler}, where by design the test and training graphs are either from different domains or different topic groups and are likely to possess different characteristics to fully test model's capability for \ourtask. We also propose another task with modifications of the NL-$k$, WK-$k$, and FB-$k$ datasets from InGram~\citep{ingram} and one synthetic task FD2 to study the expressive power of \OurModel.

%\paragraph{Datasets.}
%To the best of our knowledge, there are no existing real-world benchmarks where the test \ourgraphease is formed of entirely new nodes and new relation types not available during training. Thus, to test full capabilities of our model, we first propose one synthetic task FD2 and another task with modifications of NELL995 and FB237 dataset. Then we create two \ourtask benchmark datasets: \ourdata and WikiTopics, sampled respectively from the OpenEA library~\citep{OpenEA} and WikiData-5M \citep{wang2021kepler}.

\subsubsection{Experiment Setup}

\paragraph{Baselines.}
To the best of our knowledge, InGram~\citep{ingram} is the first and only work capable of performing \ourtask without needing significant modification to the model. Hence, we chose InGram as one baseline. 
We also run RMPI~\citep{geng2023relational}, which is capable of reasoning over new nodes and new relations but requires extra context at test time (test graphs either contain training relations or ontological information of unseen relations). We simply provide randomized embeddings of unseen relations at test time following \citet{ingram}.
In addition, we consider the state-of-the-art link prediction model NBFNet~\citep{zhu2021neural} capable of generalizing over to new nodes but not new relations and modifying its architecture to work with new relations at test time by providing randomized embeddings of unseen relations at test time following \citet{ingram}. We also compare our models with message-passing GNNs including GAT~\citep{velivckovic2017graph}, GIN~\citep{xu2018powerful}, GraphConv~\citep{Morris2019WL} which treats the graph as a homogeneous graph by ignoring the relation types. 
For fair comparisons, we add distance features as in \Cref{eq:dssrepr} to increase the expressiveness of these GNNs. 
%To the best of our knowledge, there is no prior work capable of performing the \ourtask task in \Cref{def:task-double}. Thus, we compare \OurModel with unattributed link prediction models. Specifically, we compare with message-passing GNNs including GAT~\citep{velivckovic2017graph}, GIN~\citep{xu2018powerful}, GraphConv~\citep{Morris2019WL}, and SOTA pair-wise link prediction model NBFNet~\citep{zhu2021neural}. For fair comparison, we add distance features as in \Cref{eq:dssrepr} to increase expressiveness of the message-passing GNNs, and only use unattributed NBFNet (denoted as NBFNet*, by replacing relation embedding for every relation $r$ with a single sharing embedding across all relations), as attributed NBFNets learn relational embeddings and are not able to generalize to new relation types in test. 
For training of each single run, we augment each triplet $(i, k, j)$ by its inversion $(i, k^{-1}, j)$, and sample 2 negative (node) triplets $(i', k, j')$ and 2 negative (relation) triplets $(i,k',j)$ per positive in training as \citet{sun2018rotate,zhu2021neural}. Training was performed on NVidia A100s, L4s, GeForce RTX 2080 Ti, and TITAN V GPUs.

\paragraph{Evaluation Metrics.} We sample $50$ negative triplets for each test positive triplet during test evaluation by corrupting either nodes or relation types (\Cref{eq:loss}), and use Nodes Hits@$k$ and Relation Hits@$k$ separately which counts the ratio of positive triplets ranked at or above the $k$-th place against the $50$ negative samples as evaluation metric over $5$ runs. Specifically, for Node prediction evaluation, we sample without replacement $50$ negative tail (or head) nodes, and for Relation prediction evaluation, we sample with replacement $50$ negative relation types (can also handle cases where the number of test relations is less than $50$). We also report other widely used metrics such as MRR.%

\paragraph{Hyperparameters and Implementation Details.}
For homogeneous GNN methods, NBFNet and \update{\OurNewModel}, We follow the same configuration as \citet{teru2020inductive} such that the hidden layers have 32 neurons. We use Adam optimizer with grid search over learning rate $\alpha\in \{0.01,0.001,0.0001\}$, and over weight decay $\beta\in\{0.0005,0\}$. For all datasets, we train these models for 10 epochs with a mini-batch size of 16. %If the model is not improving for 15 epochs, we early stop the training. For all methods, number of hops and number of layers are 2 on FD-1, and are 3 on real-world inductive \ourgraphease completion to ensure fair comparison. 
% We choose hidden layers to have 32 neurons, use Adam optimizer with learning rate 0.01, and weight decay 5e-4. For all dataset, we train our model 10 epochs with batch size 16. %
For the GNN kernel \update{we choose GCN~\citep{Kipf2016}} of \update{\OurNewModel}. For these models, the number of hops and number of layers are 2 on FD-2, and 3 on all other datasets to ensure fair comparison.

Since NBFNet is designed to only perform inductive link prediction with solely new nodes and utilizes trained relation embeddings, we use randomly initialized embeddings for the unseen relation types at test time to enable it for performing \ourtask.

To run InGram~\citep{ingram} on \ourdata and \ourotherdata, we conduct hyperparameter search over the configurations of ranking loss margin $\gamma \in \{ 1.0, 2.0 \}$, learning rate $\alpha \in \{ 0.0005, 0.001 \}$, number of entity layers $L \in \{ 2, 3, 4 \}$, and number of entity layers $\hat{L} \in \{ 2, 3, 4 \}$. For other hyperparameters, we use the suggested values from~\citet{ingram} and their codebase, such as the number of bins $B = 10$ and the number of attention heads $K = 8$. We then use the overall best-performing hyperparameters on \ourdata and the best-performing hyperparameters on \ourotherdata to run InGram on all tasks in \ourdata and all tasks in \ourotherdata respectively. For running on the (modified) NL-$k$, WK-$k$, and FB-$k$ datasets from~\citet{ingram}, we use the provided hyperparameters for each task from the authors.

To run \OurOtherModel, we use the same trained checkpoints of InGram. The difference is at inference time, where instead of a single forward pass with one sample of randomly initialized entity and relation embeddings for InGram, we draw 10 samples of initial entity and relation embeddings and run 10 forward passes. This yields 10 Monte Carlo samples of the triplet scores, which we then use to compute the \OurOtherModel triplet scores according to~\Cref{eq:de-ingram}.

For RMPI~\citep{geng2023relational}, we use the provided hyperparameters from the codebase and run the RMPI-NE version of the model with a concatenation-based fusion function, which generally has the best performance reported in~\citet{geng2023relational}. We note that, since our \ourgraphease does not contain ontological information over the unseen relation types of the test graphs, we instead provide the model with randomly initialized embeddings for the unseen relation types to perform \ourtask.

\subsubsection{\Ourtask over \ourdata}
\label{appx:exp-pediatype}

As discussed in \Cref{sec:exp}, we create our own \ourtask benchmark dataset \ourdata. Each graph in \ourdata is sampled from a graph in the OpenEA library~\citep{OpenEA} (under GPL-3.0 license).
OpenEA~\citep{OpenEA} library provides multiple pairs of \ourgraphease, each pair of which is a database containing similar topics.
Each node of a graph corresponds to the Universal Resource Identifier (URI) of an entity in the database, e.g., ``{\em http://dbpedia.org/resource/E399772}'' from English DBPedia.
Each relation type of a graph corresponds to the URI of a relation in the database, e.g., ``{\em http://dbpedia.org/ontology/award}'' from English DBPedia.
Moreover, since each pair of graphs describes similar topics, most entities and relations are highly related, e.g., ``{\em http://dbpedia.org/resource/E678522}'' from English and ``{\em http://fr.dbpedia.org/resource/E415873}'' from French are indeed the same thing, except that the labeling is different. \update{These multilingual KGs predominantly use English for relation labels, which causes an overlap in relations. However, in our experimental setup, we treat relations as if they were in different languages and do not leverage this overlapping information during model training.} Thus, we would expect a powerful model that is insensitive to node and relation type labelings to be able to learn on one graph of the pair and perform well on the other graph of the same pair.

To control the size under a feasible limitation, we use the same subgraph sampling algorithm as GraIL~\citep{teru2020inductive}, which proposes link prediction benchmarks over solely new nodes. Details are provided in \Cref{alg:sample-deg}. For each pair of graphs from the OpenEA library, e.g., English-to-French DBPedia, we first apply the sampling algorithm as in \Cref{alg:sample-deg} on each graph to reduce the size of each graph. Then we randomly split querying triplets given by the \Cref{alg:sample-deg} into 80\% training, 10\% validation, and 10\% test for each graph. Finally, to construct the task where we learn on English DBPedia but test on French DBPedia (denoted as EN-FR), we pick training and validation triplets from the English graph for model tuning, and only use test triplets from the French graph for model evaluation; Similarly, for task from French to English (FR-EN), we pick training and validation triplets from French graph for model tuning, and only use test triplets from English graph for model evaluation. The {\bf dataset statistics} for \ourdata are summarized in \Cref{fig:stats-pediatype}.

\begin{figure}
\centering
\begin{minipage}{0.24\textwidth}
\centering
\resizebox{\linewidth}{!}{
\begin{tabular}{l|cc}
\hline
& DBPedia & Wikidata \\
\hline
\#Nodes & 4906 & 4948\\
\#Relations & 144 & 102 \\
\#Triplets (Obv.) & 17593 & 23888 \\
\#Triplets (Qry.) & 1666 & 2456 \\
\#Avg. Deg. & 7.85 & 10.65 \\
\hline
\end{tabular}
}
\includegraphics[width=\linewidth]{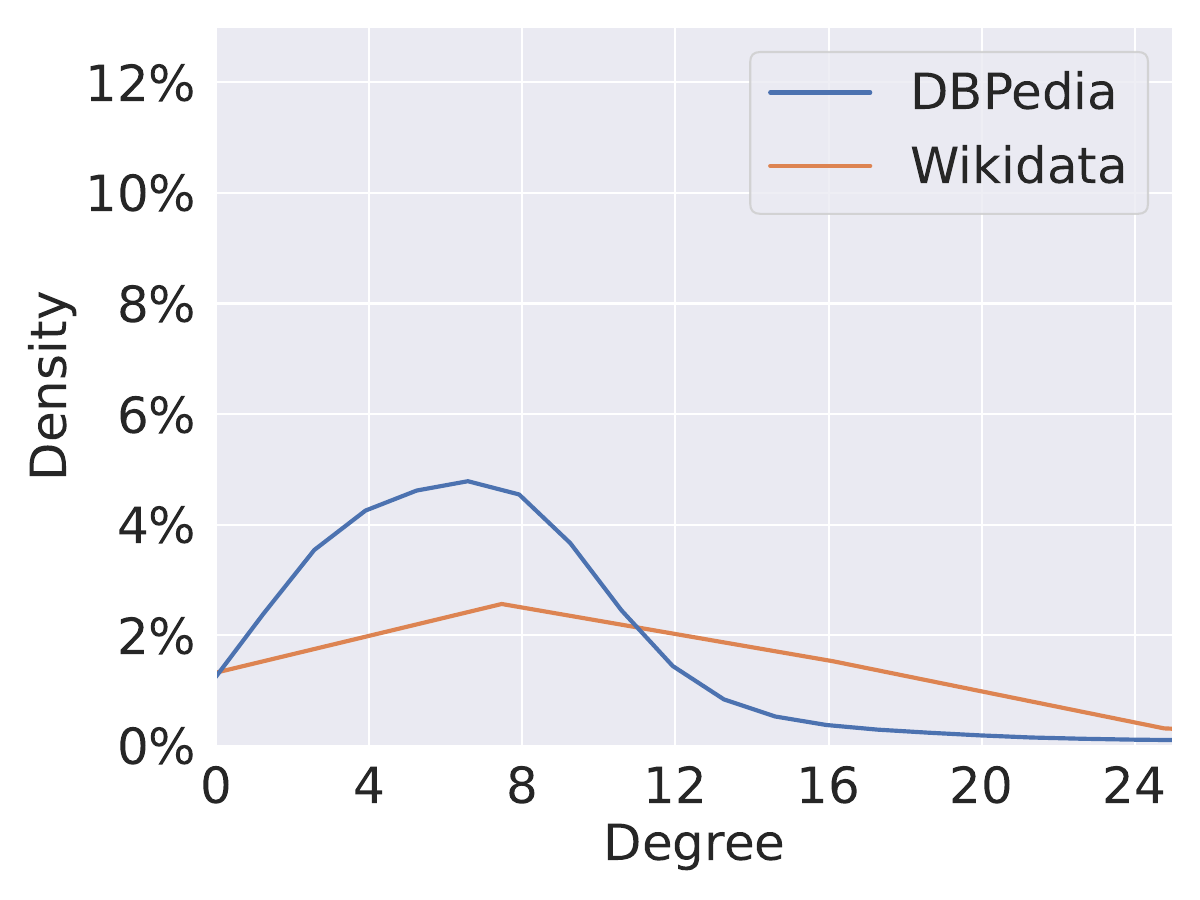}
\subcaption{DB$\longleftrightarrow$WD}
\end{minipage}
\hfill
\begin{minipage}{0.24\textwidth}
\centering
\resizebox{\linewidth}{!}{
\begin{tabular}{l|cc}
\hline
& DBPedia & YAGO \\
\hline
\#Nodes & 4795 & 4751 \\
\#Relations & 64 & 17 \\
\#Triplets (Obv.) & 13248 & 11327 \\
\#Triplets (Qry.) & 1177 & 973 \\
\#Avg. Deg. & 6.02 & 5.18 \\
\hline
\end{tabular}
}
\includegraphics[width=\linewidth]{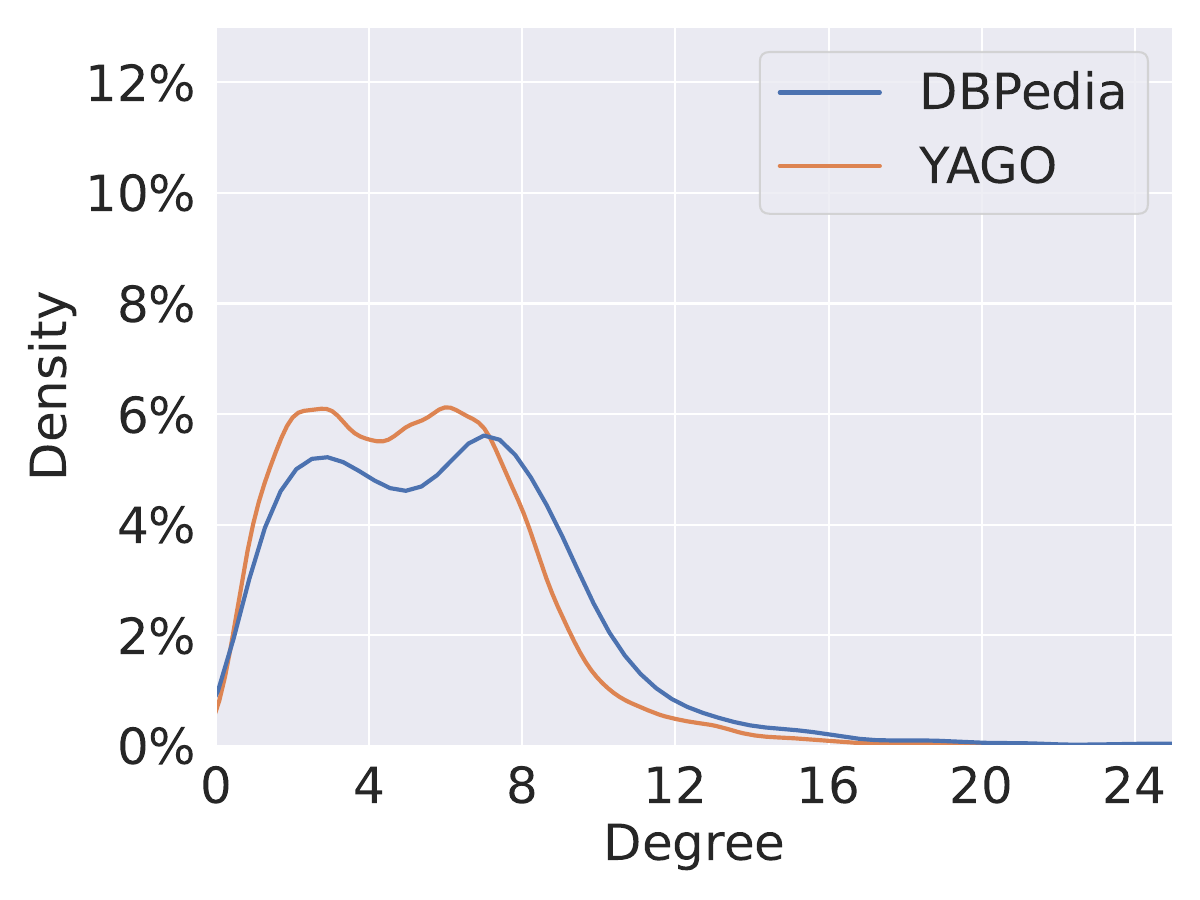}
\subcaption{DB$\longleftrightarrow$YG}
\end{minipage}
\hfill
\begin{minipage}{0.24\textwidth}
\centering
\resizebox{\linewidth}{!}{
\begin{tabular}{l|cc}
\hline
& English & French \\
\hline
\#Nodes & 4962 & 4933 \\
\#Relations & 122 & 101 \\
\#Triplets (Obv.) & 30876 & 24165 \\
\#Triplets (Qry.) & 3326 & 2485 \\
\#Avg. Deg. & 13.79 & 10.81 \\
\hline
\end{tabular}
}
\includegraphics[width=\linewidth]{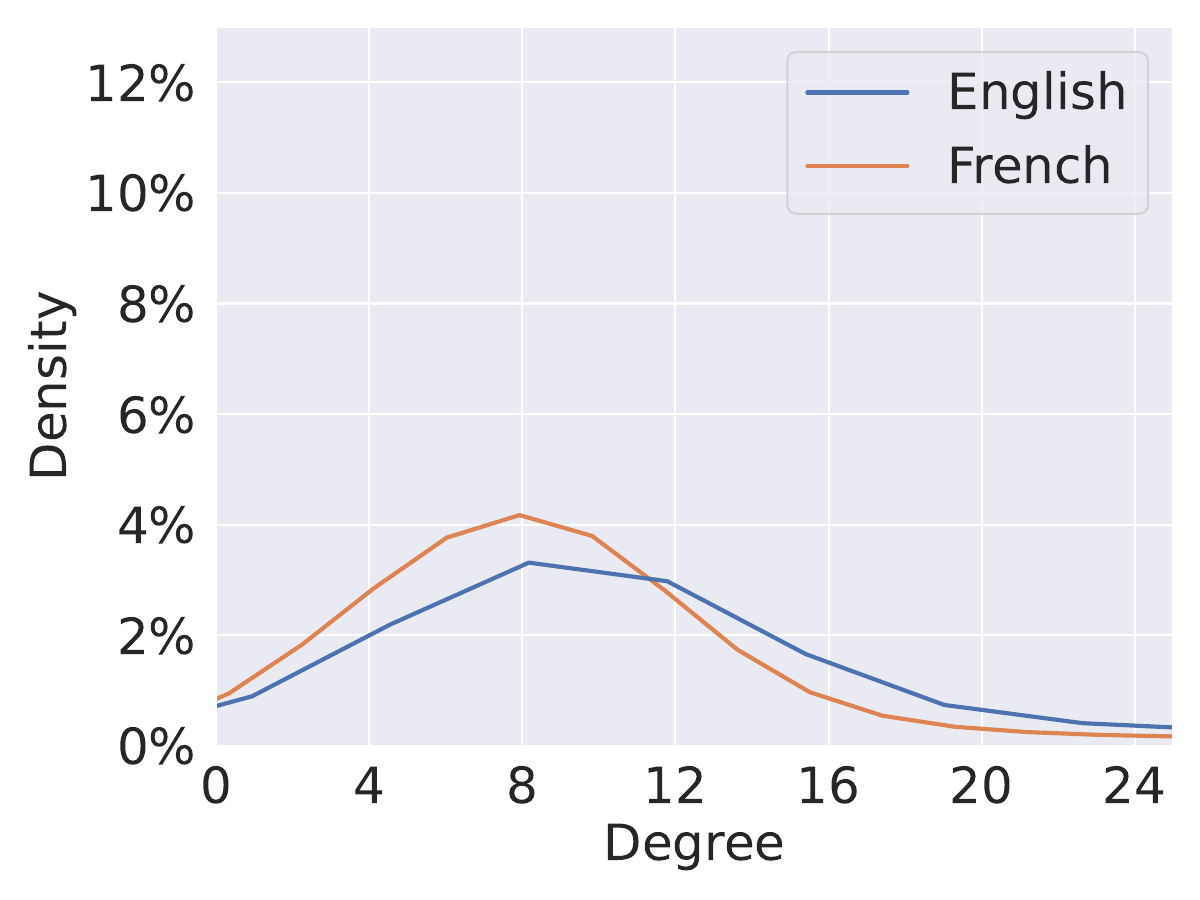}
\subcaption{EN$\longleftrightarrow$FR}
\end{minipage}
\hfill
\begin{minipage}{0.24\textwidth}
\centering
\resizebox{\linewidth}{!}{
\begin{tabular}{l|cc}
\hline
& English & German \\
\hline
\#Nodes & 4890 & 4915 \\
\#Relations & 121 & 67 \\
\#Triplets (Obv.) & 25177 & 29011 \\
\#Triplets (Qry.) & 2626 & 3100 \\
\#Avg. Deg. & 11.37 & 13.07 \\
\hline
\end{tabular}
}
\includegraphics[width=\linewidth]{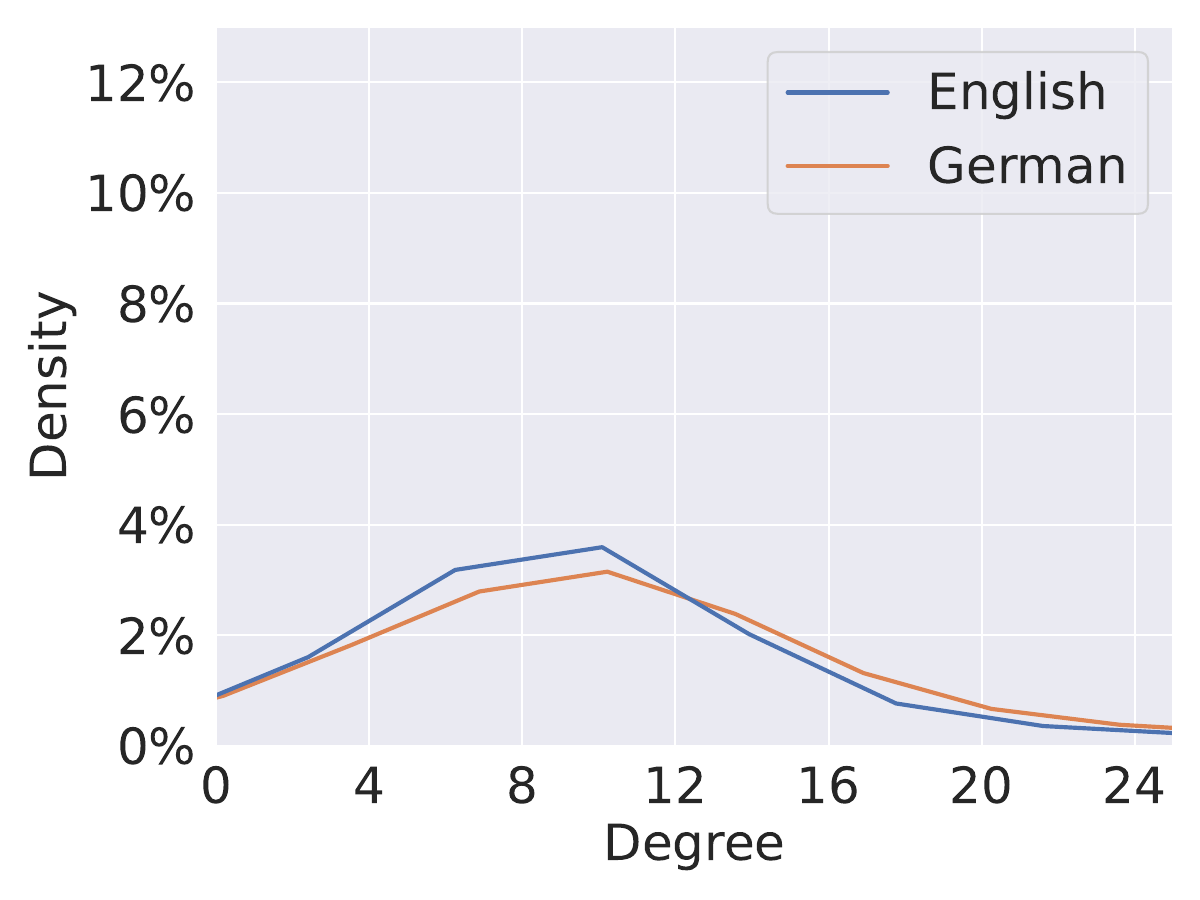}
\subcaption{EN$\longleftrightarrow$DE}
\end{minipage}
\caption{{\bf Statistics of \ourdata:} We report graph statistics including the number of nodes, number of relations, observed (obv.) triplets, querying (qry.) triplets, and average degree for each graph pair, e.g., (a) corresponds to DBPedia-and-Wikidata pair, and will be used to construct DB2WD and WD2DB tasks. We also report (in \& out) degree distribution on each graph at the bottom. We omit tail distribution larger than 25 since they are too small and almost flat.}
\label{fig:stats-pediatype}
\end{figure}

\begin{algorithm}
\caption{{\bf Sampling Algorithm for \ourdata.} This is a subgraph sampling code for a single graph (either training or test). It will reduce the large original graph into a connected graph of the required size.}
\label{alg:sample-deg}
\begin{algorithmic}[1]
\Require Raw graph triplets $\cS^\text{raw}$, Raw graph node set $\cV^\text{raw}$, Raw graph relation set $\cR^\text{raw}$, Maximum number of nodes $N$, Maximum number of edges $M$, Maximum node degree $D$.
\Ensure Subgraph triplets $\cS^\text{sub}$
\State $\cS^\text{sub} \leftarrow \emptyset$
\State $\cV^\text{sub} \leftarrow \emptyset$
\State $\cR^\text{sub} \leftarrow \emptyset$
\State Create an empty queue $Q$.
\State Get the node $v_0$ with the highest degree in the raw graph.
\State $Q\text{.add}(v_0)$
\State $\cV^\text{sub} \leftarrow \cV^\text{sub} \cup \{ v_0 \}$
\While{$|Q| > 0$}
    \State $u \leftarrow Q\text{.pop}()$
    \If{$|\cV^\text{sub}| \geq N$ or $|\cV^\text{sub}| \geq M$}
        \State \textbf{continue}
    \EndIf
    \State $\cB = \{ (v, r, u) | (r, v) \in \cR^\text{raw} \times \cV^\text{raw} \} \cup \{ (u, r, v) | (r, v) \in \cR^\text{raw} \times \cV^\text{raw} \}$
    \If{$|\cB| > D$}
        \State Uniformly select $D$ triplets from $\cB$ as $\cB'$
    \Else
        \State $\cB' \leftarrow \cB$
    \EndIf
    \For{$(i, r, j) \in \cB'$}
        \If{$i = u$}
            \State $Q\text{.add}(j)$
            \State $\cV^\text{sub} \leftarrow \cV^\text{sub} \cup \{ j \}$
        \Else
            \State $Q\text{.add}(i)$
            \State $\cV^\text{sub} \leftarrow \cV^\text{sub} \cup \{ i \}$
        \EndIf
        \State $\cS^\text{sub} \leftarrow \cS^\text{sub} \cup \{ (i, r, j) \}$
    \EndFor
\EndWhile
\end{algorithmic}
\end{algorithm}

\vspace{-5pt}
\paragraph{Additional Results} We present the Node \& Relation Hits@10 performance in the main paper. We provide more results including MRR, Hits@1, Hits@5 in \Cref{tab:pediatypes-mrr,tab:pediatypes-hit1,tab:pediatypes-hit5}. We can see that our proposed \update{\OurNewModel} and \OurOtherModel perform consistently and significantly 
better than the baselines in the much harder relation prediction task, showing their power to generalize to both new nodes and new relations. The structural double equivariant model \update{\OurNewModel} performs worse on node prediction over some datasets, which might be due to the node GNN implementation of \update{\OurNewModel}. These tasks do not care much about the actual relation type as we can see from the superior performance of homogeneous GNNs on node prediction. So the additional equivariance over relations and the training loss over both negative nodes and negative relations might cause the model to focus more on the relation prediction task, while the double equivariant structural representation might hurt the performance of missing node prediction~\citep{srinivasan2020on}. %We suppose the reason for those poor cases is that exchangeable representation of \OurModel ranks a lot negative triplets with similar scores as positive since knowledge learned from training can not distinguish them due to difference between logic behind them. This behavior may share similar reason as the expressivity limitation shown in \Cref{subsubsec:limit}.

But it is important to note that the structural double equivariant \update{\OurNewModel} model excels on relation prediction and achieves much better results on Hits@1 and Hits@5 as shown in \Cref{tab:pediatypes-hit1,tab:pediatypes-hit5}. The performance of baseline models that is lower than random is probably because the knowledge they learn from one dataset is not able to correctly transform to another dataset, while our double equivariant model architecture is able to perform this hard \ourtask over both new nodes and new relation types. We also note that in the Hits@1 and Hits@5~\Cref{tab:pediatypes-hit1,tab:pediatypes-hit5}, there are cases where \OurOtherModel has higher variances than the original InGram while achieving much better average performance. This is because due to the random initialization, InGram performs poorly on the much harder Hits@1 and Hits@5 performance compared to Hits@10. In some seeds of the runs, \OurOtherModel successfully improves the performance of InGram, but there are still seeds of runs that \OurOtherModel still performs similar to InGram. Thus, it results in \OurOtherModel having much better average results while also with higher standard deviations.

\begin{table}[t]
%\vspace{-25pt}   % Reduce table head space to the top of the page
\centering
\captionof{table}{
{\bf Relation \& Node MRR performance on \OurTask over \ourdata.} We report standard deviations over 5 runs. %
A higher value means better \ourtask performance. 
``Rand'' column contains unbiased estimations of the performance from a random predictor.
% Our models achieves constantly better results than other unattributed link prediction baselines.
{\bf Both \update{\OurNewModel} and \OurOtherModel consistently achieve better results than the baselines.}
%while the standard deviations of \OurModel $<$ \OurOtherModel $<$ baseline InGram in most cases.}
N/A*: Not available due to constant crashes.
}
{
\subcaption{{\bf {\scriptsize Relation prediction $(i, ?, j)$ performance in \%. Higher $\uparrow$ is better.}}}
\resizebox{\linewidth}{!}{
\begin{tabular}{l r r r r r r r r}
    Models & EN-FR & FR-EN & EN-DE & DE-EN & DB-WD & WD-DB & DB-YG & YG-DB \\
    \midrule
    
    Rand & 8.86{\scriptsize $\pm 00.00$} & 8.86{\scriptsize $\pm 00.00$} & 8.86{\scriptsize $\pm 00.00$} & 8.86{\scriptsize $\pm 00.00$} & 8.86{\scriptsize $\pm 00.00$} & 8.86{\scriptsize $\pm 00.00$} & 8.86{\scriptsize $\pm 00.00$} & 8.86{\scriptsize $\pm 00.00$}\\
    \midrule
    
    GAT & 8.04{\scriptsize $\pm 00.25$} & 7.93{\scriptsize $\pm 00.04$} & 8.17{\scriptsize $\pm 00.08$} & 8.12{\scriptsize $\pm 00.09$} & 8.06{\scriptsize $\pm 00.15$} & 7.90{\scriptsize $\pm 00.12$} & 8.12{\scriptsize $\pm 00.21$} & 8.17{\scriptsize $\pm 00.16$} \\
    \text{{GIN}} & 8.07{{\scriptsize $\pm 00.09$}} & 8.09{{\scriptsize $\pm 00.05$}} & 8.07{{\scriptsize $\pm 00.13$}} & 8.07{{\scriptsize $\pm 00.11$}} & 8.03{{\scriptsize $\pm 00.20$}} & 7.97{{\scriptsize $\pm 00.30$}} & 7.82{{\scriptsize $\pm 00.27$}} & 7.84{{\scriptsize $\pm 00.14$}} \\
    GraphConv & 7.92{\scriptsize $\pm 00.16$} & 7.97{\scriptsize $\pm 00.12$} & 8.07{\scriptsize $\pm 00.15$} & 8.03{\scriptsize $\pm 00.05$} & 8.14{\scriptsize $\pm 00.04$} & 7.98{\scriptsize $\pm 00.18$} & 8.04{\scriptsize $\pm 00.24$} & 7.84{\scriptsize $\pm 00.13$} \\
    NBFNet &  10.25{\scriptsize $\pm 01.24$} & 9.53{\scriptsize $\pm 00.85$} & 8.15{\scriptsize $\pm 01.21$} & 4.32{\scriptsize $\pm 00.26$} & 10.33{\scriptsize $\pm 02.45$} & 8.97{\scriptsize $\pm 01.24$} & 9.29{\scriptsize $\pm 01.38$} & 14.54{\scriptsize $\pm 04.76$} \\
    RMPI & 12.45{\scriptsize $\pm 01.90$} & 12.10{\scriptsize $\pm 02.71$} & 11.69{\scriptsize $\pm 04.37$} & 10.28{\scriptsize $\pm 01.28$} & N/A* & 8.54{\scriptsize $\pm 02.70$} & 17.89{\scriptsize $\pm 12.22$} & 6.53{\scriptsize $\pm 02.16$} \\
    InGram & 50.03{\scriptsize $\pm 05.32$} & 26.31{\scriptsize $\pm 08.27$} & 21.32{\scriptsize $\pm 07.84$} & 29.81{\scriptsize $\pm 14.21$} & 48.70{\scriptsize $\pm 10.06$} & 38.81{\scriptsize $\pm 03.10$} & 29.94{\scriptsize $\pm 13.28$} & 32.26{\scriptsize $\pm 13.97$} \\
    \midrule
    
    \OurOtherModel (Ours) & \textbf{73.38}{\scriptsize $\pm 05.77$} & \underline{41.61}{\scriptsize $\pm 10.12$} & \underline{46.86}{\scriptsize $\pm 09.11$} & \underline{40.56}{\scriptsize $\pm 14.80$} & \textbf{80.74}{\scriptsize $\pm 04.47$} & \underline{66.06}{\scriptsize $\pm 02.91$} & \underline{39.51}{\scriptsize $\pm 16.76$} & \underline{49.10}{\scriptsize $\pm 05.43$} \\
    
    % \OurModel (Ours) & \underline{70.06}{\scriptsize $\pm 02.01$} & \textbf{69.01}{\scriptsize $\pm 00.57$} & \textbf{78.38}{\scriptsize $\pm 04.04$} & \textbf{88.82}{\scriptsize $\pm 00.28$} & \underline{65.89}{\scriptsize $\pm 04.71$} & \textbf{72.57}{\scriptsize $\pm 00.73$} & \textbf{75.88}{\scriptsize $\pm 01.58$} & \textbf{74.04}{\scriptsize $\pm 00.47$} \\
    \update{\update{\OurNewModel} (Ours)} & \update{\underline{72.96}{\scriptsize $\pm 00.77$}} & \update{\textbf{65.73}{\scriptsize $\pm 00.58$}} & \update{\textbf{59.95}{\scriptsize $\pm 03.91$}} & \update{\textbf{84.71}{\scriptsize $\pm 01.11$}} & \update{\underline{71.47}{\scriptsize $\pm 00.31$}} & \update{\textbf{71.47}{\scriptsize $\pm 00.69$}} & \update{\textbf{66.48}{\scriptsize $\pm 06.75$}} & \update{\textbf{67.36}{\scriptsize $\pm 00.43$}}
\end{tabular}
\label{tab:pediatypes-relation-mrr}
}
\vspace{5pt} % Make sure subtitle of next table does not come too close to bottom of last table
{
\subcaption{{\bf {\scriptsize Node prediction $(i, k, ?)$ performance in \%. Higher $\uparrow$ is better.}}}
\resizebox{\linewidth}{!}{
\begin{tabular}{l r r r r r r r r}
    Models & EN-FR & FR-EN & EN-DE & DE-EN & DB-WD & WD-DB & DB-YG & YG-DB \\
    \midrule
    
    Rand & 8.86{\scriptsize $\pm 00.00$} & 8.86{\scriptsize $\pm 00.00$} & 8.86{\scriptsize $\pm 00.00$} & 8.86{\scriptsize $\pm 00.00$} & 8.86{\scriptsize $\pm 00.00$} & 8.86{\scriptsize $\pm 00.00$} & 8.86{\scriptsize $\pm 00.00$} & 8.86{\scriptsize $\pm 00.00$}\\
    \midrule
    
    GAT & 51.43{\scriptsize $\pm 00.25$} & 49.48{\scriptsize $\pm 01.51$} & 26.22{\scriptsize $\pm 00.44$} & 25.45{\scriptsize $\pm 01.23$} & 16.87{\scriptsize $\pm 00.59$} & 34.66{\scriptsize $\pm 00.33$} & 37.22{\scriptsize $\pm 00.29$} & 45.96{\scriptsize $\pm 00.29$} \\
    GIN & 53.72{\scriptsize $\pm 03.45$} & 52.03{\scriptsize $\pm 03.38$} & 34.60{\scriptsize $\pm 07.43$} & 37.27{\scriptsize $\pm 09.42$} & 20.75{\scriptsize $\pm 07.22$} & 40.37{\scriptsize $\pm 08.20$} & 35.80{\scriptsize $\pm 01.36$} & 44.77{\scriptsize $\pm 00.92$} \\
    GraphConv & 63.72{\scriptsize $\pm 01.76$} & 57.77{\scriptsize $\pm 01.09$} & 48.18{\scriptsize $\pm 00.96$} & 45.18{\scriptsize $\pm 00.15$} & 22.49{\scriptsize $\pm 00.76$} & 50.30{\scriptsize $\pm 02.80$} & 38.71{\scriptsize $\pm 00.55$} & 50.54{\scriptsize $\pm 00.42$} \\
    NBFNet & 69.22{\scriptsize $\pm 02.44$} & \textbf{74.01}{\scriptsize $\pm 01.41$} & {63.49}{\scriptsize $\pm 02.44$} & 38.86{\scriptsize $\pm 02.55$} & 41.26{\scriptsize $\pm 02.58$} & {64.02}{\scriptsize $\pm 01.25$} & 38.13{\scriptsize $\pm 01.11$} & 52.30{\scriptsize $\pm 02.09$}  \\
    RMPI & 63.02{\scriptsize $\pm 02.94$} & 43.72{\scriptsize $\pm 05.65$} & 44.82{\scriptsize $\pm 02.93$} & 46.84{\scriptsize $\pm 05.36$} & N/A* & 46.33{\scriptsize $\pm 08.76$} & \textbf{43.00}{\scriptsize $\pm 03.70$} & \underline{53.72}{\scriptsize $\pm 01.84$}  \\
    InGram & 71.23{\scriptsize $\pm 01.73$} & 55.67{\scriptsize $\pm 05.65$} & 55.94{\scriptsize $\pm 02.76$} & {61.15}{\scriptsize $\pm 01.42$} & 34.50{\scriptsize $\pm 08.47$} & 57.05{\scriptsize $\pm 03.73$} & 26.36{\scriptsize $\pm 04.73$} & \textbf{56.23}{\scriptsize $\pm 01.56$} \\
    \midrule
    
    \OurOtherModel (Ours) & \textbf{78.45}{\scriptsize $\pm 00.89$} & \underline{68.59}{\scriptsize $\pm 04.30$} & \underline{66.13}{\scriptsize $\pm 01.48$} & \textbf{70.32}{\scriptsize $\pm 01.58$} & \underline{44.71}{\scriptsize $\pm 08.98$} & \underline{69.23}{\scriptsize $\pm 02.53$} & 35.67{\scriptsize $\pm 03.92$} & 48.07{\scriptsize $\pm 08.76$} \\
    
    % \OurModel (Ours) & 53.92{\scriptsize $\pm 00.26$} & 57.68{\scriptsize $\pm 00.68$} & 50.30{\scriptsize $\pm 02.08$} & 51.33{\scriptsize $\pm 00.40$} & \textbf{45.75}{\scriptsize $\pm 00.66$} & 51.64{\scriptsize $\pm 00.60$}& \underline{41.72}{\scriptsize $\pm 01.64$} & {48.21}{\scriptsize $\pm 01.06$} \\

    \update{\update{\OurNewModel} (Ours)} & \update{\underline{74.95}{\scriptsize $\pm 01.56$}} & \update{57.17{\scriptsize $\pm 01.70$}} & \update{\textbf{74.38}{\scriptsize $\pm 00.66$}} & \update{\underline{62.62}{\scriptsize $\pm 00.22$}} & \update{\textbf{63.21}{\scriptsize $\pm 00.69$}} & \update{\textbf{70.58}{\scriptsize $\pm 00.42$}} & \update{34.79{\scriptsize $\pm 00.49$}} & \update{40.71{\scriptsize $\pm 01.75$}}
\end{tabular}
\label{tab:pediatypes-node-mrr}
}
}
%\vspace{-15pt}  % Reduce table bottom space to the text
}
\label{tab:pediatypes-mrr}
\end{table}

\begin{table}[t]
%\vspace{-25pt}   % Reduce table head space to the top of the page
\centering
\captionof{table}{
{\bf Relation \& Node Hits@1 performance on \OurTask over \ourdata.} We report standard deviations over 5 runs. %
A higher value means better \ourtask performance. 
``Rand'' column contains unbiased estimations of the performance from a random predictor.
% Our models achieves constantly better results than other unattributed link prediction baselines.
{\bf Both \update{\OurNewModel} and \OurOtherModel consistently achieve better results than the baselines.}
%while the standard deviations of \OurModel $<$ \OurOtherModel $<$ baseline InGram in most cases.}
N/A*: Not available due to constant crashes.
}
{
\subcaption{{\bf {\scriptsize Relation prediction $(i, ?, j)$ performance in \%. Higher $\uparrow$ is better.}}}
\resizebox{\linewidth}{!}{
\begin{tabular}{l r r r r r r r r}
    Models & EN-FR & FR-EN & EN-DE & DE-EN & DB-WD & WD-DB & DB-YG & YG-DB \\
    \midrule
    
    Rand & 1.96{\scriptsize $\pm 00.00$} & 1.96{\scriptsize $\pm 00.00$} & 1.96{\scriptsize $\pm 00.00$} & 1.96{\scriptsize $\pm 00.00$} & 1.96{\scriptsize $\pm 00.00$} & 1.96{\scriptsize $\pm 00.00$} & 1.96{\scriptsize $\pm 00.00$} & 1.96{\scriptsize $\pm 00.00$}\\
    \midrule
    
    GAT & 1.07{\scriptsize $\pm 00.14$} & 1.01{\scriptsize $\pm 00.01$} & 1.03{\scriptsize $\pm 00.03$} & 1.11{\scriptsize $\pm 00.09$} & 1.07{\scriptsize $\pm 00.14$} & 0.99{\scriptsize $\pm 00.21$} & 0.96{\scriptsize $\pm 00.16$} & 1.09{\scriptsize $\pm 00.25$} \\
    GIN & 1.01{\scriptsize $\pm 00.03$} & 0.95{\scriptsize $\pm 00.08$} & 1.03{\scriptsize $\pm 00.06$} & 1.10{\scriptsize $\pm 00.06$} & 0.96{\scriptsize $\pm 00.15$} & 1.00{\scriptsize $\pm 00.15$} & 0.92{\scriptsize $\pm 00.15$} & 0.83{\scriptsize $\pm 00.17$} \\
    GraphConv & 0.91{\scriptsize $\pm 00.03$} & 0.97{\scriptsize $\pm 00.06$} & 1.05{\scriptsize $\pm 00.14$} & 1.01{\scriptsize $\pm 00.03$} & 1.09{\scriptsize $\pm 00.07$} & 0.91{\scriptsize $\pm 00.04$} & 0.94{\scriptsize $\pm 00.22$} & 0.88{\scriptsize $\pm 00.20$} \\
    NBFNet & 4.43{\scriptsize $\pm 01.24$} & 3.62{\scriptsize $\pm 01.01$} & 2.49{\scriptsize $\pm 01.23$} & 0.51{\scriptsize $\pm 00.18$} & 4.18{\scriptsize $\pm 02.17$} & 2.80{\scriptsize $\pm 00.83$} & 1.63{\scriptsize $\pm 00.89$} & 7.30{\scriptsize $\pm 05.01$} \\
    RMPI & 3.92{\scriptsize $\pm 02.08$} & 4.04{\scriptsize $\pm 01.83$} & 3.37{\scriptsize $\pm 02.20$} & 2.13{\scriptsize $\pm 00.79$} & N/A* & 2.39{\scriptsize $\pm 02.35$} & 7.36{\scriptsize $\pm 09.03$} & 0.91{\scriptsize $\pm 00.92$} \\
    InGram & 35.19{\scriptsize $\pm 07.73$} & 12.40{\scriptsize $\pm 07.55$} & 8.45{\scriptsize $\pm 06.57$} & 16.46{\scriptsize $\pm 16.33$} & 33.66{\scriptsize $\pm 12.09$} & 25.69{\scriptsize $\pm 03.88$} & 14.24{\scriptsize $\pm 12.00$} & 15.83{\scriptsize $\pm 12.59$} \\
    \midrule
    
    \OurOtherModel (Ours) & \textbf{65.26}{\scriptsize $\pm 10.23$} & \underline{26.90}{\scriptsize $\pm 12.97$} & \underline{36.80}{\scriptsize $\pm 11.16$} & \underline{25.34}{\scriptsize $\pm 18.48$} & \textbf{75.00}{\scriptsize $\pm 06.42$} & \textbf{60.35}{\scriptsize $\pm 02.56$} & \underline{24.28}{\scriptsize $\pm 14.29$} & \underline{30.82}{\scriptsize $\pm 10.43$} \\
    
    % \OurModel (Ours) & \underline{61.46}{\scriptsize $\pm 00.79$} & \textbf{58.18}{\scriptsize $\pm 00.14$} & \textbf{68.00}{\scriptsize $\pm 06.41$} & \textbf{84.83}{\scriptsize $\pm 00.29$} & \underline{57.51}{\scriptsize $\pm 05.40$} & \textbf{62.72}{\scriptsize $\pm 01.24$} & \textbf{69.12}{\scriptsize $\pm 02.40$} & \textbf{66.68}{\scriptsize $\pm 00.81$} \\

    \update{\update{\OurNewModel} (Ours)} & \update{\underline{58.43}{\scriptsize $\pm 01.29$}} & \update{\textbf{48.68}{\scriptsize $\pm 00.96$}} & \update{\textbf{37.29}{\scriptsize $\pm 05.11$}} & \update{\textbf{75.08}{\scriptsize $\pm 01.99$}} & \update{\underline{57.05}{\scriptsize $\pm 00.92$}} & \update{\underline{56.00}{\scriptsize $\pm 01.17$}} & \update{\textbf{59.36}{\scriptsize $\pm 07.96$}} & \update{\textbf{49.41}{\scriptsize $\pm 00.85$}}
\end{tabular}
\label{tab:pediatypes-relation-hit1}
}
\vspace{5pt} % Make sure subtitle of next table does not come too close to bottom of last table
{
\subcaption{{\bf {\scriptsize Node prediction $(i, k, ?)$ performance in \%. Higher $\uparrow$ is better.}}}
\resizebox{\linewidth}{!}{
\begin{tabular}{l r r r r r r r r}
    Models & EN-FR & FR-EN & EN-DE & DE-EN & DB-WD & WD-DB & DB-YG & YG-DB \\
    \midrule
    
   Rand & 1.96{\scriptsize $\pm 00.00$} & 1.96{\scriptsize $\pm 00.00$} & 1.96{\scriptsize $\pm 00.00$} & 1.96{\scriptsize $\pm 00.00$} & 1.96{\scriptsize $\pm 00.00$} & 1.96{\scriptsize $\pm 00.00$} & 1.96{\scriptsize $\pm 00.00$} & 1.96{\scriptsize $\pm 00.00$}\\
    \midrule
    
    GAT & 31.80{\scriptsize $\pm 00.64$} & 30.19{\scriptsize $\pm 02.30$} & 10.23{\scriptsize $\pm 00.96$} & 8.68{\scriptsize $\pm 01.69$} & 7.98{\scriptsize $\pm 00.89$} & 16.26{\scriptsize $\pm 00.34$} & 26.09{\scriptsize $\pm 00.47$} & 33.06{\scriptsize $\pm 00.29$} \\
    GIN & 34.59{\scriptsize $\pm 04.64$} & 34.57{\scriptsize $\pm 05.26$} & 17.69{\scriptsize $\pm 07.91$} & 20.74{\scriptsize $\pm 10.01$} & 12.42{\scriptsize $\pm 06.59$} & 23.10{\scriptsize $\pm 09.67$} & 23.72{\scriptsize $\pm 01.62$} & 32.26{\scriptsize $\pm 01.89$} \\
    GraphConv & 47.48{\scriptsize $\pm 02.60$} & 40.37{\scriptsize $\pm 01.52$} & 31.96{\scriptsize $\pm 01.02$} & 28.46{\scriptsize $\pm 00.13$} & 12.53{\scriptsize $\pm 00.34$} & 35.82{\scriptsize $\pm 03.54$} & 24.12{\scriptsize $\pm 00.80$} & 37.05{\scriptsize $\pm 00.51$} \\
    NBFNet & \underline{64.17}{\scriptsize $\pm 02.68$} & \textbf{69.68}{\scriptsize $\pm 01.63$} & \underline{57.50}{\scriptsize $\pm 02.66$} & 32.26{\scriptsize $\pm 02.81$} & \underline{34.56}{\scriptsize $\pm 02.54$} & \underline{59.70}{\scriptsize $\pm 01.38$} & \textbf{33.32}{\scriptsize $\pm 01.11$} & \textbf{47.47}{\scriptsize $\pm 02.08$} \\
    RMPI & 48.27{\scriptsize $\pm 03.74$} & 26.92{\scriptsize $\pm 04.87$} & 27.38{\scriptsize $\pm 03.09$} & 29.60{\scriptsize $\pm 04.77$} & N/A* & 34.81{\scriptsize $\pm 08.97$} & \underline{33.29}{\scriptsize $\pm 03.20$} & \underline{42.14}{\scriptsize $\pm 02.87$} \\
    InGram & 60.00{\scriptsize $\pm 02.06$} & 41.59{\scriptsize $\pm 06.37$} & 39.05{\scriptsize $\pm 02.99$} & \underline{45.44}{\scriptsize $\pm 01.69$} & 22.06{\scriptsize $\pm 08.10$} & 42.54{\scriptsize $\pm 04.50$} & 13.47{\scriptsize $\pm 03.50$} & 20.09{\scriptsize $\pm 04.96$} \\
    \midrule
    
    \OurOtherModel (Ours) & \textbf{69.46}{\scriptsize $\pm 01.12$} & \underline{57.65}{\scriptsize $\pm 05.54$} & {51.93}{\scriptsize $\pm 01.88$} & \textbf{57.06}{\scriptsize $\pm 01.96$} & 32.12{\scriptsize $\pm 09.51$} & {57.84}{\scriptsize $\pm 03.28$} & 20.49{\scriptsize $\pm 03.35$} & 33.01{\scriptsize $\pm 08.87$} \\
    
    % \OurModel (Ours) & 43.03{\scriptsize $\pm 00.25$} & 47.38{\scriptsize $\pm 00.28$} & 35.41{\scriptsize $\pm 02.25$} & 37.12{\scriptsize $\pm 00.31$} & \textbf{35.59}{\scriptsize $\pm 00.73$} & 40.56{\scriptsize $\pm 01.72$} & 27.70{\scriptsize $\pm 01.95$} & 35.29{\scriptsize $\pm 01.67$} \\

    \update{\update{\OurNewModel} (Ours)} & \update{62.17{\scriptsize $\pm 02.38$}} & \update{44.67{\scriptsize $\pm 01.92$}} & \update{\textbf{63.36}{\scriptsize $\pm 00.78$}} & \update{\underline{47.78}{\scriptsize $\pm 00.48$}} & \update{\textbf{51.76}{\scriptsize $\pm 00.86$}} & \update{\textbf{60.15}{\scriptsize $\pm 00.69$}} & \update{20.74{\scriptsize $\pm 00.28$}} & \update{26.24{\scriptsize $\pm 02.03$}}
\end{tabular}
\label{tab:pediatypes-node-hit1}
}
}
%\vspace{-15pt}  % Reduce table bottom space to the text
}
\label{tab:pediatypes-hit1}
\end{table}

\begin{table}[t]
%\vspace{-25pt}   % Reduce table head space to the top of the page
\centering
\captionof{table}{
{\bf Relation \& Node Hits@5 performance on \OurTask over \ourdata.} We report standard deviations over 5 runs. %
A higher value means better \ourtask performance. 
``Rand'' column contains unbiased estimations of the performance from a random predictor.
% Our models achieves constantly better results than other unattributed link prediction baselines.
{\bf Both \update{\OurNewModel} and \OurOtherModel consistently achieve better results than the baselines.}
%while the standard deviations of \OurModel $<$ \OurOtherModel $<$ baseline InGram in most cases.}
N/A*: Not available due to constant crashes.
}
{
\subcaption{{\bf {\scriptsize Relation prediction $(i, ?, j)$ performance in \%. Higher $\uparrow$ is better.}}}
\resizebox{\linewidth}{!}{
\begin{tabular}{l r r r r r r r r}
    Models & EN-FR & FR-EN & EN-DE & DE-EN & DB-WD & WD-DB & DB-YG & YG-DB \\
    \midrule
    
    Rand & 9.80{\scriptsize $\pm 00.00$} & 9.80{\scriptsize $\pm 00.00$} & 9.80{\scriptsize $\pm 00.00$} & 9.80{\scriptsize $\pm 00.00$} & 9.80{\scriptsize $\pm 00.00$} & 9.80{\scriptsize $\pm 00.00$} & 9.80{\scriptsize $\pm 00.00$} & 9.80{\scriptsize $\pm 00.00$}\\
    \midrule
    
    GAT & 9.08{\scriptsize $\pm 00.39$} & 8.63{\scriptsize $\pm 00.25$} & 9.47{\scriptsize $\pm 00.18$} & 9.20{\scriptsize $\pm 00.24$} & 8.95{\scriptsize $\pm 00.36$} & 8.63{\scriptsize $\pm 00.29$} & 9.58{\scriptsize $\pm 00.50$} & 9.16{\scriptsize $\pm 00.23$} \\
    GIN & 9.09{\scriptsize $\pm 00.16$} & 9.31{\scriptsize $\pm 00.15$} & 9.18{\scriptsize $\pm 00.28$} & 9.23{\scriptsize $\pm 00.34$} & 9.12{\scriptsize $\pm 00.12$} & 8.85{\scriptsize $\pm 00.56$} & 8.53{\scriptsize $\pm 00.66$} & 8.61{\scriptsize $\pm 00.34$} \\
    GraphConv & 8.97{\scriptsize $\pm 00.66$} & 8.74{\scriptsize $\pm 00.26$} & 9.23{\scriptsize $\pm 00.11$} & 8.82{\scriptsize $\pm 00.10$} & 9.17{\scriptsize $\pm 00.29$} & 9.11{\scriptsize $\pm 00.50$} & 9.01{\scriptsize $\pm 00.72$} & 8.73{\scriptsize $\pm 00.15$} \\
    NBFNet &  12.94{\scriptsize $\pm 01.77$} & 12.46{\scriptsize $\pm 01.40$} & 8.56{\scriptsize $\pm 01.67$} & 2.68{\scriptsize $\pm 00.72$} & 13.44{\scriptsize $\pm 04.02$} & 11.74{\scriptsize $\pm 03.02$} & 11.95{\scriptsize $\pm 03.78$} & 20.37{\scriptsize $\pm 05.90$} \\
    RMPI & 16.39{\scriptsize $\pm 04.15$} & 15.76{\scriptsize $\pm 04.58$} & 15.86{\scriptsize $\pm 08.05$} & 12.56{\scriptsize $\pm 02.70$} & N/A* & 8.91{\scriptsize $\pm 03.51$}  & 24.25{\scriptsize $\pm 19.24$} & 4.98{\scriptsize $\pm 03.08$} \\
    InGram & 67.15{\scriptsize $\pm 05.04$} & 37.86{\scriptsize $\pm 14.41$} & 30.99{\scriptsize $\pm 11.82$} & 40.00{\scriptsize $\pm 13.02$} & 65.80{\scriptsize $\pm 09.59$} & 51.66{\scriptsize $\pm 03.57$} & 43.27{\scriptsize $\pm 19.30$} & 51.54{\scriptsize $\pm 26.09$}  \\
    \midrule
    
    \OurOtherModel (Ours) & \underline{83.23}{\scriptsize $\pm 05.64$} & \underline{59.83}{\scriptsize $\pm 11.57$} & \underline{54.30}{\scriptsize $\pm 08.25$} & \underline{57.65}{\scriptsize $\pm 15.74$} & \underline{87.08}{\scriptsize $\pm 02.55$} & \underline{70.79}{\scriptsize $\pm 03.80$} & \underline{51.45}{\scriptsize $\pm 29.14$} & \underline{75.85}{\scriptsize $\pm 07.26$} \\
    
    % \OurModel (Ours) & \underline{82.11}{\scriptsize $\pm 04.01$} & \textbf{83.19}{\scriptsize $\pm 01.73$} & \textbf{92.39}{\scriptsize $\pm 00.83$} & \textbf{93.59}{\scriptsize $\pm 00.53$} & \underline{75.95}{\scriptsize $\pm 03.89$} & \textbf{86.10}{\scriptsize $\pm 01.26$} & \textbf{85.80}{\scriptsize $\pm 01.23$} & \textbf{83.36}{\scriptsize $\pm 01.55$} \\

    \update{\update{\OurNewModel} (Ours)} & \update{\textbf{93.79}{\scriptsize $\pm 00.20$}} & \update{\textbf{91.21}{\scriptsize $\pm 00.25$}} & \update{\textbf{94.04}{\scriptsize $\pm 01.21$}} & \update{\textbf{96.64}{\scriptsize $\pm 00.13$}} & \update{\textbf{90.83}{\scriptsize $\pm 02.29$}} & \update{\textbf{93.97}{\scriptsize $\pm 00.45$}} & \update{\textbf{74.27}{\scriptsize $\pm 06.29$}} & \update{\textbf{92.75}{\scriptsize $\pm 00.40$}}
\end{tabular}
\label{tab:pediatypes-relation-hit5}
}
\vspace{5pt} % Make sure subtitle of next table does not come too close to bottom of last table
{
\subcaption{{\bf {\scriptsize Node prediction $(i, k, ?)$ performance in \%. Higher $\uparrow$ is better.}}}
\resizebox{\linewidth}{!}{
\begin{tabular}{l r r r r r r r r}
    Models & EN-FR & FR-EN & EN-DE & DE-EN & DB-WD & WD-DB & DB-YG & YG-DB \\
    \midrule
    
    Rand & 9.80{\scriptsize $\pm 00.00$} & 9.80{\scriptsize $\pm 00.00$} & 9.80{\scriptsize $\pm 00.00$} & 9.80{\scriptsize $\pm 00.00$} & 9.80{\scriptsize $\pm 00.00$} & 9.80{\scriptsize $\pm 00.00$} & 9.80{\scriptsize $\pm 00.00$} & 9.80{\scriptsize $\pm 00.00$}\\
    \midrule
    
    GAT & 78.49{\scriptsize $\pm 00.44$} & 74.70{\scriptsize $\pm 00.68$} & 42.17{\scriptsize $\pm 00.91$} & 42.39{\scriptsize $\pm 00.52$} & 20.96{\scriptsize $\pm 00.65$} & 57.26{\scriptsize $\pm 00.89$} & 46.92{\scriptsize $\pm 00.37$} & 59.20{\scriptsize $\pm 00.41$} \\
    GIN & 79.96{\scriptsize $\pm 01.88$} & 74.33{\scriptsize $\pm 01.16$} & 53.97{\scriptsize $\pm 07.61$} & 55.89{\scriptsize $\pm 10.06$} & 25.05{\scriptsize $\pm 09.23$} & 61.94{\scriptsize $\pm 06.71$} & 46.56{\scriptsize $\pm 01.37$} & 57.48{\scriptsize $\pm 00.35$} \\
    GraphConv & 85.21{\scriptsize $\pm 00.63$} & 80.67{\scriptsize $\pm 00.30$} & 67.76{\scriptsize $\pm 01.19$} & 64.97{\scriptsize $\pm 00.43$} & 28.37{\scriptsize $\pm 01.41$} & 67.36{\scriptsize $\pm 02.37$} & \underline{53.79}{\scriptsize $\pm 00.72$} & 64.13{\scriptsize $\pm 00.23$} \\
    NBFNet & 81.48{\scriptsize $\pm 02.24$} & \textbf{85.15}{\scriptsize $\pm 01.06$} & 77.62{\scriptsize $\pm 02.41$} & 48.73{\scriptsize $\pm 02.59$} & 51.52{\scriptsize $\pm 03.21$} & {72.18}{\scriptsize $\pm 00.90$} & 44.01{\scriptsize $\pm 01.40$} & 60.34{\scriptsize $\pm 02.28$}  \\
    RMPI & 82.47{\scriptsize $\pm 02.25$} & 64.88{\scriptsize $\pm 07.62$} & 67.24{\scriptsize $\pm 04.38$} & 69.47{\scriptsize $\pm 06.60$} & N/A* & 60.11{\scriptsize $\pm 08.77$}  & 51.57{\scriptsize $\pm 05.03$} & \textbf{66.67}{\scriptsize $\pm 01.28$} \\
    InGram & {85.15}{\scriptsize $\pm 01.74$} & 72.32{\scriptsize $\pm 05.31$} & {78.84}{\scriptsize $\pm 02.86$} & {81.01}{\scriptsize $\pm 00.97$} & 45.96{\scriptsize $\pm 11.09$} & 74.88{\scriptsize $\pm 03.09$} & 37.49{\scriptsize $\pm 06.84$} & 50.66{\scriptsize $\pm 06.76$} \\
    \midrule
    
    \OurOtherModel (Ours) & \underline{89.62}{\scriptsize $\pm 00.63$} & \underline{81.54}{\scriptsize $\pm 02.82$} & \underline{84.57}{\scriptsize $\pm 00.95$} & \textbf{87.16}{\scriptsize $\pm 01.04$} & \underline{57.44}{\scriptsize $\pm 09.14$} & \underline{83.14}{\scriptsize $\pm 01.64$} & 51.77{\scriptsize $\pm 05.14$} & \underline{65.33}{\scriptsize $\pm 09.57$} \\
    
    % \OurModel (Ours) & 64.45{\scriptsize $\pm 00.24$} & 67.24{\scriptsize $\pm 01.32$} & 68.80{\scriptsize $\pm 01.90$} & 68.20{\scriptsize $\pm 00.53$} & \underline{54.83}{\scriptsize $\pm 00.90$} & 62.60{\scriptsize $\pm 02.55$} & \textbf{55.21}{\scriptsize $\pm 01.07$} & 61.87{\scriptsize $\pm 01.30$}  \\

    \update{\update{\OurNewModel} (Ours)} & \update{\textbf{92.45}{\scriptsize $\pm 00.73$}} & \update{71.24{\scriptsize $\pm 02.13$}} & \update{\textbf{89.98}{\scriptsize $\pm 00.96$}} & \update{\underline{82.65}{\scriptsize $\pm 00.79$}} & \update{\textbf{76.12}{\scriptsize $\pm 00.87$}} & \update{\textbf{83.33}{\scriptsize $\pm 00.46$}} & \update{48.04{\scriptsize $\pm 01.78$}} & \update{57.92{\scriptsize $\pm 01.47$}}
\end{tabular}
\label{tab:pediatypes-node-hit5}
}
}
%\vspace{-15pt}  % Reduce table bottom space to the text
}
\label{tab:pediatypes-hit5}
\end{table}

\subsubsection{\ourotherdata: Testing self-supervised pre-trained zero-shot meta-learning capabilities}
\label{appx:exp-wikitopics}

As discussed in \Cref{subsec:result-wiki}, the WikiTopics dataset is created from the WikiData-5M~\citep{wang2021kepler} (under CC0 1.0 license).
Each node in the graphs of this dataset represents an entity described by an existing Wikipedia page, and each relation type corresponds to a particular relation between the entities, such as ``director of'' or ``designed by''.
The node and relation type indices are codenames that start with the prefix ``Q'' and ``P'' respectively, which are devoid of semantic meaning.
Nevertheless, WikiData-5M~\citep{wang2021kepler} provides aliases for all nodes and relation types that map their indices to textual descriptions, and we use these textual descriptions to group the relation types into 11 different topic groups, or domains (we do not however provide these textual descriptions to the models per the specification of the \ourtask task).
In total, WikiData-5M~\citep{wang2021kepler} contains 822 relation types. 
We create WikiTopics datasets from all 822 relation types, which comprise graphs with as many as 66 relation types. Each graph has a disjoint set of relation types from all other graphs.
% Below is a list of all 11 topics:
\update{\Cref{tab:wikitopics-topic-desc}~shows the 11 topics/domains of the WikiTopics dataset, each corresponding to a distinct KG with distinct relation types.}
\begin{table}[h]
    \centering
    \caption{\update{The 11 different topics/domains of the WikiTopics dataset.}}
    \resizebox{0.7\linewidth}{!}{
    \begin{tabular}{cll}
        Domain KG index & Abbreviation & Description \\
        \midrule
        T1 & Art    & Art and Media Representation \\
        T2 & Award  & Award Nomination and Achievement \\
        T3 & Edu    & Education and Academia \\
        T4 & Health & Health, Medicine, and Genetics \\
        T5 & Infra  & Infrastructure and Transportation \\
        T6 & Loc    & Location and Administrative Entity \\
        T7 & Org    & Organization and Membership \\
        T8 & People & People and Social Relationship \\
        T9 & Science    & Science, Technology, and Language \\
        T10 & Sport & Sport, and Game Competition \\
        T11 & Tax   & Taxonomy and Biology \\
    \end{tabular}}
    \label{tab:wikitopics-topic-desc}
\end{table}

% \begin{itemize}
%     \item T1 (Art): Art and Media Representation
%     \item T2 (Award): Award Nomination and Achievement
%     \item T3 (Edu): Education and Academia
%     \item T4 (Health): Health, Medicine, and Genetics
%     \item T5 (Infra): Infrastructure and Transportation
%     \item T6 (Loc): Location and Administrative Entity
%     \item T7 (Org): Organization and Membership
%     \item T8 (People): People and Social Relationship
%     \item T9 (Sci): Science, Technology, and Language,
%     \item T10 (Sport): Sport, and Game Competition
%     \item T11 (Tax): Taxonomy and Biology
% \end{itemize}

To control the overall size of the graphs in WikiTopics, we downsample $10,000$ nodes for each domain from the subgraph consisting of only the triplets with the relation types belonging to that domain.
We adopt the Forest Fire sampling procedure with burning probability $p=0.8$~\citep{SamplingGraph} implemented in the Little Ball of Fur Python package~\citep{rozemberczki2020little}.
We then split the downsampled domain KG into 90\% observable triplets and 10\% querying triplets to be predicted by the models.
When splitting, we ensure that the set of nodes in the querying triplets is a subset of those in the observable triplets.
This way, the model is not tasked with the impossible task of predicting relation types between orphaned nodes previously unseen in the observable part of the graph.
This is implemented via an iterative procedure, where we first sample a batch of missing triplets from the downsampled domain graph, then discard those that contain unseen nodes in the rest of the triplets, and repeat this process until the number of sampled triplets reaches 10\% of total triplets.
\Cref{fig:stats-wikitopics} shows the {\bf data statistics} of WikiTopics dataset. %-v1 and WikiTopics-v2 respectively.

\begin{figure}
\centering
%
% \begin{minipage}{0.49\textwidth}
% \centering
% \resizebox{\linewidth}{!}{
% \begin{tabular}{l|ccccc}
% \hline
% & \#Nodes & \# Relations & \#Triplets (Obv.) & \#Triplets (Qry.) & Avg. Deg. \\
% \hline
% Art & 10000 & 22 & 34345 & 3815 & ~~7.63 \\
% Award & 10000 & ~~6 & 25043 & 2782 & ~~5.57 \\
% Education & 10000 & ~~9 & 14898 & 1653 & ~~3.31 \\
% Health & 10000 & ~~7 & 14110 & 1566 & ~~3.14 \\
% Infrastructure & 10000 & 13 & 21778 & 2419 & ~~4.84 \\
% Location & 10000 & 11 & 22971 & 2552 & ~~5.11 \\
% Organization & 10000 & 11 & 21976 & 2441 & ~~4.88 \\
% People & 10000 & 11 & 54925 & 6102 & 12.21 \\
% Science & 10000 & 16 & 14852 & 1650 & ~~3.30 \\
% Sport & 10000 & ~~7 & 45541 & 5059 & 10.12 \\
% Taxonomy & 10000 & ~~9 & 16526 & 1834 & ~~3.67 \\
% \hline
% \end{tabular}
% }
% \includegraphics[width=\linewidth]{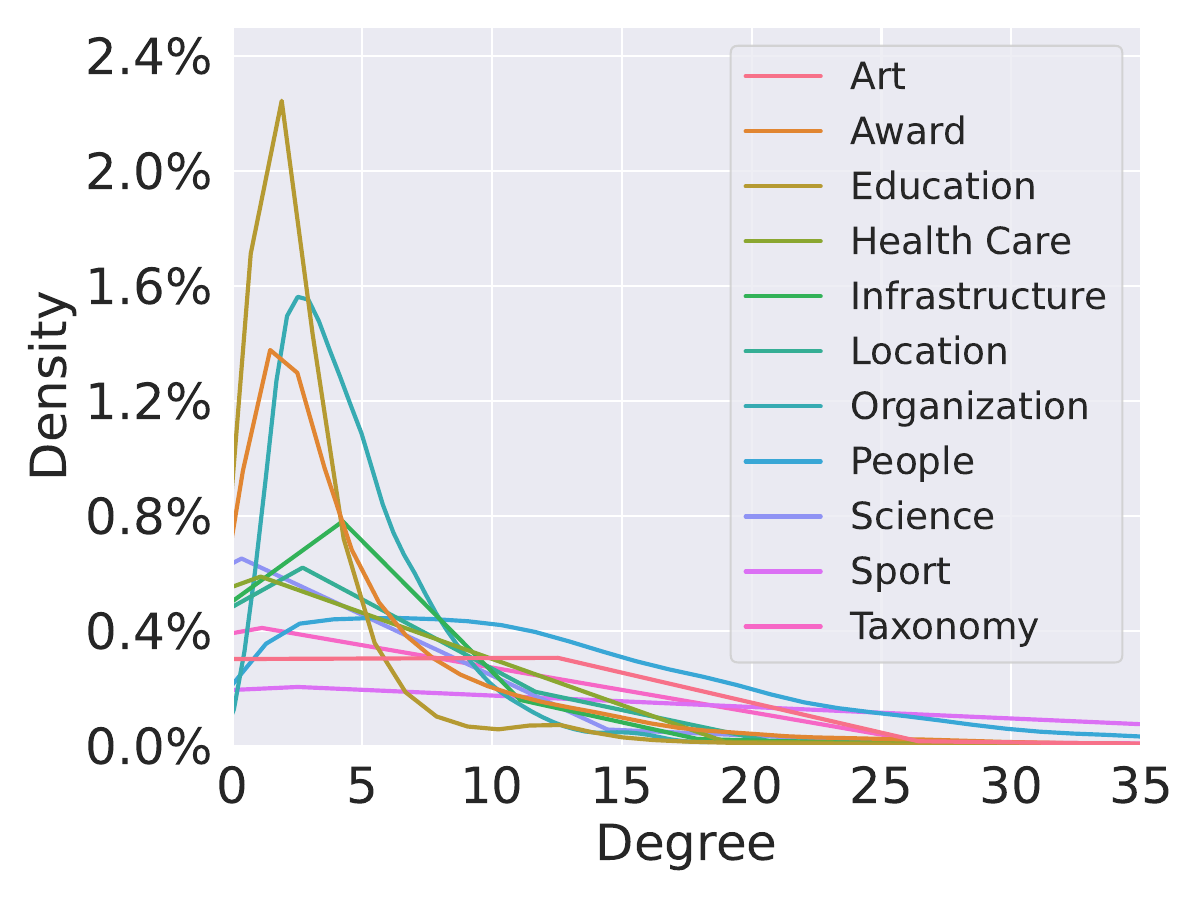}
% \subcaption{Version 1}
% \end{minipage}
% \hfill
\begin{minipage}{0.7\textwidth}
\centering
\resizebox{\linewidth}{!}{
\begin{tabular}{l|ccccc}
\hline
& \#Nodes & \# Relations & \#Triplets (Obv.) & \#Triplets (Qry.) & Avg. Deg. \\
\hline
Art & 10000 & 45 & 28023 & 3113 & ~~6.23 \\
Award & 10000 & 10 & 25056 & 2783 & ~~5.57 \\
Edu & 10000 & 15 & 14193 & 1575 & ~~3.15 \\
Health & 10000 & 20 & 15337 & 1703 & ~~3.41 \\
Infra & 10000 & 27 & 21646 & 2405 & ~~4.81 \\
Loc & 10000 & 35 & 80269 & 8918 & 17.84 \\
Org & 10000 & 18 & 30214 & 3357 & ~~6.71 \\
People & 10000 & 25 & 58530 & 6503 & 13.01 \\
Sci & 10000 & 42 & 12516 & 1388 & ~~2.78 \\
Sport & 10000 & 20 & 46717 & 5190 & 10.38 \\
Tax & 10000 & 31 & 19416 & 2157 & ~~4.32 \\
\hline
\end{tabular}
}
\includegraphics[width=\linewidth]{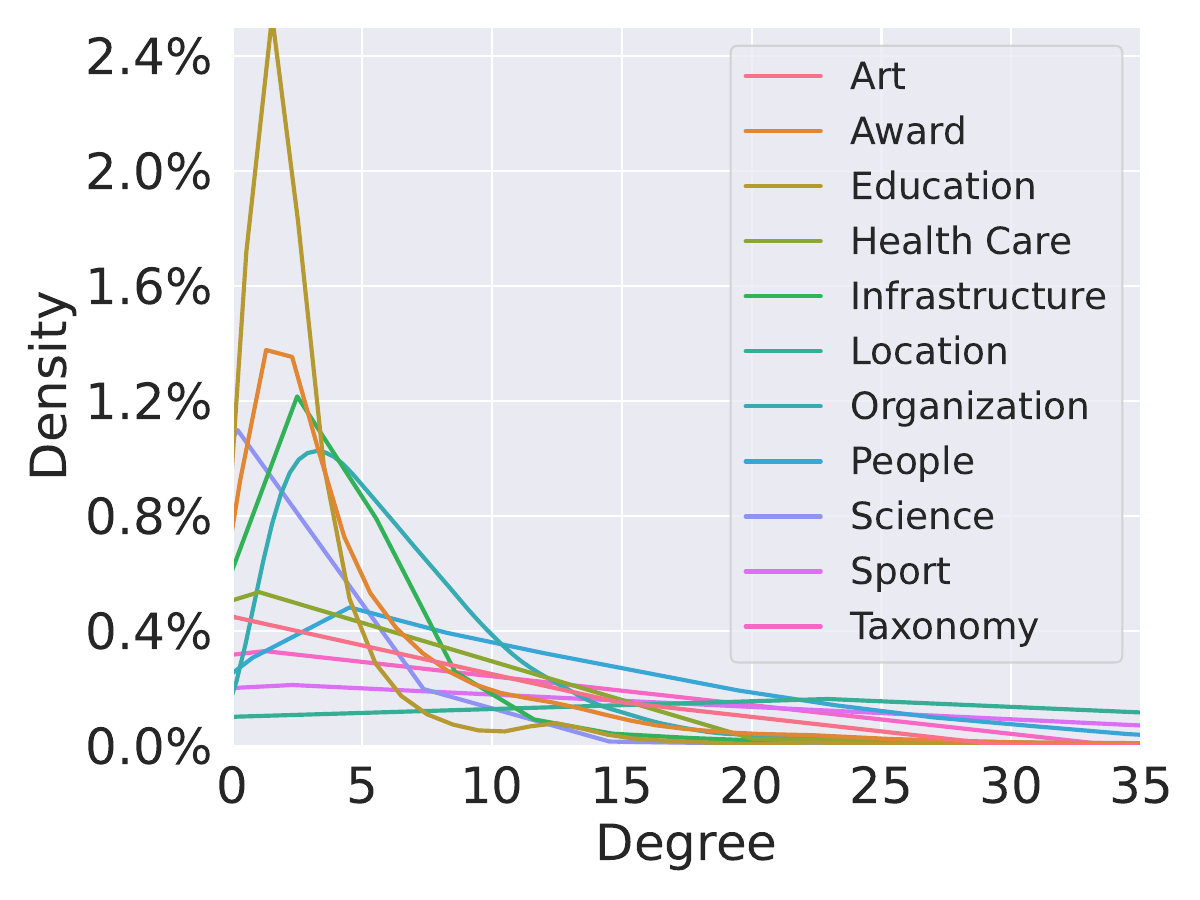}
%\subcaption{Version 2}
\end{minipage}
\caption{{\bf Statistics of WikiTopics:} We report graph statistics including the number of nodes, number of relations, observed (obv.) triplets, querying (qry.) triplets, and average degree for each graph. We also report (in \& out) degree distribution on each graph at the bottom. We omit tail distribution larger than 35 since they are fairly small and almost flat.}
\label{fig:stats-wikitopics}
\end{figure}

\paragraph{\update{Self-supervised pre-trained zero-shot meta-learning tasks over WikiTopics to train on a KG of one domain and test on a KG of a completely unseen test domain}}
\update{We train the models on each of the $11$ graphs for 5 random seeds, and for each trained model checkpoint, we cross-test it on all the other 10 graphs, resulting in a total of $550$ statistics. We report the mean results across random seeds in heatmaps.}
%In \Cref{subsec:result-wiki}, we only provide heatmaps of Relation Hits@10 Performance WikiTopics due to space limit. 
We present a detailed results (heatmaps with values) of Node and Relation Hits@10, Hits@1, and MRR for WikiTopics in \Cref{fig:wikitopics-full,fig:wikitopics-node-full}. Due to the large number of runs ($11\times 10=110$ different train-test scenarios, each with 5 random seeds, resulting in a total of 550 runs) and the time constraints to run all baseline models, we perform the evaluation over only the three models (\update{\OurNewModel}, \OurOtherModel, and InGram) that are designed for our \ourtask task. \Cref{fig:wikitopics-full} shows that for the task of predicting missing relation types $(i, ?, j)$, \update{\OurNewModel} and \OurOtherModel are consistently better than InGram across all different metrics. Especially, the structural double equivariant \update{\OurNewModel} model exhibits more consistent results across different train-test scenarios than both \OurOtherModel and InGram, and achieves significantly better results in Hits@1 and MRR, showcasing its ability for \ourtask in a much harder evaluation scenario.
For the task of prediction missing nodes $(i, k, ?)$ as shown in~\Cref{fig:wikitopics-node-full}, \update{\OurNewModel}, \OurOtherModel, and InGram showcase comparable performance, whereas \update{\OurNewModel} exhibits more consistent results across different train-test scenarios than both \OurOtherModel and InGram. We also note that similar to the relation prediction task, \update{\OurNewModel} also exhibits the best performance in the Hits@1 metric for the node prediction task.
%We can see that the performance is consistent in WikiTopics-v1 and WikiTopics-v2 that \OurModel is always better than other baselines, while GIN, GAT and GraphConv are extremely poor. On MRR metric, although there are several cases where \OurModel performs poorly, \OurModel is always better than NBFNet* except one case on WikiTopics-v2. On Hits@10 metric, \OurModel is mostly better than NBFNet* except several poor cases where \OurModel is worse than NBFNet*. We suppose the reason for those poor cases is that exchangeable representation of \OurModel ranks a lot negative triplets with similar scores as positive since knowledge learned from training can not distinguish them due to difference between logic behind them. This behavior may share similar reason as the expressivity limitation shown in \Cref{subsubsec:limit}.
% To summary, \OurModel is always better than NBFNet* except several corner cases on Hits@10 metrics which may relate to expressivity limitation caused by high exchangeability.

\begin{figure}[t]
   % \vspace{-15pt}  % Reduce figure head space to the top of the page
    \centering
    % Row 1 - Hits@10
    \begin{subfigure}[b]{0.32\textwidth}
        \centering        
        \includegraphics[width=\linewidth,height=0.84\linewidth]{figs/ISDEA+-hits@10-relation.png}
        \vspace{-10pt}
        % \caption{\OurModel Hits@10}
        \caption{\update{\update{\OurNewModel} Hits@10}}
    \end{subfigure}
    \hfill
    \begin{subfigure}[b]{0.27\textwidth}
        \centering
        \includegraphics[width=\linewidth,height=\linewidth]{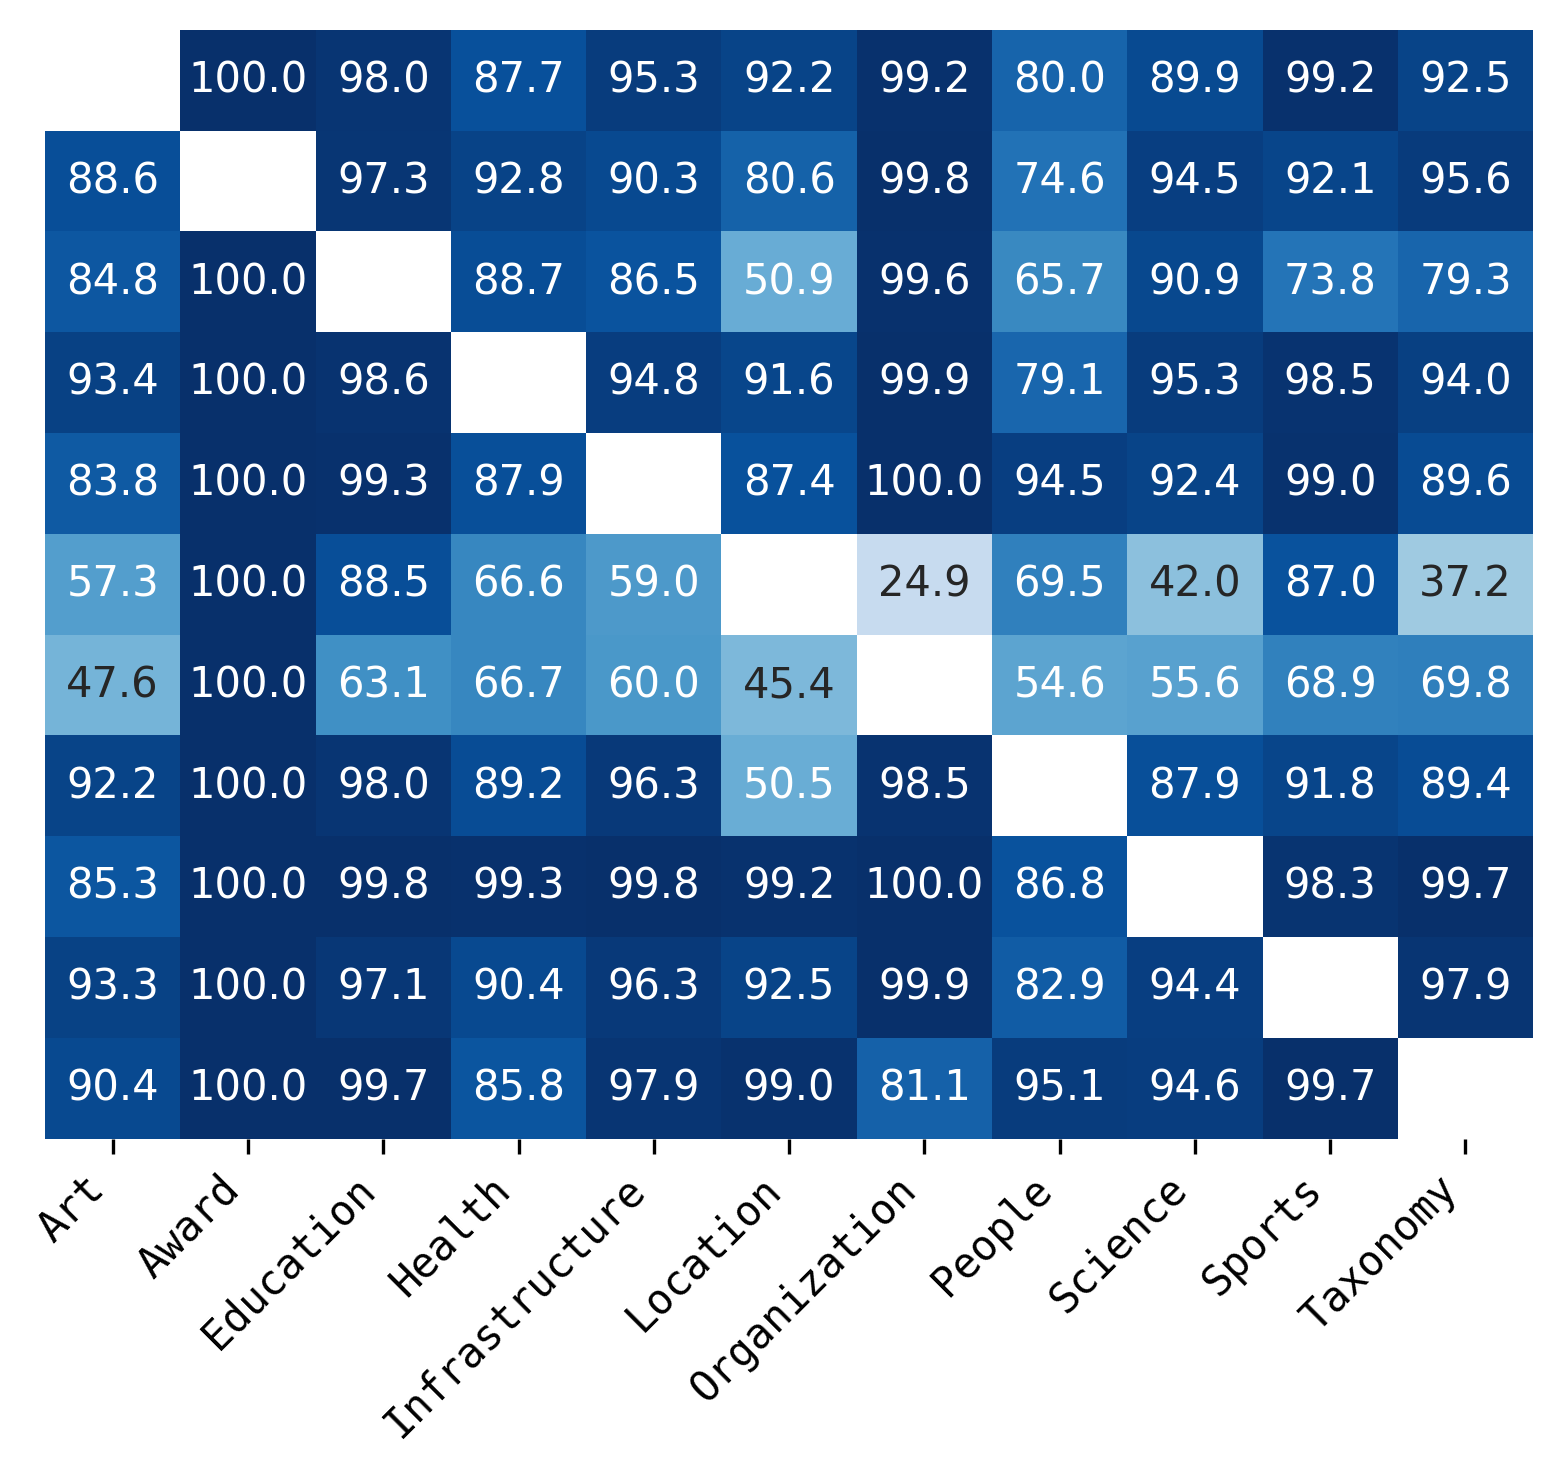}
        \vspace{-10pt}
        \caption{\OurOtherModel Hits@10}
    \end{subfigure}
    \hfill
    \begin{subfigure}[b]{0.31\textwidth}
        \centering
        \includegraphics[width=\linewidth,height=0.88\linewidth]{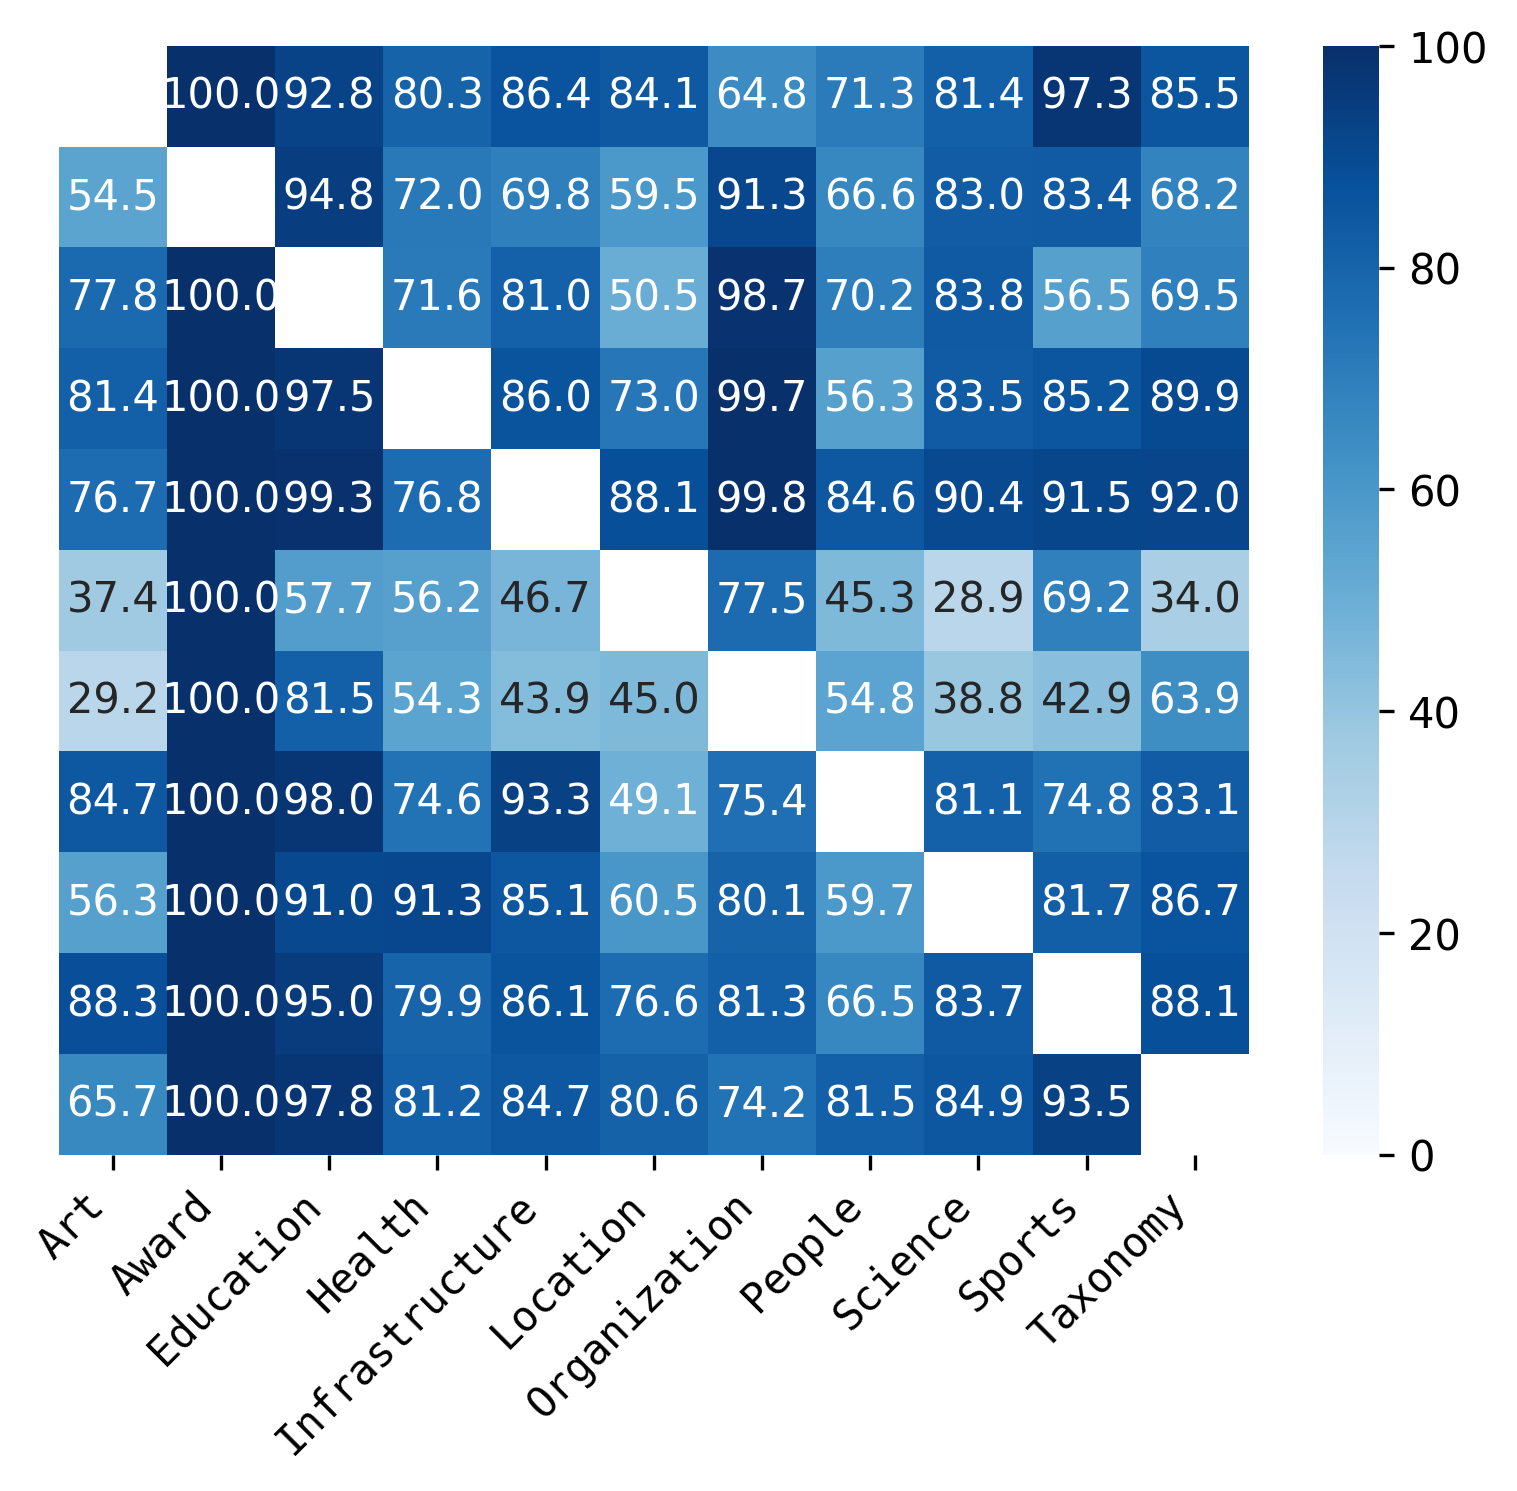}
        \vspace{-10pt}
        \caption{Original InGram Hits@10}
    \end{subfigure}
    % Row 2 - Hits@1
    \begin{subfigure}[b]{0.32\textwidth}
        \centering        
        \includegraphics[width=\linewidth,height=0.84\linewidth]{figs/ISDEA+-hits@1-relation.png}
        \vspace{-10pt}
        % \caption{\OurModel Hits@1}
        \caption{\update{\update{\OurNewModel} Hits@1}}
    \end{subfigure}
    \hfill
    \begin{subfigure}[b]{0.27\textwidth}
        \centering
        \includegraphics[width=\linewidth,height=\linewidth]{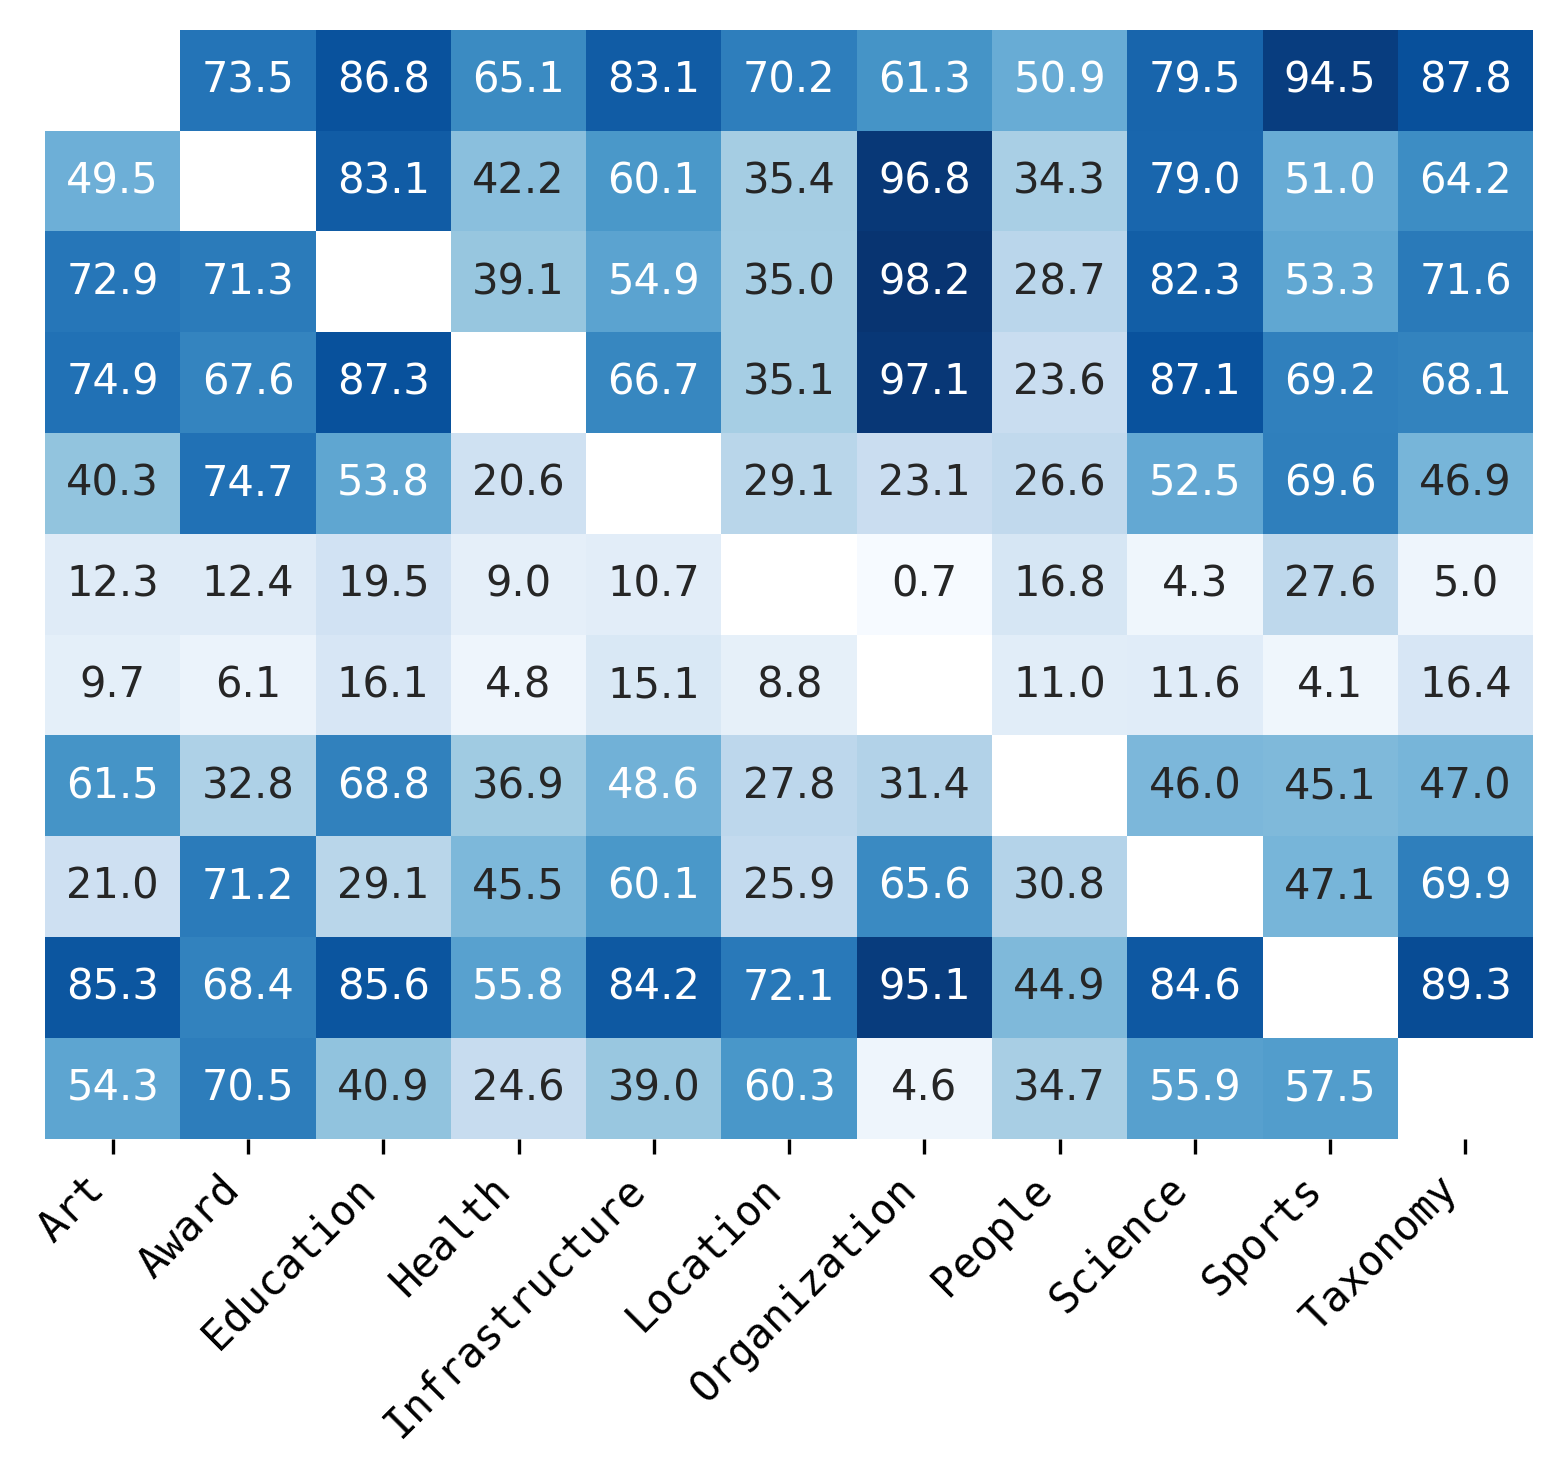}
        \vspace{-10pt}
        \caption{\OurOtherModel Hits@1}
    \end{subfigure}
    \hfill
    \begin{subfigure}[b]{0.31\textwidth}
        \centering
        \includegraphics[width=\linewidth,height=0.88\linewidth]{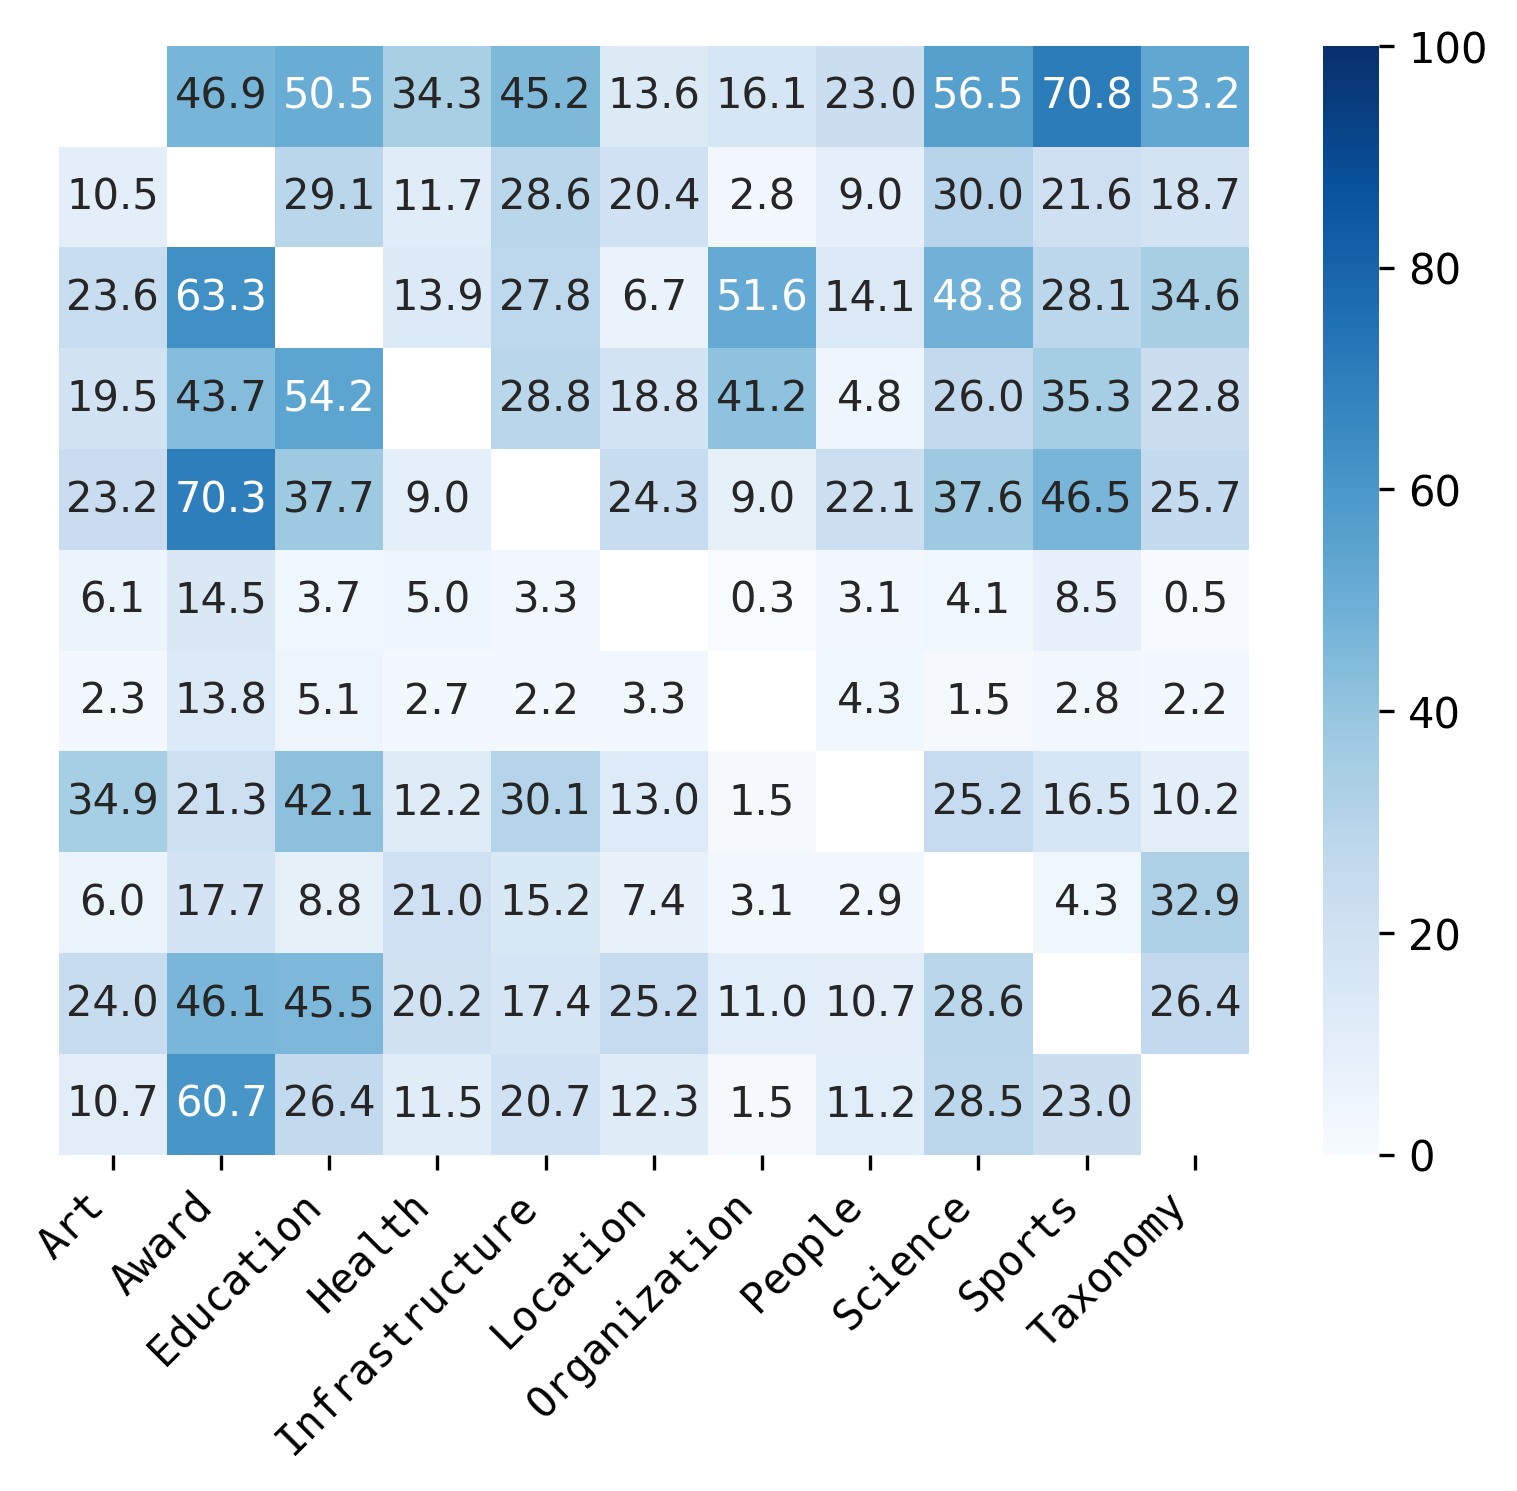}
        \vspace{-10pt}
        \caption{Original InGram Hits@1}
    \end{subfigure}
    % Row 3 - MRR
    \begin{subfigure}[b]{0.32\textwidth}
        \centering        
        \includegraphics[width=\linewidth,height=0.84\linewidth]{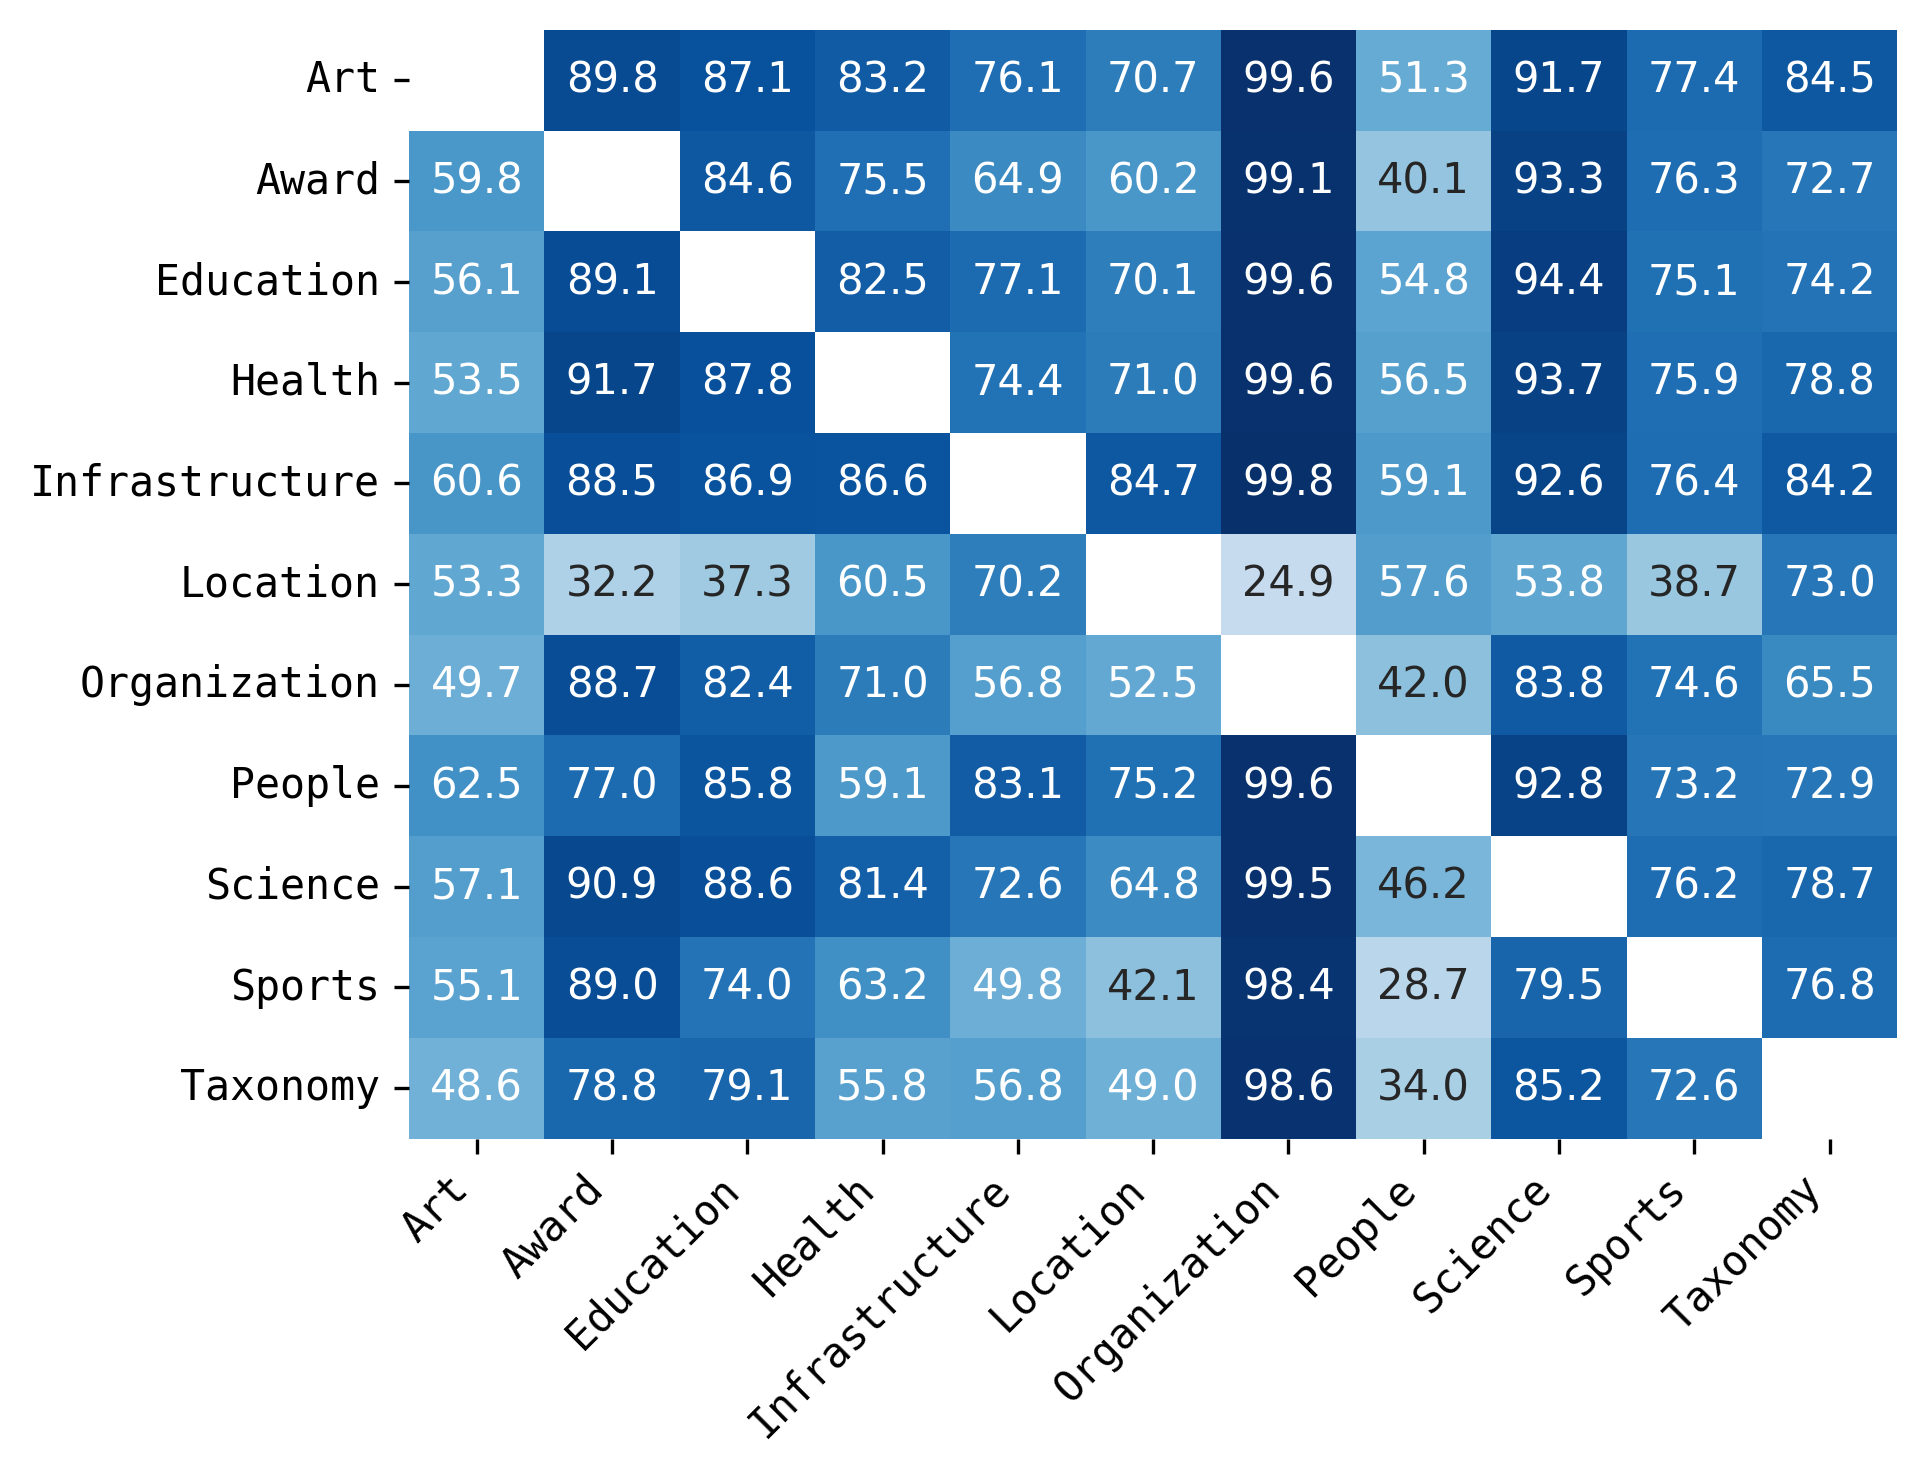}
        \vspace{-10pt}
        % \caption{\OurModel MRR}
        \caption{\update{\update{\OurNewModel} MRR}}
    \end{subfigure}
    \hfill
    \begin{subfigure}[b]{0.27\textwidth}
        \centering
        \includegraphics[width=\linewidth,height=\linewidth]{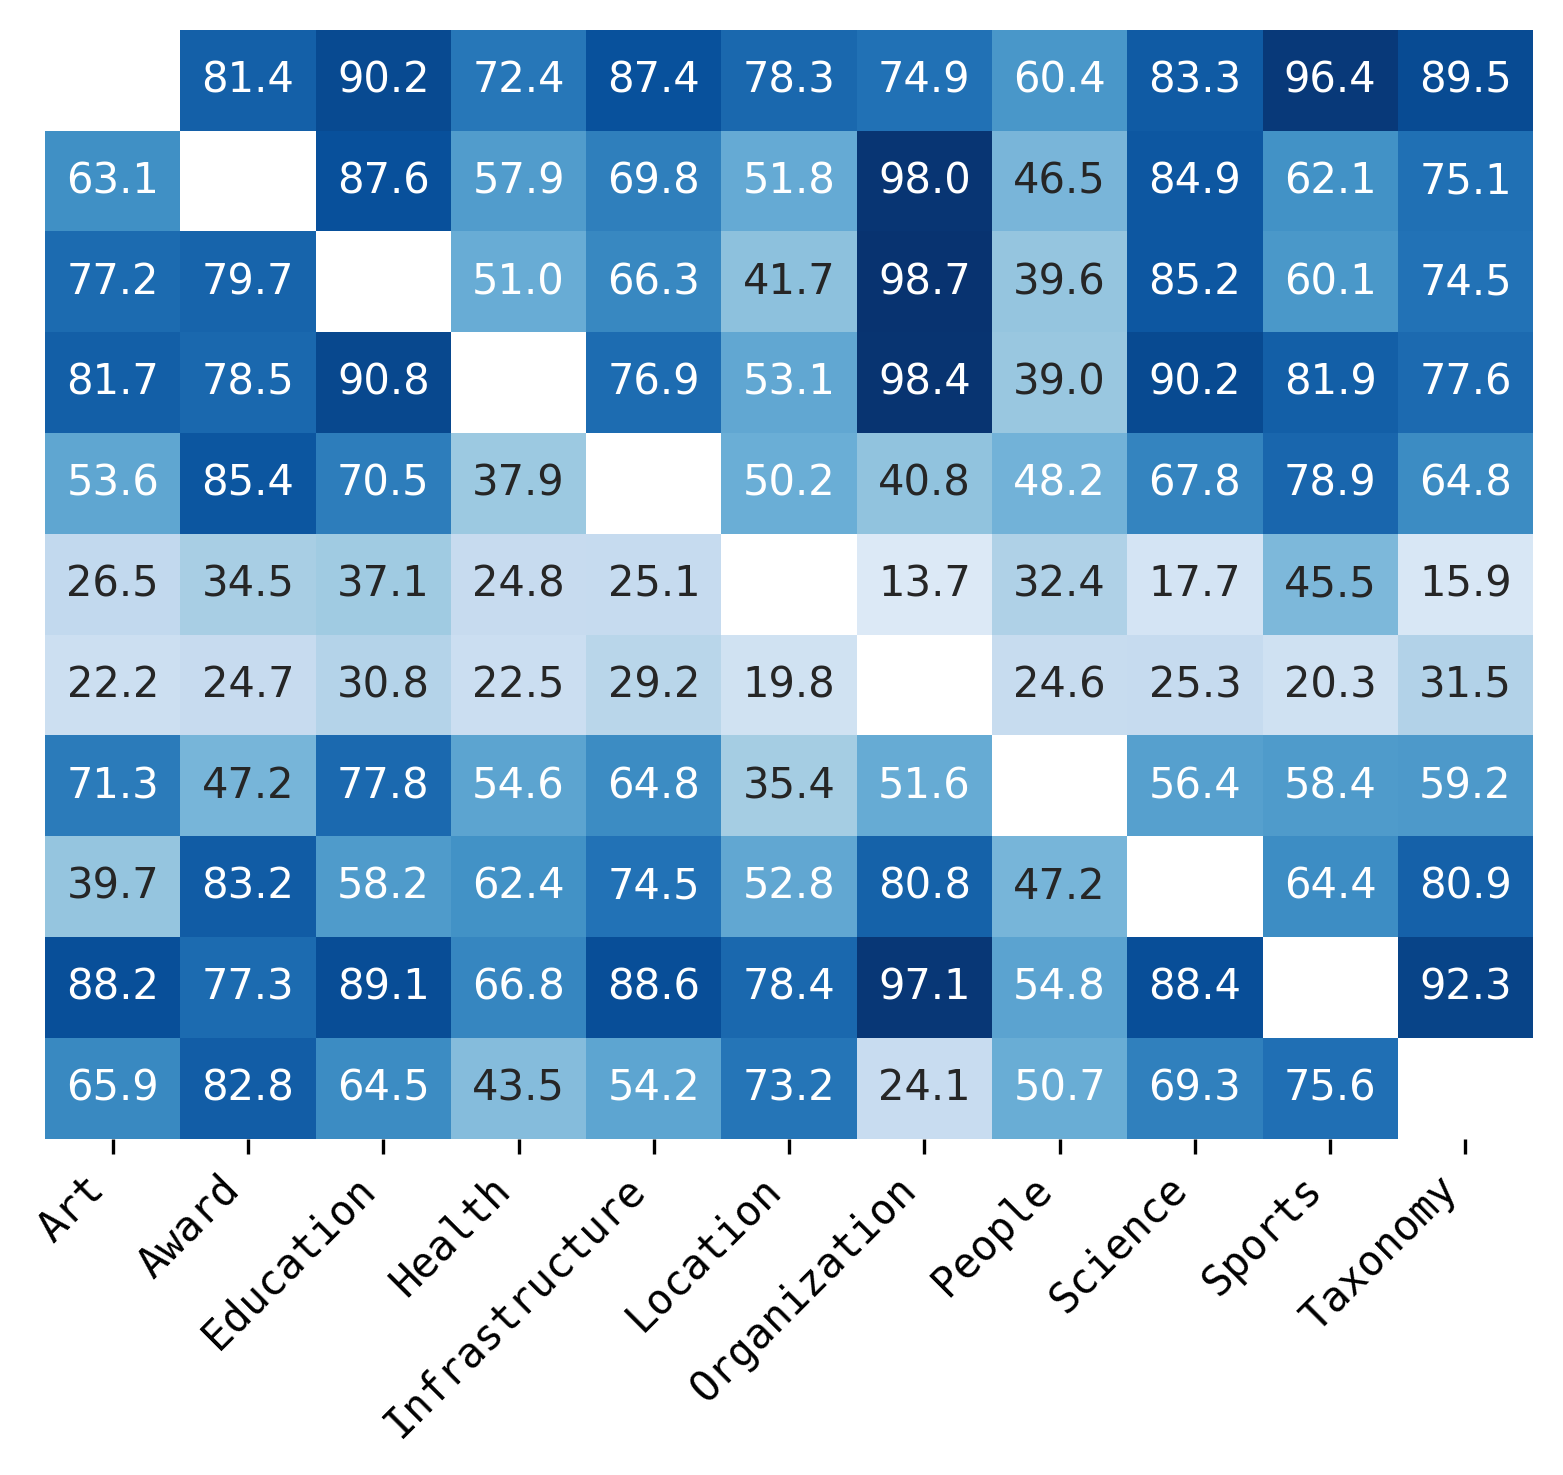}
        \vspace{-10pt}
        \caption{\OurOtherModel MRR}
    \end{subfigure}
    \hfill
    \begin{subfigure}[b]{0.31\textwidth}
        \centering
        \includegraphics[width=\linewidth,height=0.88\linewidth]{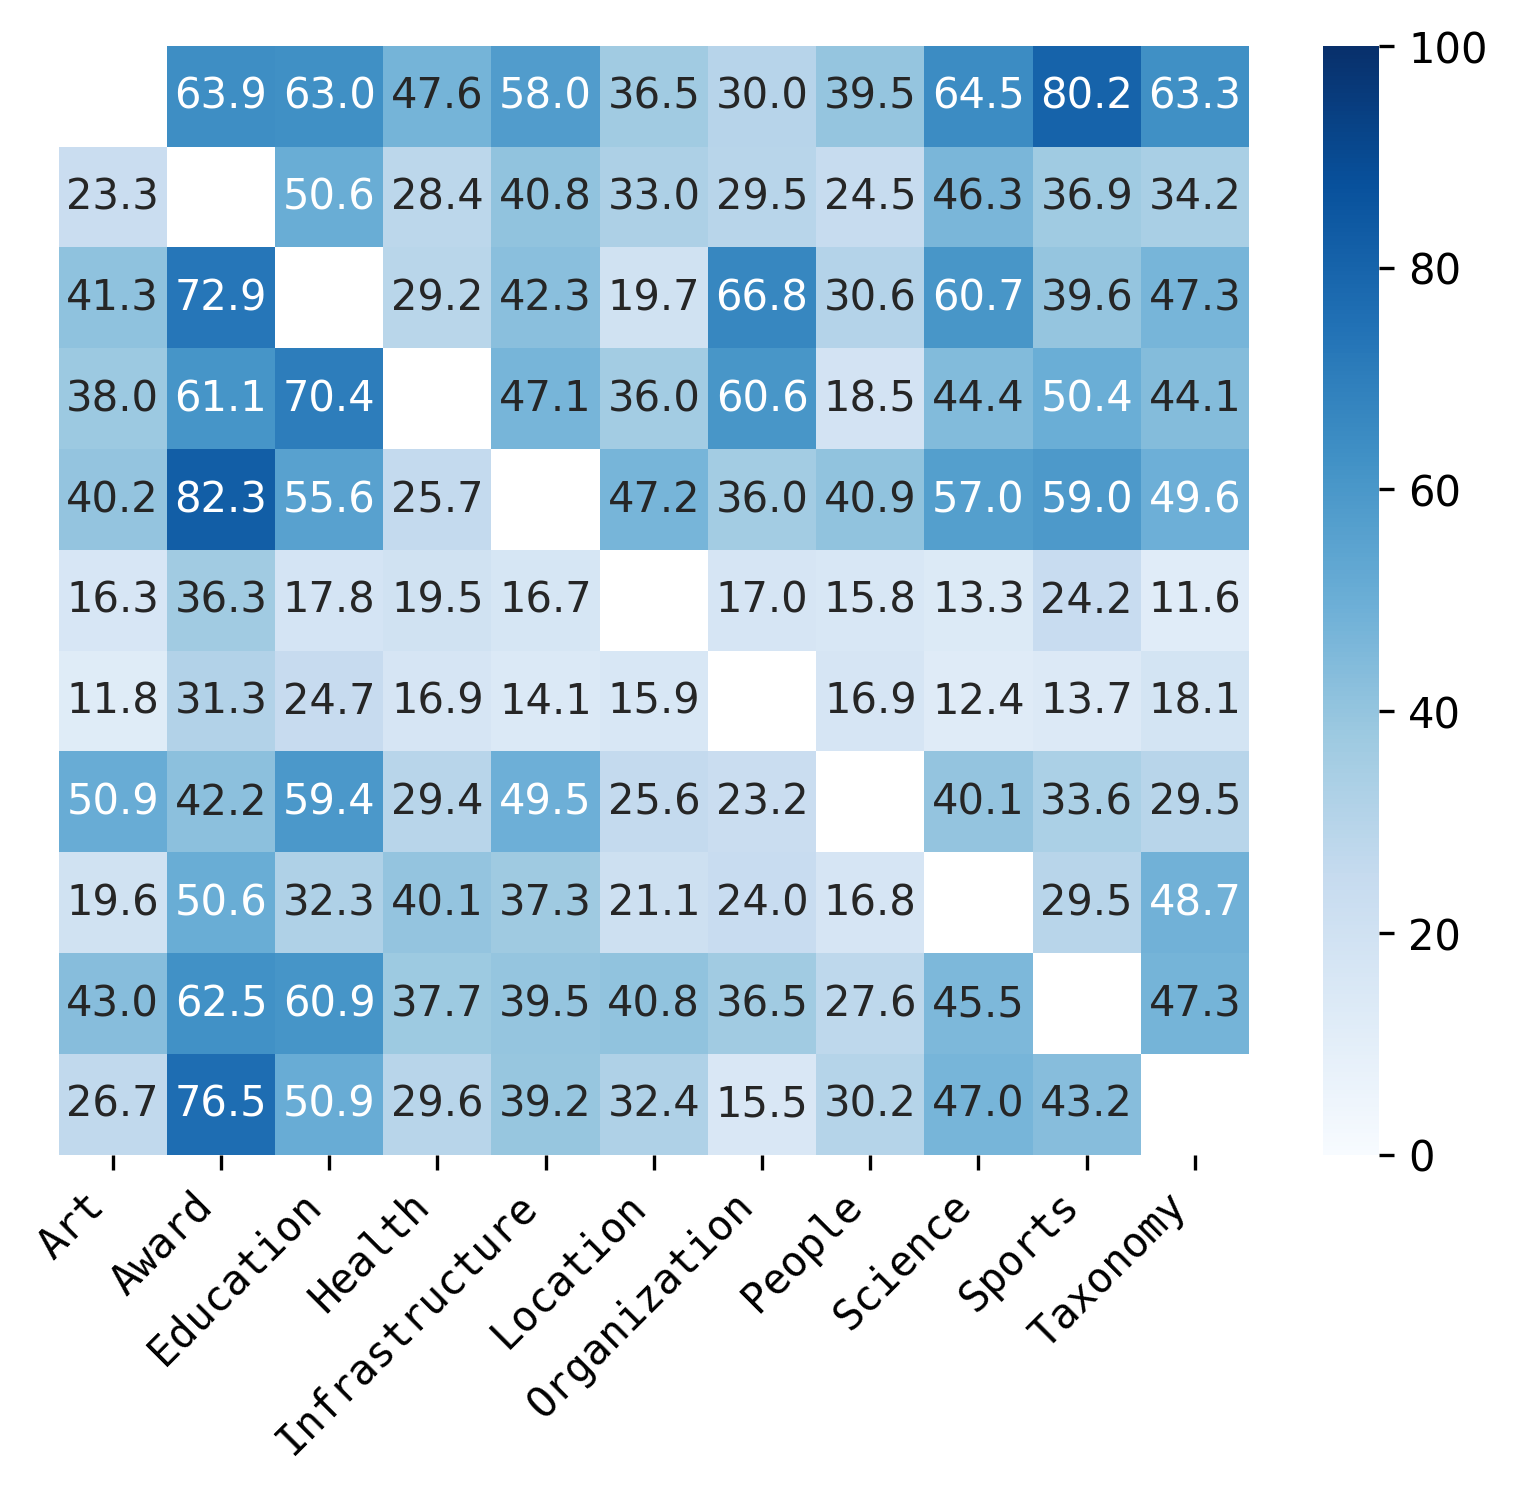}
        \vspace{-10pt}
        \caption{Original InGram MRR}
    \end{subfigure}
    \vspace{-5pt}
    \caption{{\bf Relation prediction $(i, ?, j)$ performance over WikiTopics} for \update{\OurNewModel}, \OurOtherModel, and InGram~\citep{ingram}. Each row within each heatmap corresponds to a training graph, and each column within each heatmap corresponds to a test graph. A darker color means better performance. 
    \textbf{Both \OurModel, \OurOtherModel perform significantly better than InGram, especially for Hits@1 and MRR, whereas \update{\OurNewModel} exhibits more consistent results across different train-test scenarios than both \OurOtherModel and InGram.}
    }
    %\vspace{-15pt}  % Reduce figure bottom space to the text
    \label{fig:wikitopics-full}
\end{figure}

\begin{figure}[t]
   % \vspace{-15pt}  % Reduce figure head space to the top of the page
    \centering
    % Row 1 - Hits@10
    \begin{subfigure}[b]{0.32\textwidth}
        \centering        
        \includegraphics[width=\linewidth,height=0.84\linewidth]{figs/ISDEA+-hits@10-node.png}
        \vspace{-10pt}
        % \caption{\OurModel Hits@10}
        \caption{\update{\update{\OurNewModel} Hits@10}}
    \end{subfigure}
    \hfill
    \begin{subfigure}[b]{0.27\textwidth}
        \centering
        \includegraphics[width=\linewidth,height=\linewidth]{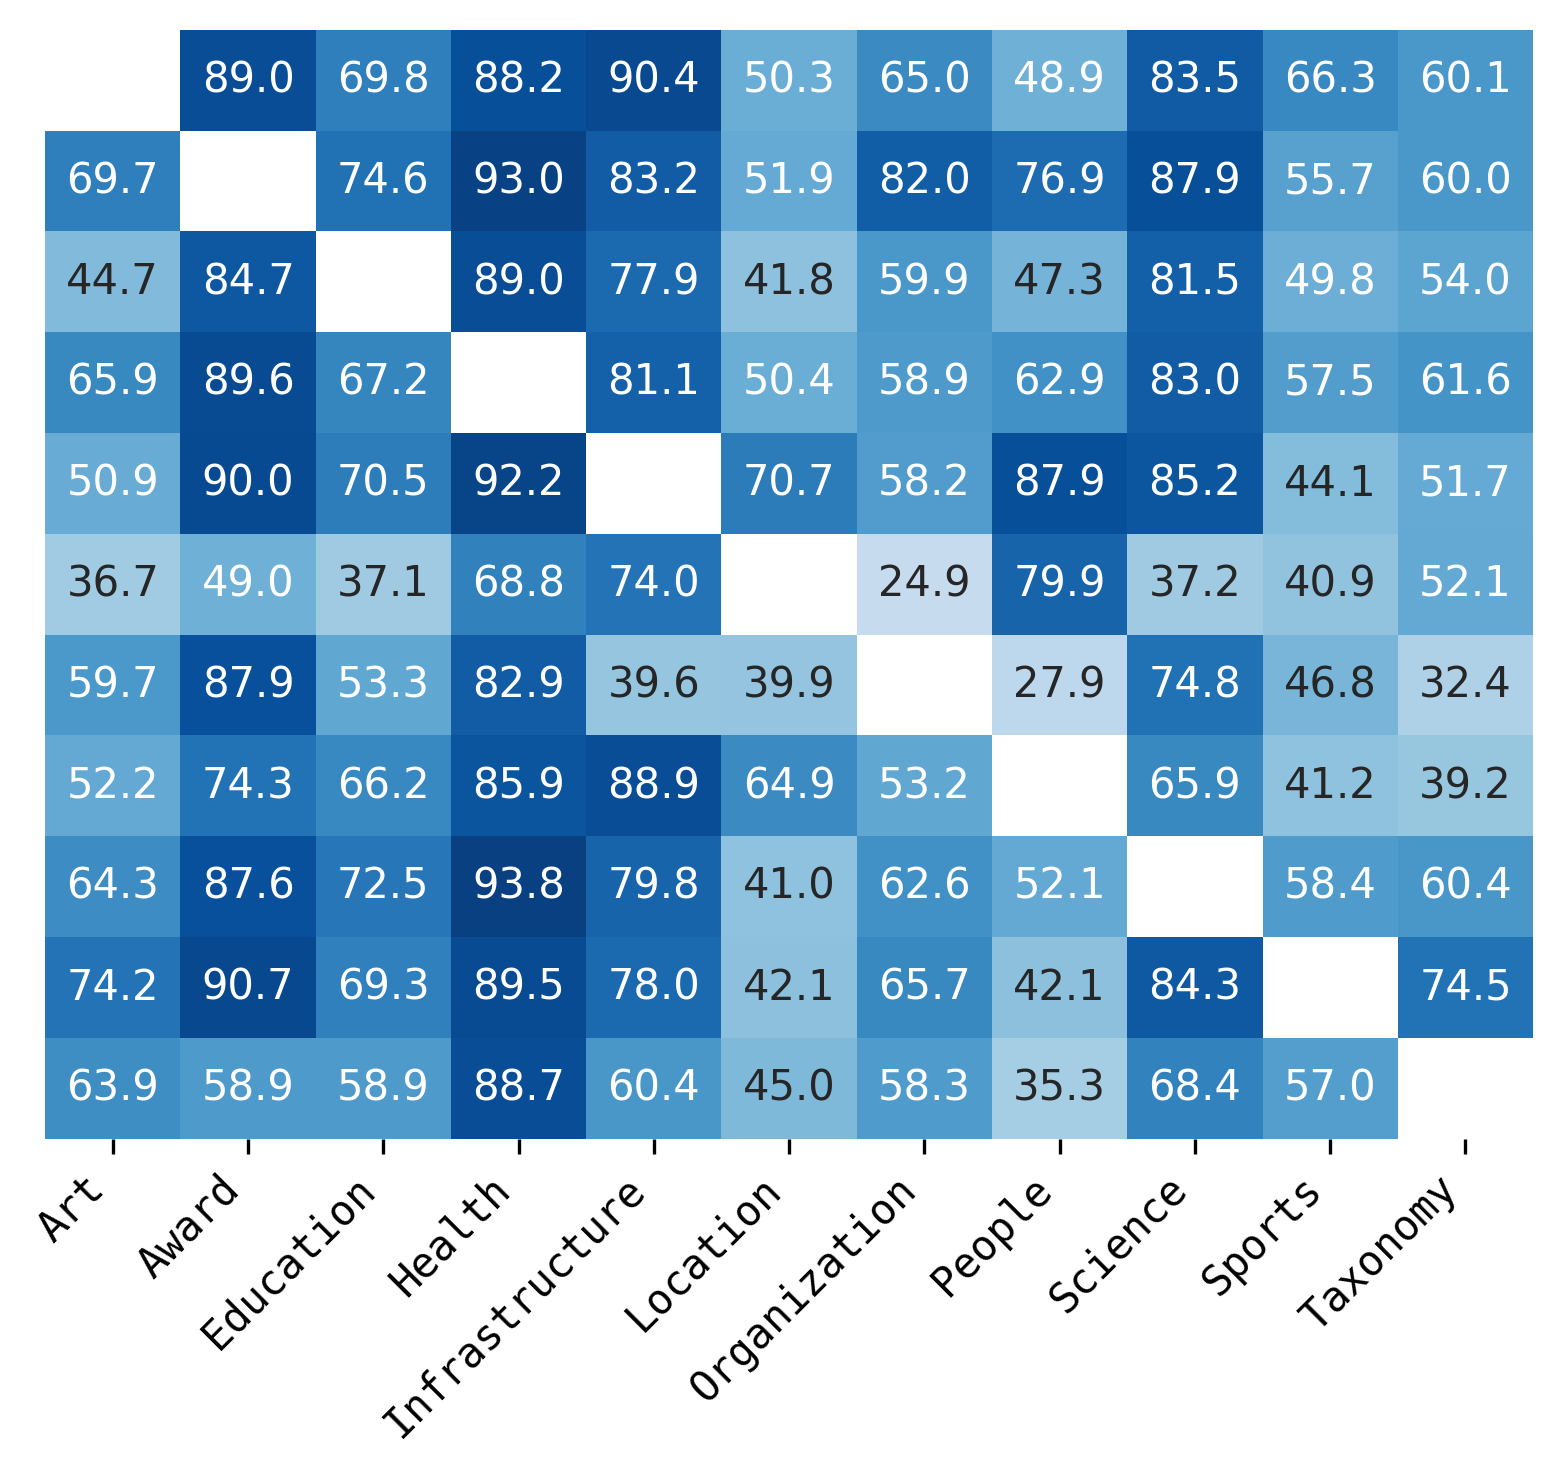}
        \vspace{-10pt}
        \caption{\OurOtherModel Hits@10}
    \end{subfigure}
    \hfill
    \begin{subfigure}[b]{0.31\textwidth}
        \centering
        \includegraphics[width=\linewidth,height=0.88\linewidth]{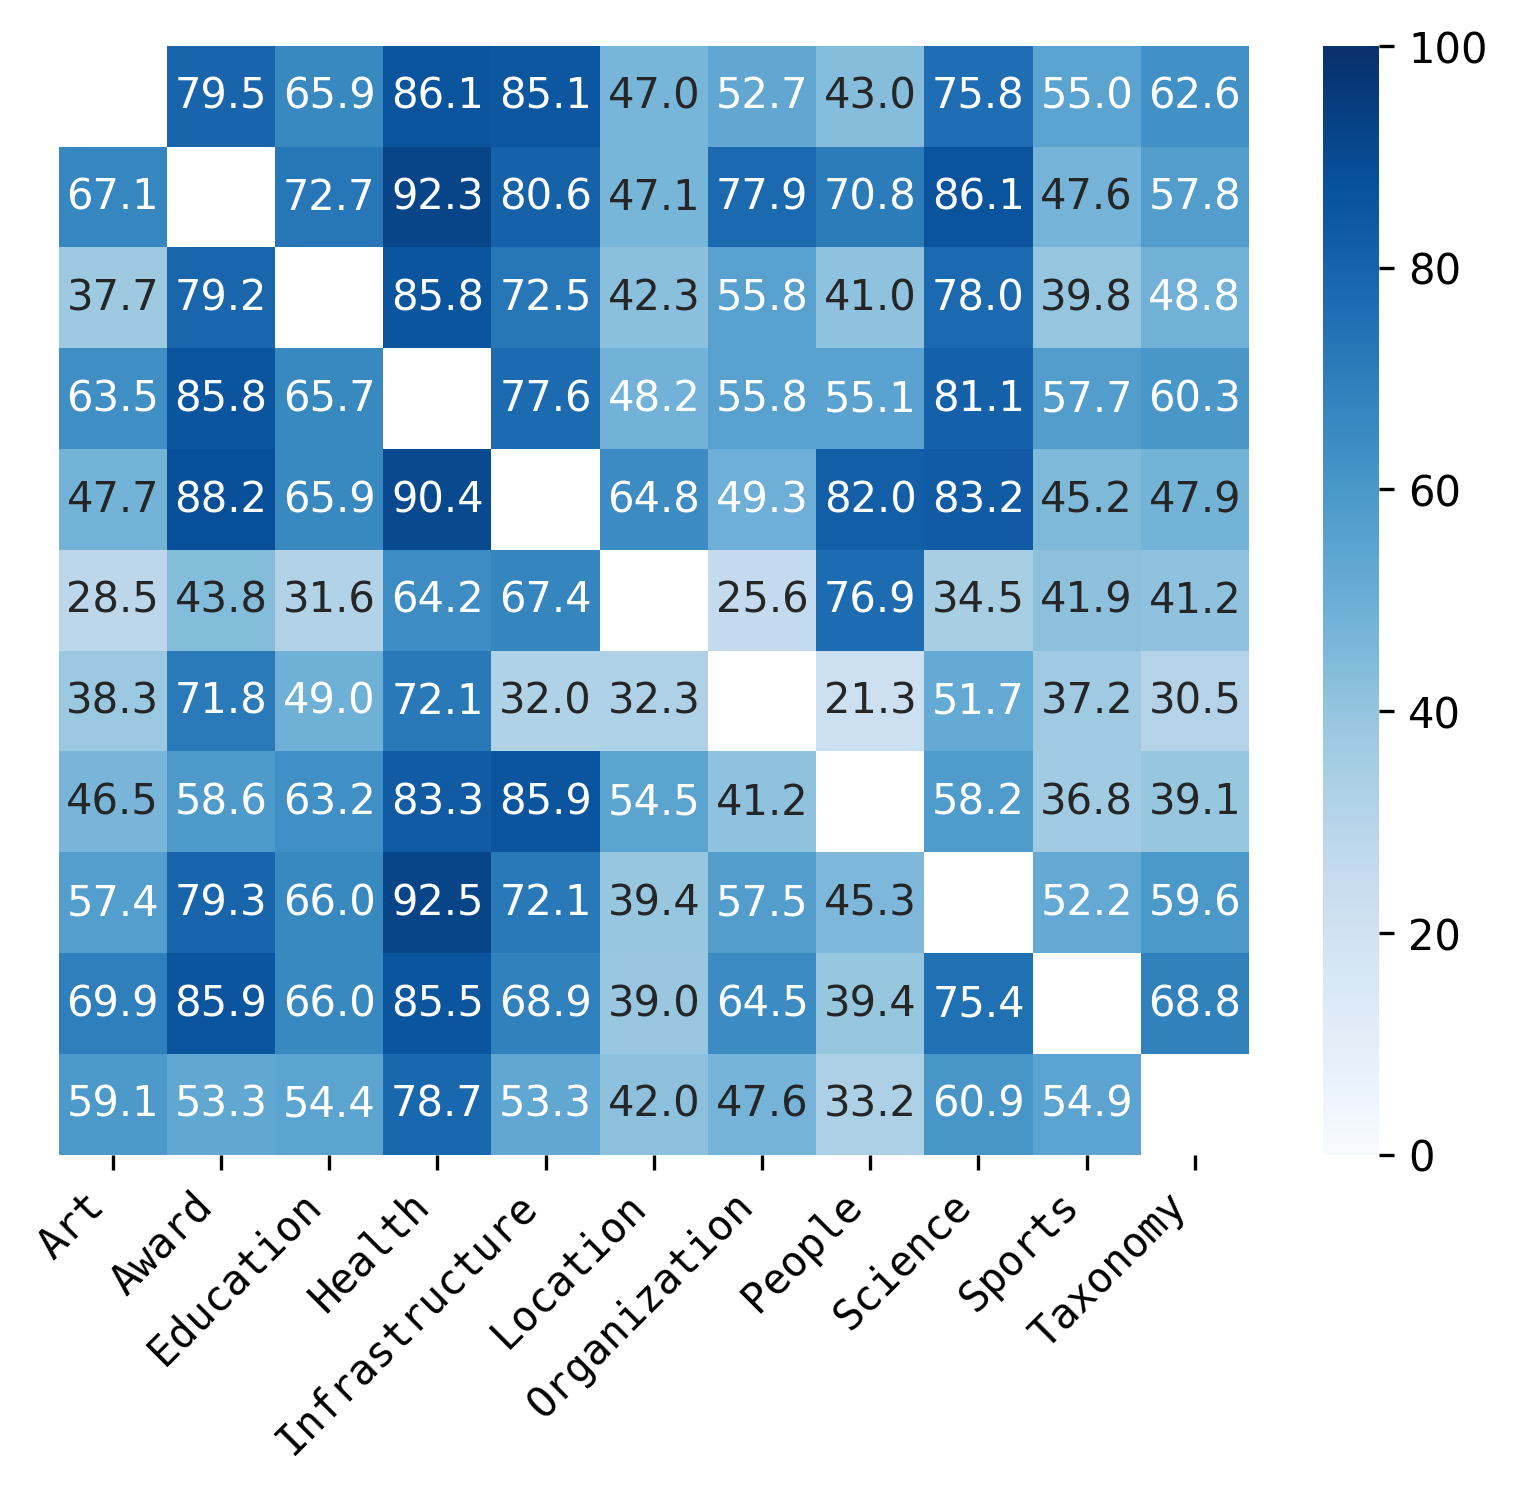}
        \vspace{-10pt}
        \caption{Original InGram Hits@10}
    \end{subfigure}
    % Row 2 - Hits@1
    \begin{subfigure}[b]{0.32\textwidth}
        \centering        
        \includegraphics[width=\linewidth,height=0.84\linewidth]{figs/ISDEA+-hits@1-node.png}
        \vspace{-10pt}
        % \caption{\OurModel Hits@1}
        \caption{\update{\update{\OurNewModel} Hits@1}}
    \end{subfigure}
    \hfill
    \begin{subfigure}[b]{0.27\textwidth}
        \centering
        \includegraphics[width=\linewidth,height=\linewidth]{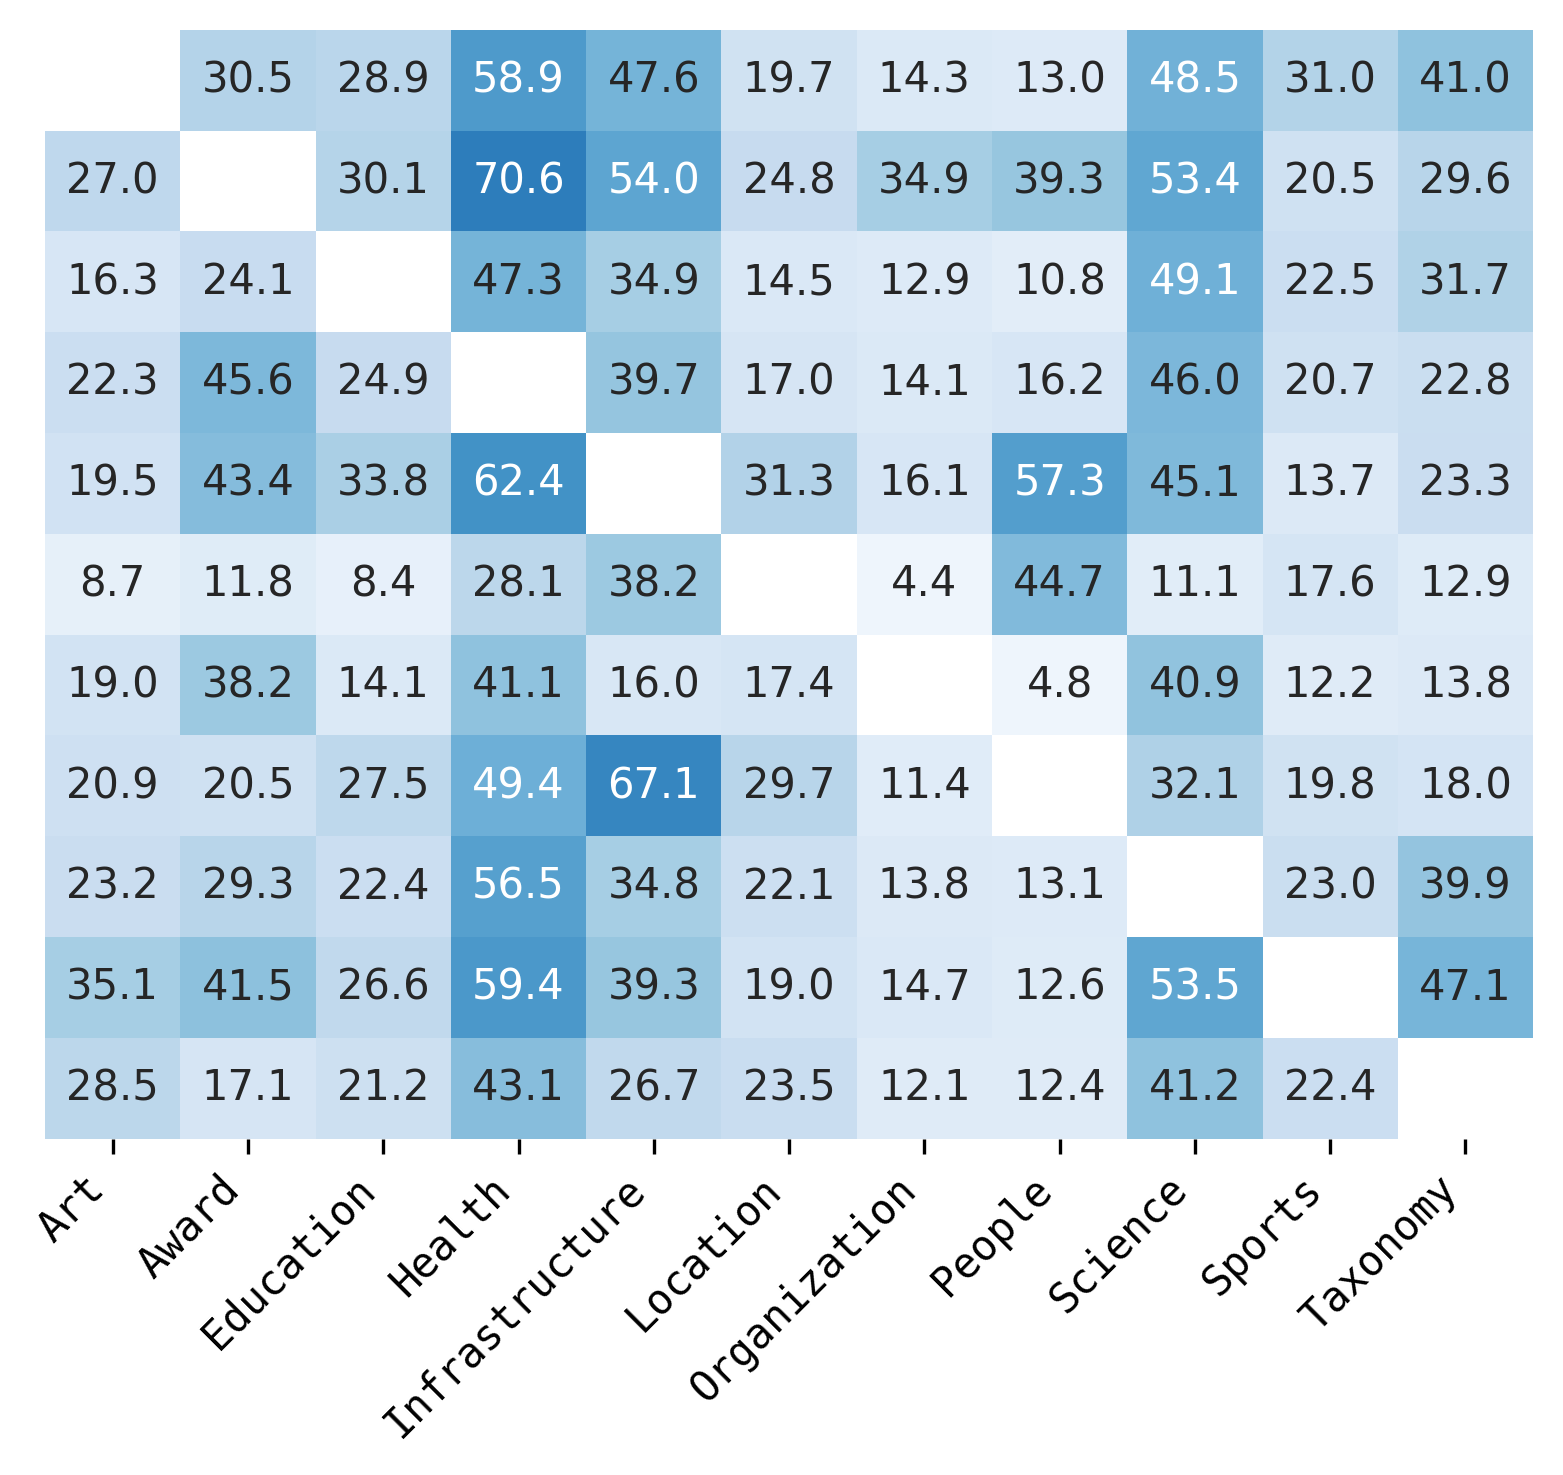}
        \vspace{-10pt}
        \caption{\OurOtherModel Hits@1}
    \end{subfigure}
    \hfill
    \begin{subfigure}[b]{0.31\textwidth}
        \centering
        \includegraphics[width=\linewidth,height=0.88\linewidth]{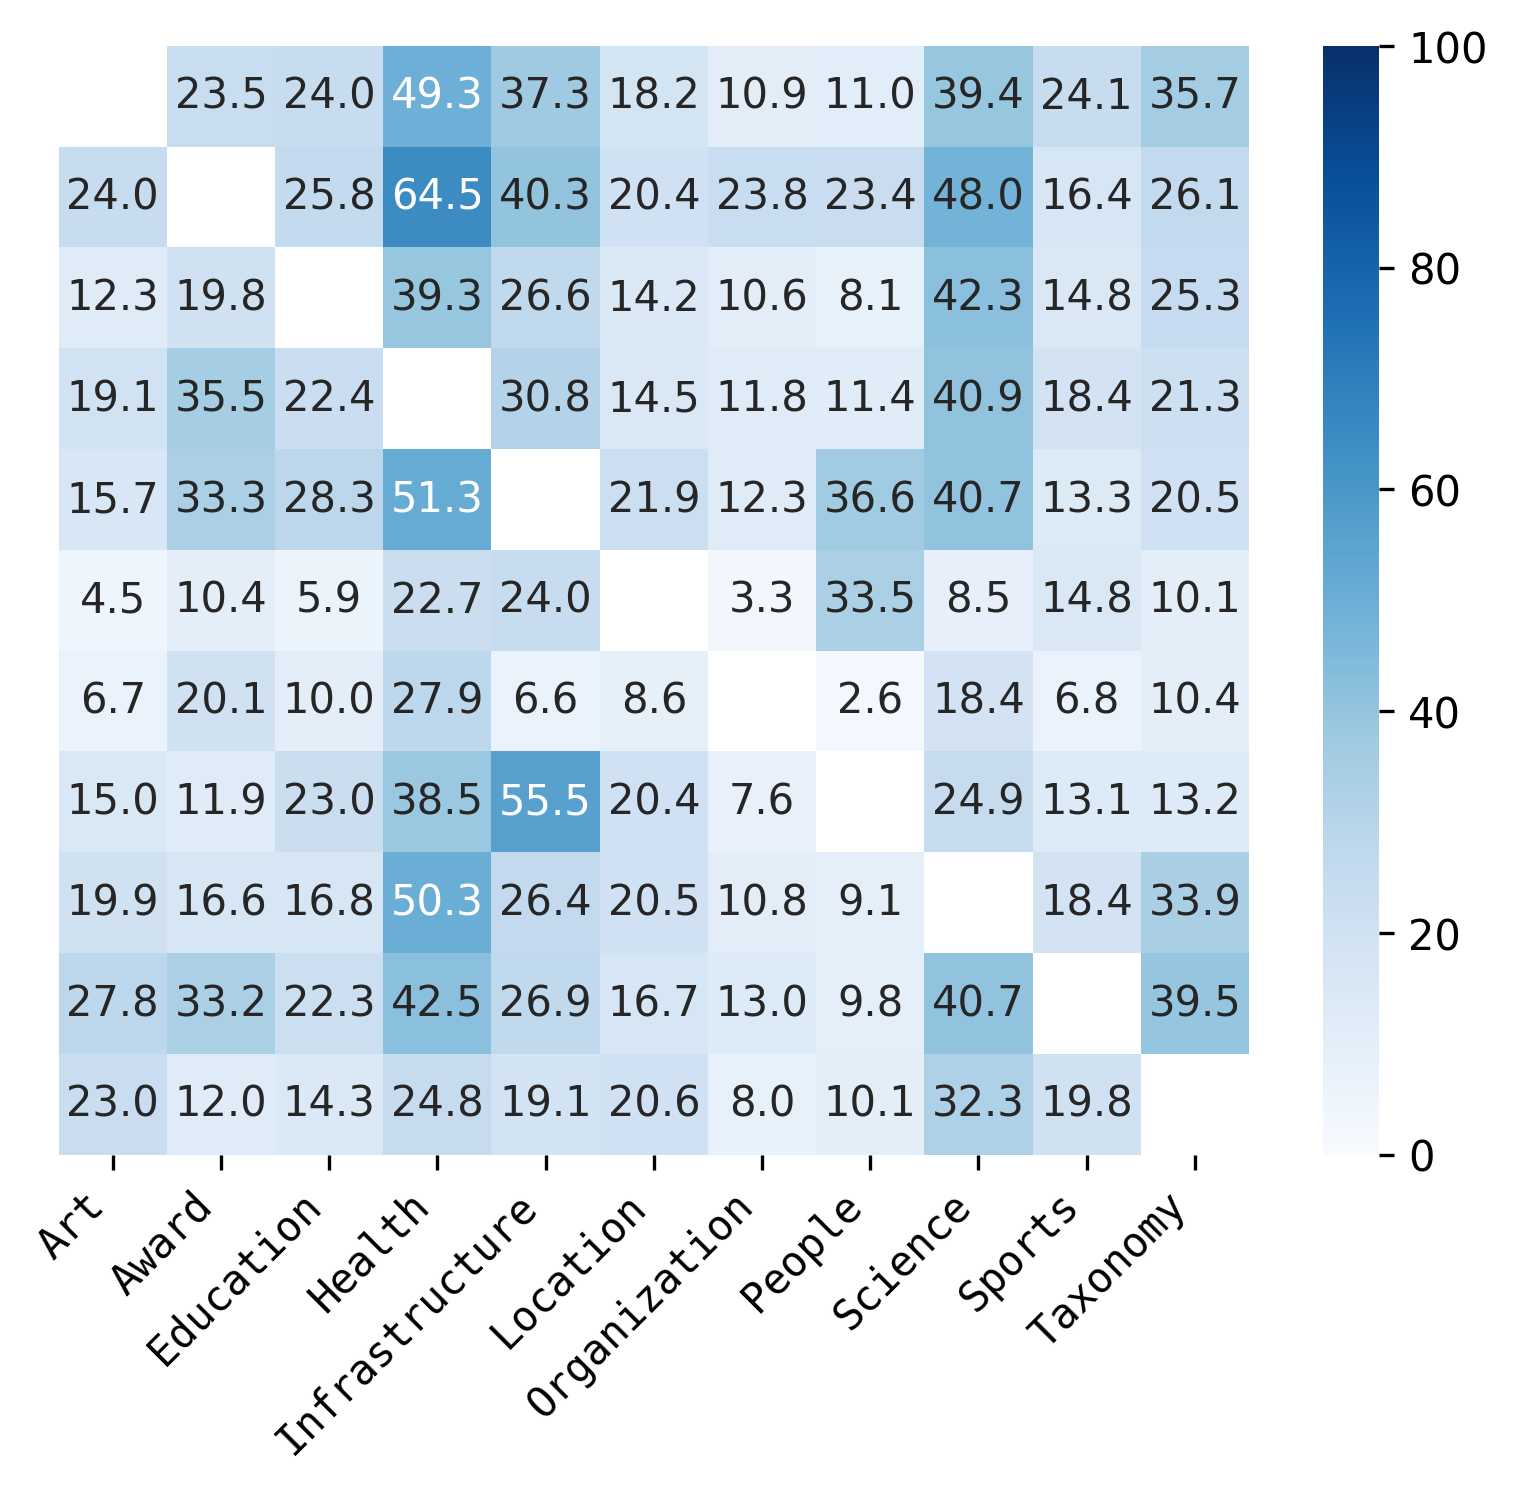}
        \vspace{-10pt}
        \caption{Original InGram Hits@1}
    \end{subfigure}
    % Row 3 - MRR
    \begin{subfigure}[b]{0.32\textwidth}
        \centering        
        \includegraphics[width=\linewidth,height=0.84\linewidth]{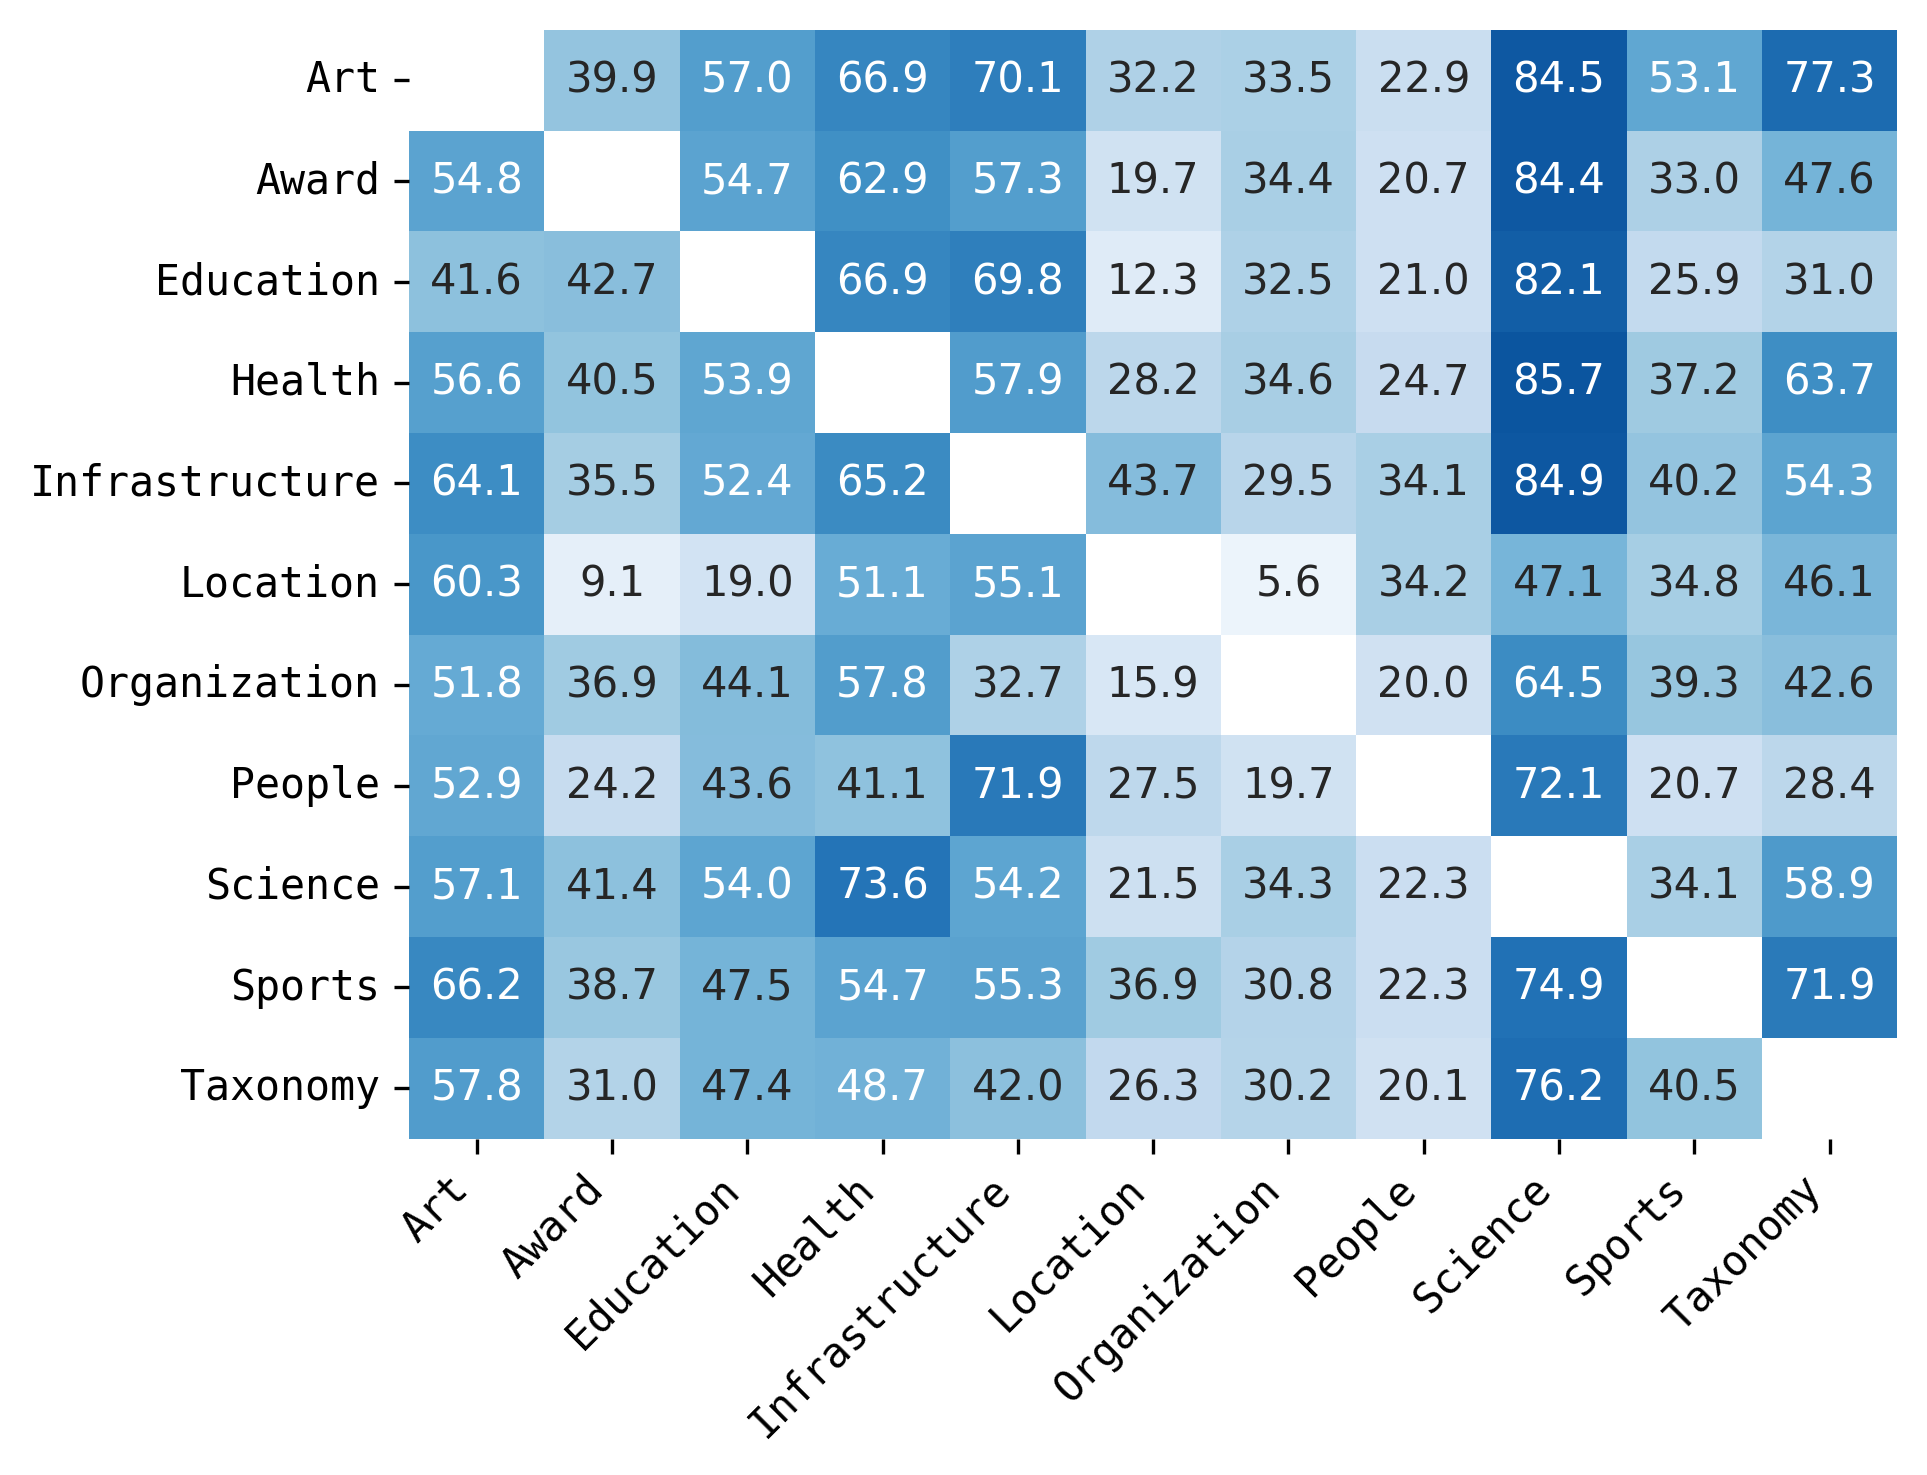}
        \vspace{-10pt}
        % \caption{\OurModel MRR}
        \caption{\update{\update{\OurNewModel} MRR}}
    \end{subfigure}
    \hfill
    \begin{subfigure}[b]{0.27\textwidth}
        \centering
        \includegraphics[width=\linewidth,height=\linewidth]{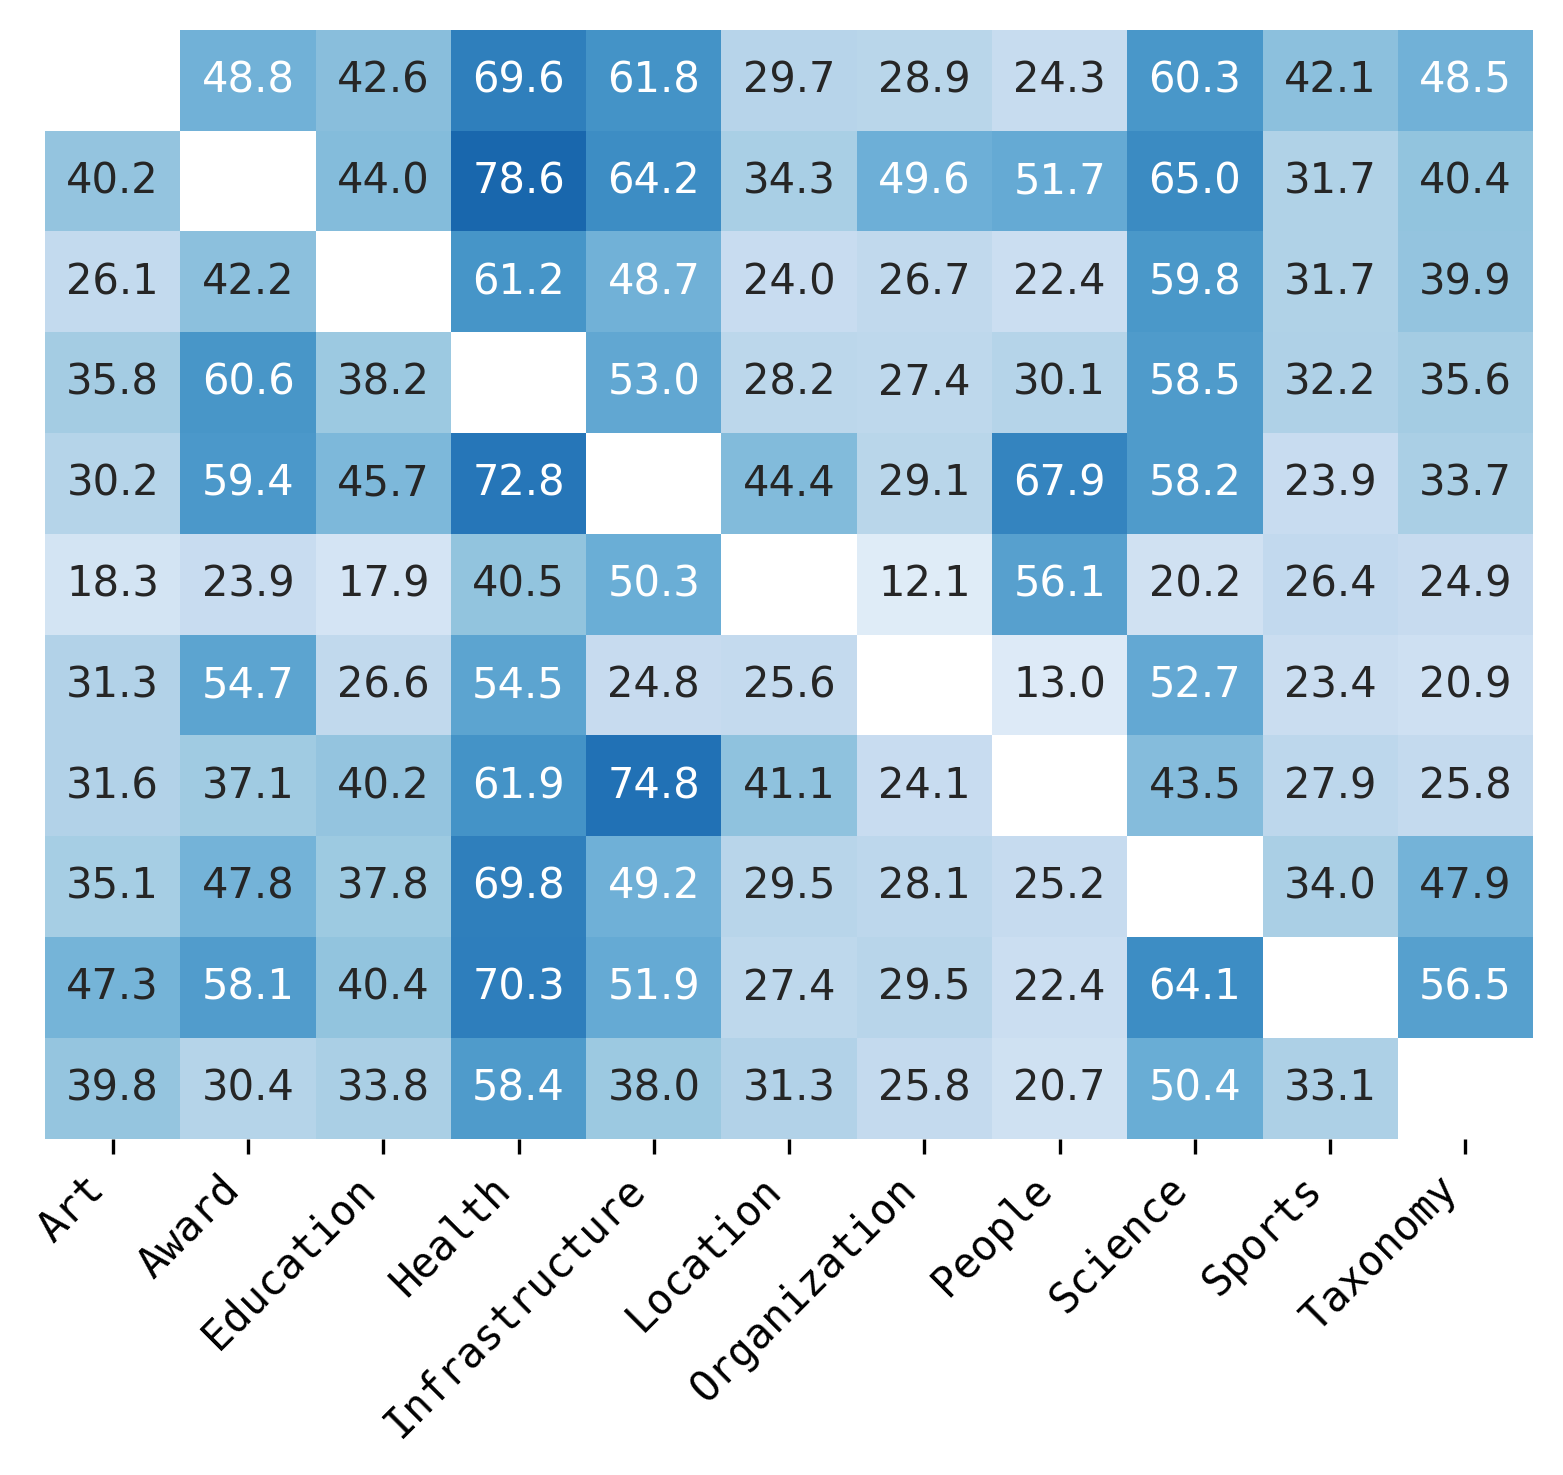}
        \vspace{-10pt}
        \caption{\OurOtherModel MRR}
    \end{subfigure}
    \hfill
    \begin{subfigure}[b]{0.31\textwidth}
        \centering
        \includegraphics[width=\linewidth,height=0.88\linewidth]{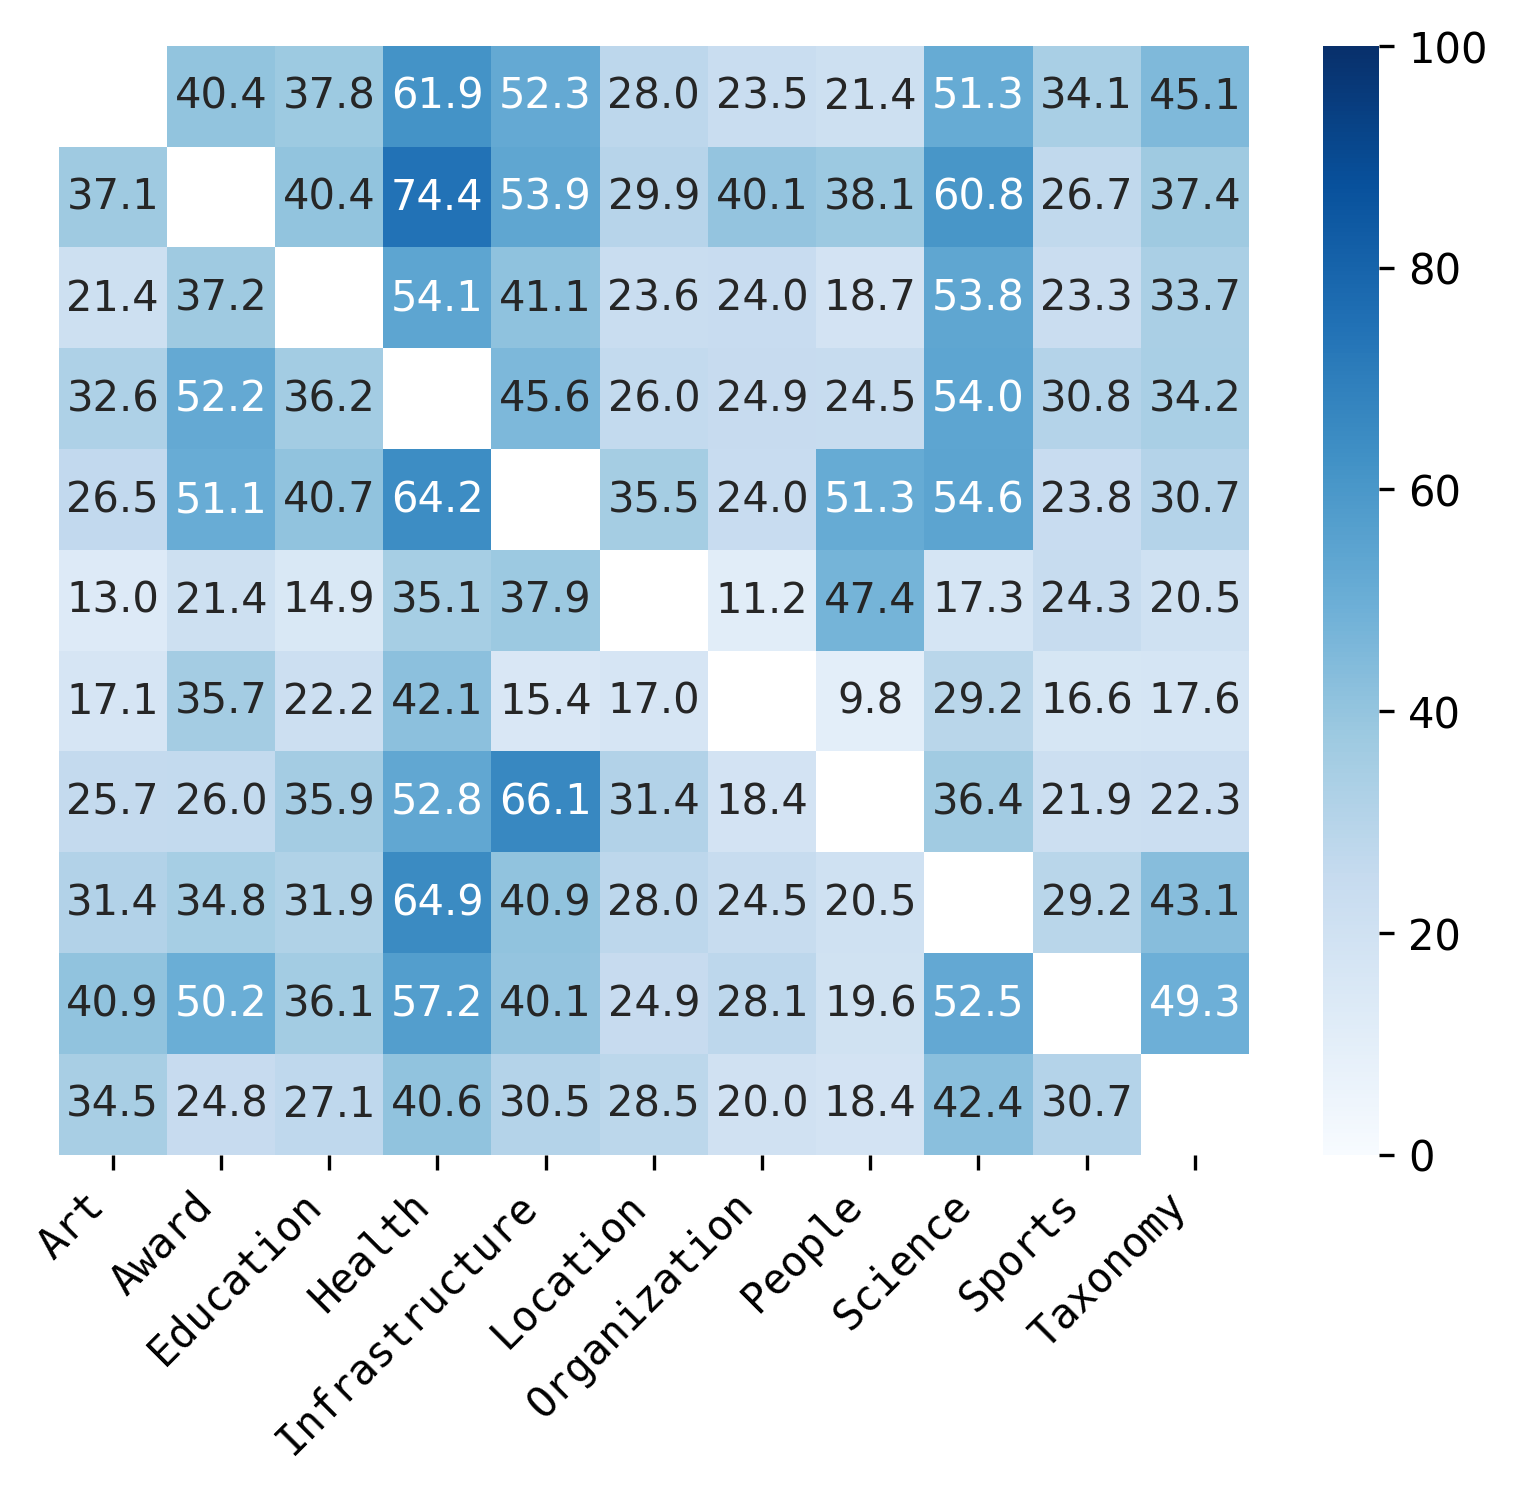}
        \vspace{-10pt}
        \caption{Original InGram MRR}
    \end{subfigure}
    \vspace{-5pt}
    \caption{{\bf Node prediction $(i, k, ?)$ performance over WikiTopics} for \update{\OurNewModel}, \OurOtherModel, and InGram~\citep{ingram}. Each row within each heatmap corresponds to a training graph, and each column within each heatmap corresponds to a test graph. A darker color means better performance. 
    \textbf{\update{\OurNewModel}, \OurOtherModel, and InGram showcase comparable performance in general, and \update{\OurNewModel} exhibits the best performance on Hits@1 in particular.}}
    %\vspace{-15pt}  % Reduce figure bottom space to the text
    \label{fig:wikitopics-node-full}
\end{figure}

\paragraph{\update{Self-supervised pre-trained zero-shot meta-learning tasks over WikiTopics to train on combined KGs with an increasing number of distinct domains and test on KGs with completely unseen test domains}}

\update{In \Cref{subsec:result-wiki}, we describe an experiment conducted with WikiTopics, focusing on the zero-shot meta-learning tasks and the effect of varying the number of training KGs. 
For this experiment, we selected 8 out of the 11 domains from \ourotherdata. 
In each experimental setup, we randomly select $1, 2, 3, \text{~or~} 4$ KGs with distinct domains for training. The model's performance is then evaluated on each of the remaining KGs for testing. We repeat this process to collect performance across various combinations, enabling us to calculate an average performance gain when training on an increasing number of KGs. 
% This approach helps us analyze how increasing the number of training topics influences test performance.
In addition, we compare the inductive performance of our \OurNewModel against the best-performing transductive model, which is trained and tested on the KG of the same domain. This approach helps us analyze whether \OurNewModel, via meta-learning on a more diverse set of training graphs, can match or even surpass the transductive model in performance.

To select the best transductive performance, we train two models: \OurNewModel and SOTA relational GNN model NBFNet~\citep{zhu2021neural} (with its original implementation) and test on graphs within the same domain, and then select the best performance from these two models as the {\em transductive SOTA} performance. We experimented with a total of 5 setups, and for each setup, we trained models with 3 different random seeds for each training combination.

\Cref{tab:meta-learning-setups}~shows training and test domains sampled for each setup, and~\Cref{tab:meta-learning-isdea-hits10,tab:meta-learning-isdea-hits5}~shows the Hits@10 and Hits@5 results on each test domain respectively. The boxplots shown in~\Cref{fig:wikitopics-relation}~are the aggregated results of~\Cref{tab:meta-learning-isdea-hits10,tab:meta-learning-isdea-hits5}. Similar to~\Cref{fig:wikitopics-relation}, we can observe that the performance of \OurNewModel consistently increases when training on more and more domains, and finally reaching or even surpassing the performance of the best-performing transductive model on certain test domains.
}

\begin{table}[h]
    \centering
    \caption{
    \update{The 5 randomly sampled setups of training and test combinations of WikiTopic domain KGs~(\Cref{tab:wikitopics-topic-desc}) that are used in our zero-shot meta-learning experiment. The $+$ between different domains denotes that the KGs corresponding to these domains are merged for model training.
    }
    }
    \resizebox{1.0\linewidth}{!}{
    \begin{tabular}{clllll}
        Setup & 1 Training Domain & 2 Training Domains & 3 Training Domains & 4 Training Domains & Test Domains \\
        \midrule
        1 & Infra  & Infra + Sci & Infra + Sci + Sport & Infra + Sci + Sport + Tax & Art, Award, Edu, Health \\
        2 & Award & Award + Edu & Award + Edu + Tax & Award + Edu + Tax + Sport & Art, Health, Infra, Sci \\
        3 & Sport & Sport + Infra & Sport + Infra + Edu & Sport + Infra + Edu + Health & Art, Award, Sci, Tax \\
        4 & Art & Art + Award & Art + Award + Health & Art + Award + Health + Infra & Edu, Sci, Sport, Tax \\
        5 & Health & Health + Sport & Health + Sport + Tax & Health + Sport + Tax + Art & Award, Edu, Infra, Sci \\
    \end{tabular}
    }
    \label{tab:meta-learning-setups}
\end{table}

\begin{table}[h]
    \centering
    \captionof{table}{
    \update{{\bf Average Relation \& Node Hits@10 performance of \OurNewModel on the Zero-Shot Meta-Learning task over \ourotherdata on each test domain.}
    We also report the performance of the best transductive model.
    {\bf \OurNewModel consistently achieves better and better performance when training on more and more domains, closing and even sometimes surpassing the best transductive model performance.} 
    }
    }
    {\subcaption{{\bf {\scriptsize Relation prediction $(i, ?, j)$ performance in \%. Higher $\uparrow$ is better.}}}
    \resizebox{\linewidth}{!}{
    \begin{tabular}{l r r r r r r r r}
        Training Scenario & Test on Art & Test on Award & Test on Edu & Test on Health & Test on Infra & Test on Sci & Test on Sport & Test on Tax \\
        \midrule
        Best Transductive & 95.37{\scriptsize $\pm 00.54$} & 99.95{\scriptsize $\pm 00.02$} & 98.33{\scriptsize $\pm 00.11$} & 99.61{\scriptsize $\pm 00.10$} & 99.83{\scriptsize $\pm 00.03$} & 99.64{\scriptsize $\pm 00.16$} & 94.40{\scriptsize $\pm 07.55$} & 87.11{\scriptsize $\pm 16.02$} \\
        \midrule
        1 training domain & 92.31{\scriptsize $\pm 02.15$} & 99.83{\scriptsize $\pm 00.18$} & 97.99{\scriptsize $\pm 00.38$} & 92.28{\scriptsize $\pm08.67$} & 96.41{\scriptsize $\pm 06.41$} & 98.50 {\scriptsize $\pm 01.23$} & 98.82{\scriptsize $\pm 00.36$} & 94.15{\scriptsize $\pm 08.49$} \\
        2 training domains & 93.61{\scriptsize $\pm 02.00$} & 99.81{\scriptsize $\pm 00.07$} & 97.66{\scriptsize $\pm 00.55$} & 98.64{\scriptsize $\pm 01.54$} & 99.25{\scriptsize $\pm 00.30$} & 98.78{\scriptsize $\pm 01.20$} & 98.43{\scriptsize $\pm 00.52$} & 96.15{\scriptsize $\pm 09.00$} \\
        3 training domains & 95.00{\scriptsize $\pm 01.75$} & 99.82{\scriptsize $\pm 00.10$} & 98.25{\scriptsize $\pm 00.22$} & 99.31{\scriptsize $\pm 00.19$} & 99.73{\scriptsize $\pm 00.22$} & 99.35{\scriptsize $\pm 00.51$} & 98.57{\scriptsize $\pm 00.35$} & 99.50{\scriptsize $\pm 00.60$} \\
        4 training domains & 96.14{\scriptsize $\pm 00.80$} & 99.84{\scriptsize $\pm 00.09$} & 98.17{\scriptsize $\pm 00.16$} & 99.25{\scriptsize $\pm 00.17$} & 99.83{\scriptsize $\pm 00.09$} & 99.55{\scriptsize $\pm 00.27$} & 99.38{\scriptsize $\pm 00.12$} & 99.71{\scriptsize $\pm 00.38$} \\
    \end{tabular}
    }
    }
    \vspace{5pt} % Make sure subtitle of next table does not come too close to bottom of last table
    {\subcaption{{\bf {\scriptsize Node prediction $(i, k, ?)$ performance in \%. Higher $\uparrow$ is better.}}}
    \resizebox{\linewidth}{!}{
    \begin{tabular}{l r r r r r r r r}
        Training Scenario & Test on Art & Test on Award & Test on Edu & Test on Health & Test on Infra & Test on Sci & Test on Sport & Test on Tax \\
        \midrule
        Best Transductive & 91.70{\scriptsize $\pm 00.54$} & 93.57{\scriptsize $\pm 01.32$} & 96.85{\scriptsize $\pm 00.18$} & 98.92{\scriptsize $\pm 00.07$} & 97.75{\scriptsize $\pm 00.17$} & 96.73{\scriptsize $\pm 00.65$} & 81.21{\scriptsize $\pm 00.10$} & 90.87{\scriptsize $\pm 05.16$} \\
        \midrule
        1 training domain & 88.55{\scriptsize $\pm 04.53$} & 85.16{\scriptsize $\pm 05.44$} & 94.75{\scriptsize $\pm 01.23$} & 89.44{\scriptsize $\pm 09.11$} & 81.81{\scriptsize $\pm 08.62$} & 95.91{\scriptsize $\pm 00.52$} & 66.93{\scriptsize $\pm 14.16$} & 82.85{\scriptsize $\pm 12.84$} \\
        2 training domains & 88.55{\scriptsize $\pm 05.52$} & 88.14{\scriptsize $\pm 01.69$} & 95.87{\scriptsize $\pm 01.37$} & 96.84{\scriptsize $\pm 01.58$} & 89.90{\scriptsize $\pm 07.05$} & 95.88{\scriptsize $\pm 01.05$} & 66.98{\scriptsize $\pm 13.73$} & 86.92{\scriptsize $\pm 11.03$} \\
        3 training domains & 92.26{\scriptsize $\pm 00.71$} & 87.93{\scriptsize $\pm 01.23$} & 96.85{\scriptsize $\pm 00.53$} & 97.27{\scriptsize $\pm 01.22$} & 87.63{\scriptsize $\pm 06.73$} & 96.33{\scriptsize $\pm 00.54$} & 77.19{\scriptsize $\pm 05.87$} & 93.67{\scriptsize $\pm 01.25$} \\
        4 training domains & 90.74{\scriptsize $\pm 02.54$} & 89.47{\scriptsize $\pm 00.82$} & 97.00{\scriptsize $\pm 00.36$} & 97.82{\scriptsize $\pm 00.48$} & 94.01{\scriptsize $\pm 01.82$} & 96.19{\scriptsize $\pm 00.28$} & 80.69{\scriptsize $\pm 00.29$} & 92.89{\scriptsize $\pm 01.19$} \\
    \end{tabular}
    }
    }
    \label{tab:meta-learning-isdea-hits10}
\end{table}

\begin{table}[h]
    \centering
    \captionof{table}{
    \update{{\bf Average Relation \& Node Hits@5 performance of \OurNewModel on the Zero-Shot Meta-Learning task over \ourotherdata on each test domain.}
    We also report the performance of the best transductive model.
    {\bf \OurNewModel consistently achieves better and better performance when training on more and more domains, closing and even sometimes surpassing the best transductive model performance.} 
    }
    }
    {\subcaption{{\bf {\scriptsize Relation prediction $(i, ?, j)$ performance in \%. Higher $\uparrow$ is better.}}}
    \resizebox{\linewidth}{!}{
    \begin{tabular}{l r r r r r r r r}
        Training Scenario & Test on Art & Test on Award & Test on Edu & Test on Health & Test on Infra & Test on Sci & Test on Sport & Test on Tax \\
        \midrule
        Best Transductive & 83.80{\scriptsize $\pm 01.92$} & 97.32{\scriptsize $\pm 00.14$} & 94.31{\scriptsize $\pm 00.27$} & 98.43{\scriptsize $\pm 00.26$} & 98.32{\scriptsize $\pm 00.43$} & 99.57{\scriptsize $\pm 00.16$} & 90.60{\scriptsize $\pm 05.84$} & 87.11{\scriptsize $\pm 16.02$} \\
        \midrule
        1 training domain & 79.93{\scriptsize $\pm 03.42$} & 96.08{\scriptsize $\pm 01.68$} & 92.83{\scriptsize $\pm 00.99$} & 88.99{\scriptsize $\pm 08.63$} & 92.02{\scriptsize $\pm 06.72$} & 98.45{\scriptsize $\pm 01.29$} & 88.40{\scriptsize $\pm 01.23$} & 94.14{\scriptsize $\pm 08.48$} \\
        2 training domains & 82.78{\scriptsize $\pm 03.27$} & 96.19{\scriptsize $\pm 00.51$} & 93.33{\scriptsize $\pm 01.07$} & 96.48{\scriptsize $\pm 01.73$} & 95.93{\scriptsize $\pm 00.88$} & 98.72{\scriptsize $\pm 01.18$} & 89.79{\scriptsize $\pm 05.11$} & 96.12{\scriptsize $\pm 08.98$} \\
        3 training domains & 84.46{\scriptsize $\pm 03.01$} & 96.08{\scriptsize $\pm 00.39$} & 92.66{\scriptsize $\pm 01.32$} & 96.92{\scriptsize $\pm 00.22$} & 96.28{\scriptsize $\pm 00.72$} & 99.30{\scriptsize $\pm 00.49$} & 86.47{\scriptsize $\pm 01.64$} & 99.48{\scriptsize $\pm 00.59$} \\
        4 training domains & 85.44{\scriptsize $\pm 02.71$} & 96.20{\scriptsize $\pm 00.40$} & 92.74{\scriptsize $\pm 01.20$} & 96.65{\scriptsize $\pm 00.57$} & 97.33{\scriptsize $\pm 00.71$} & 99.47{\scriptsize $\pm 00.26$} & 92.25{\scriptsize $\pm 02.16$} & 99.69{\scriptsize $\pm 00.37$} \\
    \end{tabular}
    }
    }
    \vspace{5pt} % Make sure subtitle of next table does not come too close to bottom of last table
    {\subcaption{{\bf {\scriptsize Node prediction $(i, k, ?)$ performance in \%. Higher $\uparrow$ is better.}}}
    \resizebox{\linewidth}{!}{
    \begin{tabular}{l r r r r r r r r}
        Training Scenario & Test on Art & Test on Award & Test on Edu & Test on Health & Test on Infra & Test on Sci & Test on Sport & Test on Tax \\
        \midrule
        Best Transductive & 85.01{\scriptsize $\pm 00.89$} & 75.54{\scriptsize $\pm 03.10$} & 86.10{\scriptsize $\pm 00.27$} & 95.95{\scriptsize $\pm 00.30$} & 96.24{\scriptsize $\pm 00.11$} & 95.15{\scriptsize $\pm 00.29$} & 67.30{\scriptsize $\pm 00.08$} & 85.04{\scriptsize $\pm 06.03$} \\
        \midrule
        1 training domain & 80.20{\scriptsize $\pm 05.57$} & 60.59{\scriptsize $\pm 09.59$} & 77.25{\scriptsize $\pm 06.02$} & 81.27{\scriptsize $\pm 09.32$} & 73.61{\scriptsize $\pm 08.63$} & 94.30{\scriptsize $\pm 00.71$} & 52.22{\scriptsize $\pm 14.46$} & 77.75{\scriptsize $\pm 12.63$} \\
        2 training domains & 80.55{\scriptsize $\pm 05.80$} & 65.41{\scriptsize $\pm 03.45$} & 83.19{\scriptsize $\pm 02.46$} & 90.89{\scriptsize $\pm 02.09$} & 84.92{\scriptsize $\pm 08.23$} & 94.36{\scriptsize $\pm 01.03$} & 52.88{\scriptsize $\pm 14.05$} & 81.17{\scriptsize $\pm 10.75$} \\
        3 training domains & 84.32{\scriptsize $\pm 01.34$} & 65.56{\scriptsize $\pm 02.17$} & 84.03{\scriptsize $\pm 01.60$} & 92.20{\scriptsize $\pm 01.14$} & 81.93{\scriptsize $\pm 07.45$} & 94.97{\scriptsize $\pm 00.53$} & 62.13{\scriptsize $\pm 06.85$} & 87.91{\scriptsize $\pm 00.88$} \\
        4 training domains & 83.29{\scriptsize $\pm 02.56$} & 68.97{\scriptsize $\pm 01.44$} & 83.93{\scriptsize $\pm 01.11$} & 91.94{\scriptsize $\pm 02.09$} & 88.38{\scriptsize $\pm 04.51$} & 94.64{\scriptsize $\pm 00.43$} & 66.12{\scriptsize $\pm 00.17$} & 86.91{\scriptsize $\pm 01.09$} \\
    \end{tabular}
    }
    }
    \label{tab:meta-learning-isdea-hits5}
\end{table}

\subsubsection{\OurTask over datasets from InGram (Lee et al., 2023)}

\citet{ingram} proposed the NL-$k$, WK-$k$, and FB-$k$ benchmarks originally used to evaluate InGram's performance of reasoning over new nodes and new relation types at test time, where $k \in \{ 25, 50, 75, 100 \}$ means that, in the test graphs, approximately $k\%$ of triplets have unseen relations. For example, the test graph of WK-100 does not contain any training relations and thus induces a \ourtask task. Hence, we run our models (\OurModel and \OurOtherModel) against InGram on these benchmarks with results shown in~\Cref{tab:ingram-dataset}. We note that, however, due to the different experimental settings (as we discuss next), our results reported in~\Cref{tab:ingram-dataset} are not directly comparable to those reported in~\citet{ingram}, even though they are experimented on essentially the same datasets.

\paragraph{Difference to the original data split and evaluation in InGram~\citep{ingram}:} Different from~\citet{ingram}, which uses part of the test graph as the validation set to conduct model hyperparameter search, {\em our experiments consider a harder setting where the relations in test are not observed in the validation data}. Hence, to modify the NL-$k$, WK-$k$, and FB-$k$ datasets to our setting, we discard the original validation set and instead split the original training set into a new set of training and validation triplets with a ratio of 9:1. During training, the models perform self-supervised masking over the training set of triplets to create the training-time observable triplets and training-time target triplets. During validation, the entire set of the new training triplets is taken as the validation-time observable triplets, and the new validation triplets are the target triplets to predict. In addition, \citet{ingram} evaluate their model's node prediction performance against \textit{all} nodes in the graph. For efficiency reasons, we evaluate the model performance by sampling without replacement 50 negative nodes for the node prediction task and sampling with replacement 50 negative relation types for the relation prediction task.

\Cref{tab:ingram-dataset} shows the results, where we can see that \OurModel outperforms InGram on most datasets on the relation prediction task and has smaller standard deviation in general, and \OurOtherModel consistently outperforms InGram on all datasets for both relation prediction and node prediction tasks. Importantly, in the dataset FB-100 which follows our \ourtask setting with completely new nodes and new relation types in the test with the largest number of training and test relations ($134$ in train and $77$ in test)~\citep{ingram}, \OurModel achieves significant better results in the relation perdiction task, showcasing its ability for \ourtask.

\begin{table}[t]
% \vspace{-25pt}   % Reduce table head space to the top of the page
\centering
\captionof{table}{
{\bf Relation \& Node Hits@10 performance on \OurTask over NL-$k$, WK-$k$, and FB-$k$ of~\citet{ingram}.} We report standard deviations over 5 runs. %
A higher value means better \ourtask performance. 
The best values are shown in bold font, while the second-best values are underlined. 
{\bf \OurModel outperforms InGram on most datasets on the relation prediction task, and \OurOtherModel consistently outperforms InGram on all datasets for both relation prediction and node prediction tasks.}
}
%\vspace{5pt}
{
\subcaption{{\bf {\scriptsize Performance in \% on WK-$k$ datasets. Higher $\uparrow$ is better.}}}
\resizebox{1.0\linewidth}{!}{
\begin{tabular}{l r r r r c r r r r}
    & \multicolumn{4}{c}{Relation prediction $(i, ?, j)$} & & \multicolumn{4}{c}{Node prediction $(i, k, ?)$} \\
    
    \cmidrule{2-5} \cmidrule{7-10} 
    Models & WK-25 & WK-50 & WK-75 & WK-100 & & WK-25 & WK-50 & WK-75 & WK-100 \\
    \midrule
    
    InGram & 58.76{\scriptsize $\pm 13.91$} & {84.01}{\scriptsize $\pm 03.30$} & 80.19{\scriptsize $\pm 04.19$} & 58.20{\scriptsize $\pm 11.13$} & & {76.99}{\scriptsize $\pm 07.72$} & 70.93{\scriptsize $\pm 02.38$} & {78.85}{\scriptsize $\pm 04.65$} & 66.29{\scriptsize $\pm 03.70$} \\
    \midrule
    
    \OurOtherModel (Ours) & \underline{81.06}{\scriptsize $\pm 22.31$} & \textbf{94.85}{\scriptsize $\pm 00.85$} & \textbf{95.84}{\scriptsize $\pm 01.54$} & \underline{81.83}{\scriptsize $\pm 10.10$} & & \underline{87.91}{\scriptsize $\pm 05.68$} & \underline{82.58}{\scriptsize $\pm 01.70$} & \underline{89.10}{\scriptsize $\pm 02.15$} & \underline{79.69}{\scriptsize $\pm 03.07$} \\
    
    % \OurModel (Ours) & \underline{79.49}{\scriptsize $\pm 06.88$} & {81.25}{\scriptsize $\pm 07.02$} & \underline{84.92}{\scriptsize $\pm 06.86$} & \underline{79.70}{\scriptsize $\pm 07.68$} & & 58.28{\scriptsize $\pm 23.68$} & \underline{73.24}{\scriptsize $\pm 00.57$} & 76.19{\scriptsize $\pm 01.04$} & \underline{71.76}{\scriptsize $\pm 01.85$} \\

    \update{\OurNewModel (Ours)} & \update{\textbf{96.25}{\scriptsize $\pm 00.86$}} & \update{\underline{93.10}{\scriptsize $\pm 02.55$}} & \update{\underline{95.66}{\scriptsize $\pm 00.82$}} & \update{\textbf{95.00}{\scriptsize $\pm 00.15$}} & & \update{\textbf{94.41}{\scriptsize $\pm 01.61$}} & \update{\textbf{90.34}{\scriptsize $\pm 01.71$}} & \update{\textbf{91.98}{\scriptsize $\pm 01.61$}} & \update{\textbf{91.22}{\scriptsize $\pm 00.45$}}
\end{tabular}
\label{tab:ingram-dataset-WK}
}
\vspace{5pt}
\subcaption{{\bf {\scriptsize Performance in \% on FB-$k$ datasets. Higher $\uparrow$ is better.}}}
\resizebox{1.0\linewidth}{!}{
\begin{tabular}{l r r r r c r r r r}
    & \multicolumn{4}{c}{Relation prediction $(i, ?, j)$} & & \multicolumn{4}{c}{Node prediction $(i, k, ?)$} \\
    
    \cmidrule{2-5} \cmidrule{7-10} 
    Models & FB-25 & FB-50 & FB-75 & FB-100 & & FB-25 & FB-50 & FB-75 & FB-100 \\
    \midrule
    
    InGram & 68.26{\scriptsize $\pm 08.27$} & 50.41{\scriptsize $\pm 08.79$} & 79.51{\scriptsize $\pm 02.69$} & 40.46{\scriptsize $\pm 12.21$} & & \underline{86.79}{\scriptsize $\pm 00.70$} & {73.32}{\scriptsize $\pm 06.64$} & {86.57}{\scriptsize $\pm 00.69$} & 71.72{\scriptsize $\pm 06.93$} \\
    \midrule
    
    \OurOtherModel (Ours) & \underline{82.89}{\scriptsize $\pm 03.58$} & \underline{76.65}{\scriptsize $\pm 04.05$} & \underline{89.70}{\scriptsize $\pm 01.14$} & \underline{46.88}{\scriptsize $\pm 15.76$} & & \textbf{92.39}{\scriptsize $\pm 00.30$} & \underline{81.08}{\scriptsize $\pm 06.98$} & \textbf{92.14}{\scriptsize $\pm 00.43$} & \underline{77.54}{\scriptsize $\pm 06.36$} \\
    
    % \OurModel (Ours) & \textbf{83.63}{\scriptsize $\pm 05.66$} & \textbf{78.70}{\scriptsize $\pm 05.90$} & \underline{81.27}{\scriptsize $\pm 07.24$} & \textbf{85.41}{\scriptsize $\pm 04.43$} & & 75.93{\scriptsize $\pm 00.49$} & 69.90{\scriptsize $\pm 00.81$} & 73.45{\scriptsize $\pm 01.17$} & \textbf{79.70}{\scriptsize $\pm 00.81$} \\

    \update{\OurNewModel (Ours)} & \update{\textbf{96.68}{\scriptsize $\pm 00.15$}} & \update{\textbf{93.55}{\scriptsize $\pm 00.77$}} & \update{\textbf{96.86}{\scriptsize $\pm 00.58$}} & \update{\textbf{97.55}{\scriptsize $\pm 00.33$}} & & \update{85.01{\scriptsize $\pm 00.92$}} & \update{\textbf{84.40}{\scriptsize $\pm 00.38$}} & \update{\underline{86.62}{\scriptsize $\pm 00.31$}} & \update{\textbf{91.28}{\scriptsize $\pm 00.19$}}
\end{tabular}
\label{tab:ingram-dataset-FB}
}
\vspace{5pt}
\subcaption{{\bf {\scriptsize Performance in \% on NL-$k$ datasets. Higher $\uparrow$ is better.}}}
\resizebox{1.0\linewidth}{!}{
\begin{tabular}{l r r r r c r r r r}
    & \multicolumn{4}{c}{Relation prediction $(i, ?, j)$} & & \multicolumn{4}{c}{Node prediction $(i, k, ?)$} \\
    
    \cmidrule{2-5} \cmidrule{7-10} 
    Models & NL-25 & NL-50 & NL-75 & NL-100 & & NL-25 & NL-50 & NL-75 & NL-100 \\
    \midrule
    
    InGram & 64.54{\scriptsize $\pm 16.86$} & 64.54{\scriptsize $\pm 12.56$} & {80.16}{\scriptsize $\pm 04.43$} & 70.84{\scriptsize $\pm 08.52$} & & \underline{89.95}{\scriptsize $\pm 02.01$} & \underline{92.74}{\scriptsize $\pm 00.52$} & \underline{95.40}{\scriptsize $\pm 01.38$} & {88.20}{\scriptsize $\pm 01.92$} \\
    \midrule
    
    \OurOtherModel (Ours) & \underline{83.58}{\scriptsize $\pm 17.57$} & \underline{91.32}{\scriptsize $\pm 05.60$} & \underline{96.01}{\scriptsize $\pm 01.23$} & \underline{87.52}{\scriptsize $\pm 10.39$} & & \textbf{95.03}{\scriptsize $\pm 00.32$} & \textbf{96.02}{\scriptsize $\pm 00.34$} & \textbf{97.94}{\scriptsize $\pm 00.34$} & \textbf{93.80}{\scriptsize $\pm 01.38$} \\
    
    % \OurModel (Ours) & \underline{69.49}{\scriptsize $\pm 05.71$} & \underline{76.23}{\scriptsize $\pm 06.92$} & 76.03{\scriptsize $\pm 03.31$} & \underline{80.84}{\scriptsize $\pm 07.35$} & & 73.74{\scriptsize $\pm 03.35$} & 75.76{\scriptsize $\pm 03.52$} & 77.27{\scriptsize $\pm 03.80$} & 72.81{\scriptsize $\pm 04.41$} \\
    \update{\OurNewModel (Ours)} & \update{\textbf{92.04}{\scriptsize $\pm 02.67$}} & \update{\textbf{93.78}{\scriptsize $\pm 01.37$}} & \update{\textbf{96.57}{\scriptsize $\pm 01.85$}} & \update{\textbf{99.72}{\scriptsize $\pm 00.15$}} & & \update{{82.20}{\scriptsize $\pm 04.36$}} & \update{83.35{\scriptsize $\pm 00.40$}} & \update{90.94{\scriptsize $\pm 00.85$}} & \update{\underline{90.06}{\scriptsize $\pm 00.49$}}
\end{tabular}
\label{tab:ingram-dataset-NL}
}
% \vspace{-15pt}  % Reduce table bottom space to the text
}
\label{tab:ingram-dataset}
\end{table}

\subsubsection{A Synthetic Case Study for \OurModel}
\label{subsec:limit}

\begin{figure}[ht]
\centering
\includegraphics[width=.5\linewidth]{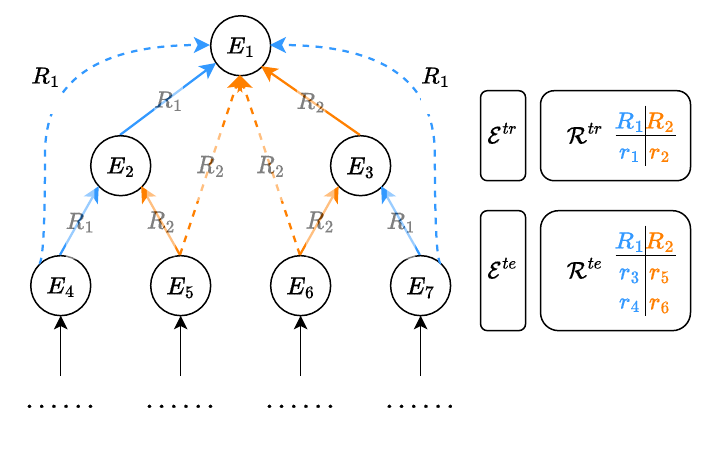}
\caption{
{\bf Synthetic Example of FD-2:} Training and test has their own node and relation type sets: $\cV\suptr \cap \cV\supte = \emptyset$ and $\cR\suptr \cap \cR\supte = \emptyset$.}
\label{fig:example-fd2}
\end{figure}

To further understand the expressive power and limitations of our proposed sturctural double equivariant model \OurModel, we create {\bf FD-2} to empirically justify the expressivity of our proposal on tasks over both new nodes and new relation types. On FD-2, training has 127 nodes and 2 relations, while test has 254 nodes and 4 relations (more nodes and more relations).

FD-2 is constructed by only a single rule, $\left( E_1, R_1, E_3 \right) \land \left( E_3, R_2, E_2 \right) \Rightarrow \left( E_1, R_1, E_3 \right)$ where $E_1, E_2, E_3$ and $R_1, R_2$ are all variables.
As illustrated in \Cref{fig:example-fd2}, The training data has only two relation types $\{r_1, r_2\}$, while test data has four relation types $\{r_3, r_4, r_5, r_6\}$ which are all different from training relations.
For all relation types, only $r_1, r_3, r_4$ can be used for $R_1$ assignments, and only $r_2, r_5, r_6$ can be use for $R_2$ assignments.
Besides, training and test also have distinct node sets.

Each graph (training or test) is consisted by one or more tree-like structures as left side of \Cref{fig:example-fd2}.
In each tree-like structure, all solid edges are used as observations, and will form a complete binary tree; 
while all dashed edges are used as training, validation or test samples which are built by applying the only rule over all observed edges.
In training, we have only one tree-like structure; while in test, we have two disconnected tree-like structures. A more detailed generation algorithm for a graph given depths of all tree-like structures is provided in \Cref{alg:synth-fd2}.

Since the structure of FD-2 does not satisfy the requirement of the spanning tree algorithm used in InGram~\citep{ingram}, we are not able to apply InGram and \OurOtherModel on FD-2. So we provide the results on FD-2 in \Cref{tab:exp-fd2-relation} with all remaining baselines and \OurModel. We can see that \OurModel clearly perform better than other baselines, especially in the relation prediction task, and shows capability to perform accurately on the \ourtask over both new nodes and new relation types, while methods like NBFNet and RMPI are not able to correctly perdict this task, even for node prediction.

\begin{table}[t!]
\centering
\centering
\captionof{table}{
{\bf Relation \& Node performance on \OurTask over FD2.} We report standard deviations over 5 runs. %
A higher value means better \ourtask performance. 
The best values are shown in bold font, while the second-best values are underlined. 
\OurModel  consistently achieve better results than the baselines, especially in the Relation perdiction task. NA* due to the fact that FD2 does not satisfy the spanning tree algorithm used in InGram~\citep{ingram}.
}
\resizebox{\linewidth}{!}{
\begin{tabular}{l r r r r c r r r r}
    & \multicolumn{4}{c}{Relation prediction $(i, ?, j)$} & & \multicolumn{4}{c}{Node prediction $(i, k, ?)$} \\
    
    \cmidrule{2-5} \cmidrule{7-10} 
    Models & MRR & Hits@1 & Hits@2 & Hits@4 & & MRR & Hits@1 & Hits@2 & Hits@4\\
    \midrule
    GAT & 7.61{\scriptsize $\pm 00.71$} & 0.77{\scriptsize $\pm 00.39$} & 2.78{\scriptsize $\pm 00.80$} & 5.85{\scriptsize $\pm 00.95$} & & 84.62{\scriptsize $\pm 02.64$} & 71.61{\scriptsize $\pm 04.94$} & \underline{93.51}{\scriptsize $\pm 01.03$} & 99.72{\scriptsize $\pm 00.27$}  \\
    GIN & 8.44{\scriptsize $\pm 00.40$} & 1.29{\scriptsize $\pm 00.37$} & 3.51{\scriptsize $\pm 00.58$} & \underline{7.18}{\scriptsize $\pm 01.01$} & & 73.99{\scriptsize $\pm 09.60$} & 65.73{\scriptsize $\pm 06.58$} & 76.69{\scriptsize $\pm 12.44$} & 81.45{\scriptsize $\pm 15.80$} \\
    GraphConv & 7.88{\scriptsize $\pm 00.45$} & 0.81{\scriptsize $\pm 00.29$} & 2.62{\scriptsize $\pm 00.61$} & 6.98{\scriptsize $\pm 01.09$} & & \underline{85.95}{\scriptsize $\pm 00.77$} & \underline{74.52}{\scriptsize $\pm 01.81$} & 92.66{\scriptsize $\pm 01.02$} & \textbf{99.84}{\scriptsize $\pm 00.15$}\\
    RMPI & \underline{9.09}{\scriptsize $\pm 03.18$} & \underline{1.94}{\scriptsize $\pm 01.88$} & \underline{3.95}{\scriptsize $\pm 04.43$} & 7.10{\scriptsize $\pm 05.58$} & & 21.16{\scriptsize $\pm 05.85$} & 9.84{\scriptsize $\pm 05.04$} & 16.74{\scriptsize $\pm 06.50$} & 27.98{\scriptsize $\pm 09.96$} \\
    NBFNet & 6.39{\scriptsize $\pm 02.19$} & 1.50{\scriptsize $\pm 02.49$} &1.79{\scriptsize $\pm 02.39$} & 2.91{\scriptsize $\pm 02.22$}&  & 21.95{\scriptsize $\pm 04.14$} & 14.44{\scriptsize $\pm 04.34$}  & 18.61{\scriptsize $\pm 04.29$} & 26.47{\scriptsize $\pm 04.24$} \\
    InGram &  N/A* & N/A* &N/A* & N/A*&  &  N/A* & N/A* &N/A* & N/A*\\
    \midrule
    
    \OurOtherModel (Ours) & N/A* & N/A* &N/A* & N/A*&  &  N/A* & N/A* &N/A* & N/A* \\
    
    \OurModel (Ours) & \textbf{44.39}{\scriptsize $\pm 12.17$} & \textbf{32.82}{\scriptsize $\pm 12.69$} & \textbf{38.71}{\scriptsize $\pm 13.60$} & \textbf{50.73}{\scriptsize $\pm 14.04$} & & \textbf{90.98}{\scriptsize $\pm 03.55$} & \textbf{83.59}{\scriptsize $\pm 06.22$} & \textbf{95.69}{\scriptsize $\pm 02.34$} & \underline{99.72}{\scriptsize $\pm 00.27$} \\ \\
    % \update{\OurNewModel (Ours)} & 
\end{tabular}
}
\vspace{5pt}
%\vspace{-20pt}
\label{tab:exp-fd2-relation}
\end{table}

% \begin{table}[t!]
% \centering
% %
% \resizebox{0.6\linewidth}{!}{
% \begin{tabular}{l|cccc}
%     \hline
%     \multirow{2}{*}{Model} & \multicolumn{4}{c}{FD-2} \\
%     \cline{2-5}
%     & MRR$\uparrow$ & Hits@1$\uparrow$ & Hits@2$\uparrow$ & Hits@4$\uparrow$ \\
%     \hline
% GAT & 11.80 & ~~1.80 & ~~5.20 & 12.10 \\
% GIN & 12.30 & ~~1.60 & ~~4.80 & 11.10 \\
% GraphConv & 13.40 & ~~2.60 & ~~5.60 & 14.50 \\
% NBFNet* & 13.50 & ~~4.70 & ~~8.10 & 15.70 \\
% \hline
% ISDEA & \textbf{68.30} & \textbf{52.40} & \textbf{68.10} & \textbf{87.90} \\
% \hline
% \end{tabular}
% }
% \vspace{5pt}
% \caption{\textbf{Node Inductive \ourtask over both new nodes and new relation types performance on Family Diagrams 2.} Existing baselines clearly struggle to perform the task.\yangze{change description}}
% %\vspace{-20pt}
% \label{tab:exp-fd2-node}
% \end{table}

%\vspace{-20pt}
\begin{algorithm}
\caption{{\bf Synthesis Algorithm for FD-2.} This is triplet generation code for a single graph (either training and test). It will provide observation and query triplets. For training, query triplets are further divided into training and validation triplets; For test, query triplets directly become test triplets.}
\label{alg:synth-fd2}
\begin{algorithmic}[1]
\Require Tree depth $\{D_1, \ldots, D_M\}$, Node Labeling ``$\text{Names}^\text{nd}$'', Relation Type Labeling ``$\text{Names}^\text{rl}$''.
\Ensure Observation triplets $\cS$, Query triplets $\cQ$
\State $\cS = \emptyset$
\State $\cQ = \emptyset$
\State $n \leftarrow 0$
\For{$m \leftarrow 1, \ldots, M$}
    \For{$d \leftarrow 1, \ldots, D_m$}
        \For{$v \leftarrow 2^d - 1, \ldots, 2^{d + 1} - 2$}
            \State $u_1 \leftarrow \lceil \sfrac{(v - 2)}{2} \rceil$
            \State $u_2 \leftarrow \lceil \sfrac{(u_1 - 2)}{2} \rceil$
            \If{$v \text{ mod } 2 = 0$}
                \Comment{For relation type variable $R_2$.}
                \If{$u_1 \geq 0$}
                    \State $\cS$.add$\big(\,(\text{Names}^\text{nd}[n + v], \text{Names}^\text{rl}[2m - 1], \text{Names}^\text{nd}[n + u_1])\,\big)$
                \EndIf
                \If{$u_2 \geq 0$}
                    \State $\cQ$.add$\big(\,(\text{Names}^\text{nd}[n + v], \text{Names}^\text{rl}[2m - 1], \text{Names}^\text{nd}[n + u_2])\,\big)$
                \EndIf
            \Else
                \Comment{For relation type variable $R_1$.}
                \If{$u_1 \geq 0$}
                    \State $\cS$.add$\big(\,(\text{Names}^\text{nd}[n + v], \text{Names}^\text{rl}[2m - 2], \text{Names}^\text{nd}[n + u_1])\,\big)$
                \EndIf
                \If{$u_2 \geq 0$}
                    \State $\cQ$.add$\big(\,(\text{Names}^\text{nd}[n + v], \text{Names}^\text{rl}[2m - 2], \text{Names}^\text{nd}[n + u_2])\,\big)$
                \EndIf
            \EndIf
        \EndFor
        \State $n \leftarrow n + 2^d$
    \EndFor
\EndFor
\end{algorithmic}
\end{algorithm}
%\vspace{-20pt}

\subsubsection{Expressivity Limitation Case Study with FD-2 for \OurModel}
\label{subsubsec:limit}
We now provide a FD-2 variant where we show that \ourequiv representation is not expressive enough to solve a specific task. It is a simple 2-depth tree structure as shown in \Cref{fig:example-limit}.
We denote node representations given by arbitrary \ourequiv representation as $H_{v, r}$ where $v \in [1, 7]$ and $r \in [1, 4]$. We can easily notice that $e_4$ and $e_7$ are symmetric, $e_5$ and $e_6$ are symmetric (simply flipping blue and orange colors), thus we will expect $H_{4, 1} = H_{7, 2}, H_{4, 2} = H_{7, 1}, H_{5, 1} = H_{6, 2}, H_{5, 2} = H_{6, 1}$.

\begin{figure}[h]
\centering
\includegraphics[width=0.3\linewidth]{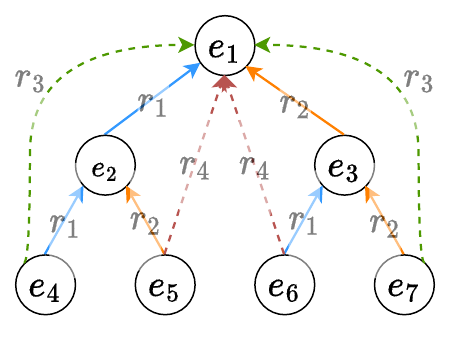}
\caption{
{\bf Expressivity Limitation:} Relation $r_1$ and $r_2$ are always observed, while $r_3$ and $r_4$ are always querying. $r_3$ implies that relation types on the path are same, while $r_4$ implies that relation types on the path are different..}
\label{fig:example-limit}
\end{figure}

Since there is no $r_3$ and $r_4$ in observation, they are freely exchangeable with each other, thus we will also expect 
\begin{equation*}
\begin{gathered}
H_{1, 3} = H_{1, 4}, \\
H_{4, 3} = H_{4, 4} = H_{7, 4} = H_{7, 3}, \\
H_{5, 3} = H_{5, 4} = H_{6, 4} = H_{6, 3}. \\
\end{gathered}
\end{equation*}

After getting all those representations, we can now focus on querying triplet representations (dashed green and red) by concatenating head and tail node representations w.r.t. relation types:
\begin{equation*}
\begin{gathered}
\trifunc{\Gamma} \left( \left( e_1, r_4, e_4 \right), \adj \right) = H_{1, 4} \mathbin\Vert H_{4, 4}, \\
\trifunc{\Gamma} \left( \left( e_1, r_3, e_5 \right), \adj \right) = H_{1, 3} \mathbin\Vert H_{5, 3}, \\
\trifunc{\Gamma} \left( \left( e_1, r_3, e_6 \right), \adj \right) = H_{1, 3} \mathbin\Vert H_{6, 3} ,\\
\trifunc{\Gamma} \left( \left( e_1, r_4, e_7 \right), \adj \right) = H_{1, 4} \mathbin\Vert H_{7, 4}. \\
\end{gathered}
\end{equation*}

We can notice that
\begin{equation*}
\begin{gathered}
\overbrace{H_{1, 4} \mathbin\Vert H_{4, 4}}^{\trifunc{\Gamma} \left( \left( e_1, r_4, e_4 \right), \adj \right)} = \overbrace{H_{1, 4} \mathbin\Vert H_{7, 4}}^{\trifunc{\Gamma} \left( \left( e_1, r_4, e_7 \right), \adj \right)}
= \overbrace{H_{1, 3} \mathbin\Vert H_{7, 3}}^{\trifunc{\Gamma} \left( \left( e_1, r_3, e_7 \right), \adj \right)} = \overbrace{H_{1, 3} \mathbin\Vert H_{4, 3}}^{\trifunc{\Gamma} \left( \left( e_1, r_3, e_4 \right), \adj \right)}, \\
\overbrace{H_{1, 4} \mathbin\Vert H_{5, 4}}^{\trifunc{\Gamma} \left( \left( e_1, r_4, e_5 \right), \adj \right)} = \overbrace{H_{1, 4} \mathbin\Vert H_{6, 4}}^{\trifunc{\Gamma} \left( \left( e_1, r_4, e_6 \right), \adj \right)}
= \overbrace{H_{1, 3} \mathbin\Vert H_{6, 3}}^{\trifunc{\Gamma} \left( \left( e_1, r_3, e_6 \right), \adj \right)} = \overbrace{H_{1, 3} \mathbin\Vert H_{5, 3}}^{\trifunc{\Gamma} \left( \left( e_1, r_3, e_5 \right), \adj \right)}. \\
\end{gathered}
\end{equation*}

Suppose the score of $\left( e_u, r_c, e_v \right)$ utilizing such representation is $s_{u, c, v}$, we will have
\begin{equation*}
\begin{gathered}
s_{4, 4, 1} = s_{7, 4, 1} = s_{7, 3, 1} = s_{4, 3, 1}, \\
s_{5, 4, 1} = s_{6, 4, 1} = s_{6, 3, 1} = s_{5, 3, 1}. \\
\end{gathered}
\end{equation*}

If a model can distinguish $r_3$ and $r_4$, it should at least rank node $e_7$ higher than $e_6$ given head node $e_1$ and relation $r_3$ since this is a positive triplet in training.
Then, we will have $s_{7, 3, 1} > s_{6, 3, 1}$, since we already knew that $s_{7, 3, 1} = s_{7, 4, 1}, s_{6, 3, 1} = s_{6, 4, 1}$, we will also have $s_{7, 4, 1} > s_{6, 4, 1}$.
This means that we rank node $e_7$ higher than node $e_6$  given head node $e_1$ and relation $r_4$, however, this is incorrect since $\left( e_7, r_4, e_1) \right)$ is negative while $\left( e_6, r_4, e_1 \right)$ is positive.
In summary, if we use \ourequiv representation for triplet scoring in this specific example, there is no way for it to correctly rank $r_3$ and $r_4$ in the same time.
This shows that \ourequiv representation (even the most expressive) can face challenges for \ourtask on \ourgraph.

\subsection{Complexity Analysis for \OurModel and \update{\OurNewModel}}
\label{appx:complexity}

\update{For each layer of our method ISDEA, it can be treated as running 2 unattributed GNN $|\cR|$ times on the \ourgraphease, thus time cost is roughly $2|\cR|$ times of adopted GNN. In our experiment, we use node representation GNNs (e.g., GIN \citep{xu2018powerful}, GAT \citep{velivckovic2017graph}, GraphConv~\citep{Morris2019WL}) as our GNN architecture, thus the complexity is $\mathcal{O}(|\cR|L(|\cS|d+|\cV|d^2))$ where $L$ is the number of layers, $d$ is the maximum size of hidden layers, $|\cV|$ is number of nodes and $|\cR|$ is number of relations in the \ourgraphease, and $|\cS|$ is number of fact triplets (number of edges) in the \ourgraphease.

However, for \OurNewModel, since the update for each relation can be conducted independently, by using parrallezing or a carefully designed training batch process, we can reduce the time complexity to $\mathcal{O}(L(|\cS|d+|\cV|d^2))$, $|\cR|$ times faster than \OurModel.

Besides, for both positive and negative samples $(i,k,j)$, our method requires the shortest distance between any two nodes without considering $(i,k,j)$, which can be achieved from the Dijkstra or Floyd algorithm, \update{where we will pre-split the graph in \OurNewModel and simplify the computation of calculating distances to only one time rather than repeating it in each batch as implemented in \OurModel}.}

% For each layer of our method ISDEA, it can be treated as running 2 unattributed GNN $|\cR|$ times on the \ourgraphease, thus time cost is roughly $2|\cR|$ times of adopted GNN. In our experiment, we use node representation GNNs (e.g., GIN \citep{xu2018powerful}, GAT \citep{velivckovic2017graph}, GraphConv~\citep{Morris2019WL}) as our GNN architecture, thus the complexity is $\mathcal{O}(|\cR||\cS|d^3)$ where $d$ is the maximum size of hidden layers, $|\cR|$ is number of relations in the \ourgraphease, and $|\cS|$ is number of fact triplets (number of edges) in \ourgraphease.

% Besides, for both positive and negative samples $(i,k,j)$, our method requires the shortest distance between any two nodes without considering $(i,k,j)$. %
% Pay attention that this can not be simply achieved from the Dijkstra or Floyd algorithm since the graph changes on computing each node pair, indeed computing such distance needs to traverse the enclosed graph~\citep{zhang2018link,teru2020inductive} between each node pair once. %

\subsection{Ablation study for \OurModel}

Since a part of negative samplings is drawn by uniformly corrupting objects (without loss of generality), it is very likely that corrupted objects are far way from the subject while the true object is close to the subject. Then, the distance feature can help predict in such cases. However, the shortest distance feature will not provide any additional information if we corrupt the relation type.
Under such a scenario, shortest distance itself may provide some features to achieve good ranking performance in inductive link prediction on \ourgraphease, thus we want to know if shortest distance feature augmentation contributes to the performance gain. We perform an ablation study for \OurModel with or without distance on \ourtask over \ourdata. 

As shown in \Cref{tab:exp-ablation}, even if the shortest distance is excluded from our model, our model still performs quite well and is better than most other baselines in the \ourtask on \ourdata. Especially, as we anticipate, the distance feature is more helpful in the node prediction task than the relation prediction task. %
Thus, we can say that double equivariant node representation itself is enough to provide good performance on \ourtask. 

\begin{figure}
\begin{minipage}{1\textwidth}
\captionof{table}{
{\bf Relation \& Node performance on \OurTask over \ourdata for \OurModel with/without Shortest Distances.} We report standard deviations over 5 runs. %
A higher value means better \ourtask performance. 
{\bf Even without the shortest distance as an augmented feature, our proposal still achieves comparable results, especially in the relation prediction task.}%
}
\centering
{
%\vspace{-10pt}
\subcaption{{\bf {\scriptsize Relation prediction $(i, ?, j)$ performance in \%. Higher $\uparrow$ is better.}}}
\resizebox{0.85\linewidth}{!}{
\begin{tabular}{l|l|rrrr}
    \hline
    \multicolumn{2}{c|}{Dataset}  & MRR & Hits@1 & Hits@5 & Hits@10    \\
    \hline
    \multirow{2}{*}{EN-FR} & \OurModel w/ Distance & 70.06{\scriptsize $\pm 02.01$} & 61.46{\scriptsize $\pm 00.79$} & 82.11{\scriptsize $\pm 04.01$} & 84.94{\scriptsize $\pm 05.00$} \\
    & \OurModel w/o Distance & 68.65{\scriptsize $\pm 00.41$} & 60.34{\scriptsize $\pm 00.53$} & 80.17{\scriptsize $\pm 00.99$} & 82.80{\scriptsize $\pm 01.73$}
    \\
\hline
    \multirow{2}{*}{FR-EN} & \OurModel w/ Distance & 69.01{\scriptsize $\pm 00.57$} & 58.18{\scriptsize $\pm 00.14$} & 83.19{\scriptsize $\pm 01.73$} & 84.75{\scriptsize $\pm 02.51$} \\
    & \OurModel w/o Distance & 67.74{\scriptsize $\pm 01.15$} & 56.35{\scriptsize $\pm 01.53$} & 83.07{\scriptsize $\pm 00.75$} & 86.23{\scriptsize $\pm 00.56$}
    \\
\hline
    \multirow{2}{*}{EN-DE} & \OurModel w/ Distance & 78.38{\scriptsize $\pm 04.04$} & 68.00{\scriptsize $\pm 06.41$} & 92.39{\scriptsize $\pm 00.83$} & 95.26{\scriptsize $\pm 00.63$} \\
    & \OurModel w/o Distance & 76.52{\scriptsize $\pm 01.32$} & 67.66{\scriptsize $\pm 02.37$} & 87.49{\scriptsize $\pm 00.87$} & 88.47{\scriptsize $\pm 00.64$} 
    \\
\hline
    \multirow{2}{*}{DE-EN} & \OurModel w/ Distance & 88.82{\scriptsize $\pm 00.28$} & 84.83{\scriptsize $\pm 00.29$} & 93.59{\scriptsize $\pm 00.53$} & 94.23{\scriptsize $\pm 00.71$}  \\
    & \OurModel w/o Distance & 88.94{\scriptsize $\pm 00.92$} & 84.76{\scriptsize $\pm 00.49$} & 93.98{\scriptsize $\pm 01.74$} & 94.73{\scriptsize $\pm 01.98$} 
    \\
\hline
    \multirow{2}{*}{DB-WD} & \OurModel w/ Distance & 65.89{\scriptsize $\pm 04.71$} & 57.51{\scriptsize $\pm 05.40$} & 75.95{\scriptsize $\pm 03.89$} & 82.22{\scriptsize $\pm 02.44$} \\
    & \OurModel w/o Distance & 70.66{\scriptsize $\pm 07.05$} & 63.36{\scriptsize $\pm 05.30$} & 79.87{\scriptsize $\pm 10.19$} & 82.96{\scriptsize $\pm 11.89$}
    \\
\hline
    \multirow{2}{*}{WD-DB} & \OurModel w/ Distance & 72.57{\scriptsize $\pm 00.73$} & 62.72{\scriptsize $\pm 01.24$} & 86.10{\scriptsize $\pm 01.26$} & 88.87{\scriptsize $\pm 02.94$}  \\
    & \OurModel w/o Distance & 67.98{\scriptsize $\pm 02.14$} & 60.83{\scriptsize $\pm 01.55$} & 76.65{\scriptsize $\pm 03.14$} & 77.90{\scriptsize $\pm 03.09$} 
    \\
\hline
    \multirow{2}{*}{DB-YG} & \OurModel w/ Distance & 75.88{\scriptsize $\pm 01.58$} & 69.12{\scriptsize $\pm 02.40$} & 85.80{\scriptsize $\pm 01.23$} & 91.42{\scriptsize $\pm 01.79$} \\
    & \OurModel w/o Distance &  75.42{\scriptsize $\pm 00.35$} & 69.17{\scriptsize $\pm 01.13$} & 84.86{\scriptsize $\pm 01.58$} & 88.78{\scriptsize $\pm 02.36$}
    \\
\hline
    \multirow{2}{*}{YG-DB} & \OurModel w/ Distance & 74.04{\scriptsize $\pm 00.47$} & 66.68{\scriptsize $\pm 00.81$} & 83.36{\scriptsize $\pm 01.55$} & 85.34{\scriptsize $\pm 01.49$}  \\
    & \OurModel w/o Distance & 74.22{\scriptsize $\pm 01.56$} & 66.97{\scriptsize $\pm 01.63$} & 83.62{\scriptsize $\pm 01.85$} & 85.73{\scriptsize $\pm 02.66$}
    \\
\hline

\end{tabular}
}
}
\\
\vspace{5pt}
{
%\subcaption{{\bf {\scriptsize PediaTypes}}}
\subcaption{{\bf {\scriptsize Node prediction $(i, k, ?)$ performance in \%. Higher $\uparrow$ is better.}}}
\resizebox{0.85\linewidth}{!}{
\begin{tabular}{l|l|rrrr}
    \hline
    \multicolumn{2}{c|}{Dataset}  & MRR & Hits@1 & Hits@5 & Hits@10    \\
    \hline
    \multirow{2}{*}{EN-FR} & \OurModel w/ Distance & 53.92{\scriptsize $\pm 00.26$} & 43.03{\scriptsize $\pm 00.25$} & 64.45{\scriptsize $\pm 00.24$} & 76.28{\scriptsize $\pm 00.50$} \\
    & \OurModel w/o Distance & 45.12{\scriptsize $\pm 00.41$} & 34.04{\scriptsize $\pm 00.36$} & 56.61{\scriptsize $\pm 00.48$} & 63.46{\scriptsize $\pm 00.76$}
    \\
\hline
    \multirow{2}{*}{FR-EN} & \OurModel w/ Distance & 57.68{\scriptsize $\pm 00.68$} & 47.38{\scriptsize $\pm 00.28$} & 67.24{\scriptsize $\pm 01.32$} & 77.51{\scriptsize $\pm 01.46$}  \\
    & \OurModel w/o Distance & 42.52{\scriptsize $\pm 00.91$} & 30.41{\scriptsize $\pm 01.17$} & 54.94{\scriptsize $\pm 00.22$} & 65.29{\scriptsize $\pm 00.20$}
    \\
\hline
    \multirow{2}{*}{EN-DE} & \OurModel w/ Distance & 50.30{\scriptsize $\pm 02.08$} & 35.41{\scriptsize $\pm 02.25$} & 68.80{\scriptsize $\pm 01.90$} & 82.24{\scriptsize $\pm 00.94$} \\
    & \OurModel w/o Distance & 45.16{\scriptsize $\pm 00.76$} & 30.26{\scriptsize $\pm 00.76$} & 62.59{\scriptsize $\pm 00.57$} & 76.98{\scriptsize $\pm 00.63$}
    \\
\hline
    \multirow{2}{*}{DE-EN} & \OurModel w/ Distance & 51.33{\scriptsize $\pm 00.40$} & 37.12{\scriptsize $\pm 00.31$} & 68.20{\scriptsize $\pm 00.53$} & 81.80{\scriptsize $\pm 00.68$}  \\
    &\OurModel  w/o Distance & 43.67{\scriptsize $\pm 00.32$} & 28.97{\scriptsize $\pm 00.25$} & 60.36{\scriptsize $\pm 00.54$} & 74.95{\scriptsize $\pm 00.51$}
    \\
\hline
    \multirow{2}{*}{DB-WD} & \OurModel w/ Distance & 45.75{\scriptsize $\pm 00.66$} & 35.59{\scriptsize $\pm 00.73$} & 54.83{\scriptsize $\pm 00.90$} & 66.69{\scriptsize $\pm 01.01$}\\
    & \OurModel w/o Distance & 40.26{\scriptsize $\pm 03.77$} & 30.59{\scriptsize $\pm 03.89$} & 48.15{\scriptsize $\pm 03.68$} & 59.43{\scriptsize $\pm 03.76$}
    \\
\hline
    \multirow{2}{*}{WD-DB} & \OurModel w/ Distance & 51.64{\scriptsize $\pm 00.60$} & 40.56{\scriptsize $\pm 01.72$} & 62.60{\scriptsize $\pm 02.55$} & 75.19{\scriptsize $\pm 03.12$} \\
    & \OurModel w/o Distance & 45.94{\scriptsize $\pm 00.14$} & 35.17{\scriptsize $\pm 00.30$} & 56.89{\scriptsize $\pm 00.33$} & 66.46{\scriptsize $\pm 00.55$} 
    \\
\hline
    \multirow{2}{*}{DB-YG} & \OurModel w/ Distance & 41.72{\scriptsize $\pm 01.64$} & 27.70{\scriptsize $\pm 01.95$} & 55.21{\scriptsize $\pm 01.07$} & 72.87{\scriptsize $\pm 01.03$}  \\
    & \OurModel w/o Distance & 32.71{\scriptsize $\pm 00.60$} & 17.69{\scriptsize $\pm 00.39$} & 47.82{\scriptsize $\pm 00.60$} & 66.92{\scriptsize $\pm 01.90$} 
    \\
\hline
    \multirow{2}{*}{YG-DB} & \OurModel w/ Distance & 48.21{\scriptsize $\pm 01.06$} & 35.29{\scriptsize $\pm 01.67$} & 61.87{\scriptsize $\pm 01.30$} & 76.41{\scriptsize $\pm 01.52$}   \\
    & \OurModel w/o Distance & 37.52{\scriptsize $\pm 00.79$} & 23.10{\scriptsize $\pm 00.76$} & 53.34{\scriptsize $\pm 00.88$} & 68.43{\scriptsize $\pm 01.62$}
    \\
\hline

\end{tabular}
}
}
\label{tab:exp-ablation}
\vspace{-5pt}
\end{minipage}
\end{figure}
