# Supplementary material for: Double Equivariance for Inductive Link Prediction for Both New Nodes and New Relation Types
Source: arXiv:2302.01313 source file (2025-01-14)
Supplement: Supplementary file 5 [file exp_solely_new_nodes.tex]

\subsection{Inductively link prediction over solely new nodes}
\label{subsec:exp-node-ind}

In this section, we provide the experiment results and analysis comparing our method with SOTA baselines on inductive link prediction over solely new nodes. Note that this task is intrinsically different than our proposed \ourtask.
Different from our task where the model will be exposed to new relations, inductively link prediction over solely new nodes will ensure test relation types are the same as training relation types.

\subsubsection{Experiment Setup}
\label{sec:exp-set-nodes}

\paragraph{Datasets.}
Inductively link prediction over solely new nodes are wildly studied in literature~\cite{teru2020inductive,zhu2021neural,yang2017differentiable}. We propose one synthetic task FD1, and pick the most widely used benchmarks, WN18RR, FB237 and NELL995 ~\cite{teru2020inductive}, as our datasets. Each benchmark has four pairs of graphs for inductive link prediction. For graphs of each pair, they contains two thoroughly distinct sets of nodes, but the same set of relations. The learning task is tuning a model on the first graph, and apply tuned model to predict missing head or tail nodes for querying triplets on the second graph.

\begin{figure}[h]
%\vspace{-25pt}
\centering
\begin{minipage}{\linewidth}
\centering
\includegraphics[width=.5\linewidth]{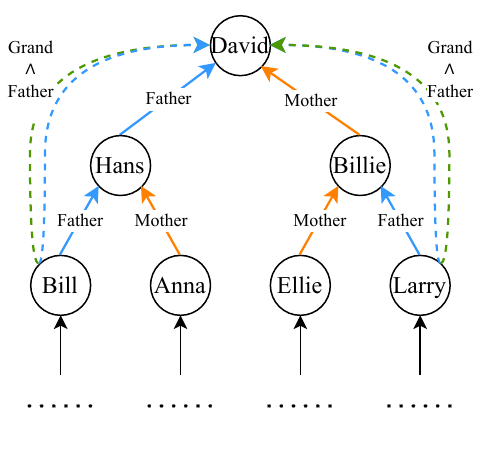}
\vspace{-25pt}
\subcaption{{\bf Training}}
\end{minipage}
\\
\begin{minipage}{\linewidth}
\centering
\includegraphics[width=.5\linewidth]{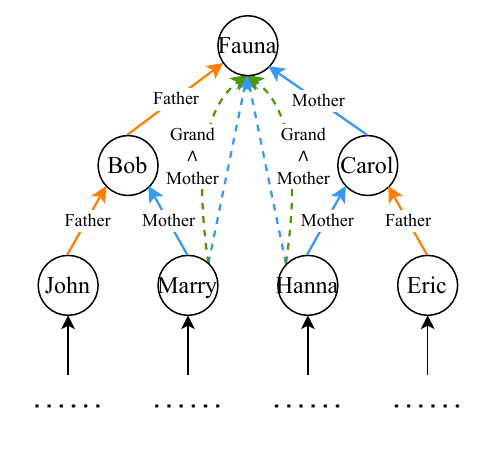}
\vspace{-25pt}
\subcaption{{\bf Test}}
\end{minipage}
\caption{
{\bf Synthetic Example of FD-1:} The arrow direction implies ``who is with which relation of whom''. For instance, the directed edge $(\text{Hans}, \text{Father}, \text{David})$ means ``Hans is father of David''.}
\label{fig:example-fd1}
%\vspace{-10pt}
\end{figure}
\paragraph{Baseline and Implementation Details.}
We compare with four widely used and SOTA approaches for inductively link prediction over solely new nodes: Neural LP~\cite{yang2017differentiable}, DRUM~\cite{sadeghian2019drum}, GraIL~\cite{teru2020inductive} and NBFNet~\cite{zhu2021neural}. All neural network approaches, including the models proposed in this paper, are implemented in PyTorch~\cite{pytorchcitation} and Pytorch Geometric~\cite{FeyLenssen2019} (available
 respectively under the BSD and MIT license). Same as \cite{teru2020inductive,zhu2021neural}, we run each method 5 times on each dataset, and collect mean performance whose standard deviations are omitted since they are all small. For training of each single run, we augment each triplet $(i, r, j)$ by its inversion $(i, r^{-1}, j)$, and sample 2 negative triplets $(i', r, j')$ per positive in training as \cite{sun2018rotate,zhu2021neural}; For evaluation, we will not augment triplets by inversions, and sample 50 negative triplets per positive to compute common metrics such as Mean Reciprocal Rank (MRR) and Hits@$k$ as all baselines. For each positive sample, its negative samples are generated by uniformly corrupt either its subject or object by a random node. We will filter out negative samples that collide with any positive triplets in facts and sample them again until there is no collision. Besides, we only corrupt objects in training, since corruption of subject can be achieved from corrupting object of inverse triplets \cite{sun2018rotate,zhu2021neural}. Note this negative sampling procedure is different from the main paper since here we are following the conventional inductive \ourgraphease completion~\cite{teru2020inductive, zhu2021neural} task over solely new nodes. Training was performed on NVIDIA Telsa P100, GeForce RTX 2080 Ti, and TITAN V GPUs.

\paragraph{Hyperparameters.} We follow the same configuration as \cite{teru2020inductive} such that hidden layer is of 32 neurons, use Adam optimizer with learning rate 0.01, and weight decay 5e-4. For all dataset, we train our model 50 epochs with batch size 256. If the model is not improving for 15 epochs, we early stop the training. For all methods, number of hops and number of layers are 2 on FD-1, and are 3 on real-world inductive \ourgraphease completion to ensure fair comparison.

\subsubsection{A Synthetic Case Study}

As introduced in \Cref{subsec:exp-node-ind}, we construct a simple synthetic task, {\bf FD-1} to empirically justify the expressivity of our proposal against other approaches.
The task is based on simple family tree with only parent and grand parent relation types.
The goal is to learn to predict female grand parent relation type (grand mother) while \textbf{only} male grand parent relation type (grand father) are provided in training. Note that we do not consider grand mother as new relation type in test, since we have already observed both ``grand" and ``mother" relation types in training.
An simple illustration of this synthetic task is provided in \Cref{fig:example-fd1}, and the synthesis generation pseudo code is provided in \Cref{alg:synth-fd1}.

\begin{algorithm}
\caption{{\bf Synthesis Algorithm for FD-1.} This is triplet generation code for a single graph (either training and test). It will provide observation and query triplets. For training, query triplets are further divided into training and validation triplets; For test, query triplets directly become test triplets.}
\label{alg:synth-fd1}
\begin{algorithmic}[1]
\Require Depth $D$, Training flag ``$\text{is{\_}train}$'', Node Labeling ``$\text{Names}$''.
\Ensure Observation triplets $\cS$, Query triplets $\cQ$
\State $\cS \leftarrow \emptyset$
\State $\cQ \leftarrow \emptyset$
\For{$d \leftarrow 1, \ldots, D$}
    \For{$v \leftarrow 2^d - 1, \ldots, 2^{d + 1} - 2$}
        \State $u_1 \leftarrow \lceil \sfrac{(v - 2)}{2} \rceil$
        \State $u_2 \leftarrow \lceil \sfrac{(u_1 - 2)}{2} \rceil$
        \If{$v \text{ mod } 2 = 0$}
            \Comment{$v$ is female.}
            \If{$u_1 \geq 0$}
                \State $\cS$.add$\big(\,(\text{Names}[v], \text{Mother}, \text{Names}[u_1])\,\big)$
            \EndIf
            \If{$u_2 \geq 0$ and $\neg \text{is{\_}train}$}
                \Comment{Test query.}
                \State $\cQ$.add$\big(\,(\text{Names}[v], \text{Grand}, \text{Names}[u_2])\,\big)$
                \State $\cQ$.add$\big(\,(\text{Names}[v], \text{Mother}, \text{Names}[u_2])\,\big)$
            \EndIf
        \Else
            \Comment{$v$ is male.}
            \If{$u_1 \geq 0$}
                \State $\cS$.add$\big(\,(\text{Names}[v], \text{Father}, \text{Names}[u_1])\,\big)$
            \EndIf
            \If{$u_2 \geq 0$ and $\text{is{\_}train}$}
                \Comment{Training query.}
                \State $\cQ$.add$\big(\,(\text{Names}[v], \text{Grand}, \text{Names}[u_2])\,\big)$
                \State $\cQ$.add$\big(\,(\text{Names}[v], \text{Father}, \text{Names}[u_2])\,\big)$
            \EndIf
        \EndIf
    \EndFor
\EndFor
\end{algorithmic}
\end{algorithm}

Before we move to the result of this task, we want to first highlight several interesting properties of this dataset which is useful to examine expressivity of a attributed graph representation:
\begin{itemize}[leftmargin=*]
\item The logical reasoning is very simple to learn: Two consecutive parent relations will result in a grand parent relation of the first parent type. For example, if Larry is father of Billie, and Billie is father of David, then Larry is grand father of David as \Cref{fig:example-fd1}(a). An expressive representation should easily capture this, and performs well on test.
\vspace{-3pt}
\item If we ignore the identities of relation types (labeling bijections), training and test graphs are indeed the same graphs. This can be easily observed if you ignore edge lables and focus only edge colors of each graph (flipping colors will not change graph). Thus, an expressive representation should perform similarly on training and test graphs.
\vspace{-3pt}
\item On the other hand, if we focus only on edge lables, \textbf{not} colors, we will find that all observations (solid edges) of training and test are same, while the querying triplets (dashed edges) are non-overlapping. Indeed, every test query (grand mother) will be treated as negative triplets in training (since they are missing), while they should be predicted as positive at test time. Thus, if a representation improperly focuses only on edge labels, it will perform poorly on test, while perform perfectly on training.
\vspace{-3pt}
\item The graphs are highly symmetric, thus representations that are equivariant only to node permutations can not perform well on test graph. For example, the 1-hop local structure around Marry and Hanna in test graph are exactly the same, thus it is impossible for node-equivariant representation to distinguish them, and if we use these representation to tell their relations with Bob, they will predict both as ``Mother'' which is not true for Hanna. If we go deeper on given graphs (trees), you will find more such node pairs which are far away but have exactly the same node-equivariant representations which will hurt prediction performance. Thus, only pairwise-equivariant representation can work well. Please refer more details to \cite{srinivasan2020on}.
\end{itemize}

We provide the results on FD-1 in \Cref{tab:exp-fd1}. We can see that ISDEA significantly outperforms all baselines. This task tests the relation-invariance property of ISDEA.

Interestingly, the baselines that tend to perform better on real-world \ourgraphease (e.g., NBFNet~\cite{zhu2021neural}, GraIL~\cite{teru2020inductive}) tend to perform worse on FD-1. This is because training and test queries are conflicting: Positive triplet queries in the training graph are negative queries in test, while positive test queries become negative in training. Hence, for models that does not have the double-invariance property, the better it can perform on triplets similar to the ones seeing in training, the worse it will perform on the test data. 

\begin{table}[t!]
\centering
\resizebox{0.6\linewidth}{!}{
\begin{tabular}{l|cccc}
    \hline
    \multirow{2}{*}{Model} & \multicolumn{4}{c}{FD-1} \\
    \cline{2-5}
    & MRR$\uparrow$ & Hits@1$\uparrow$ & Hits@2$\uparrow$ & Hits@4$\uparrow$ \\
    \hline
    Neural LP & 50.20 & 33.90 & 41.50 & 65.10  \\
    DRUM & 50.20 & 33.90 & 41.50 & 65.10  \\
    GraIL & 42.20 & 18.10 & 41.60 & 74.00 \\
    NBFNet & 31.10 & 26.20 & 31.80 & 32.20 \\
\hline
ISDEA & \textbf{84.80} & \textbf{73.80} & \textbf{89.50} & \textbf{98.40} \\
    \hline
\end{tabular}
}
\vspace{5pt}
\caption{\textbf{(Node) Inductive link prediction over solely new nodes performance on Family Diagrams 1.} Existing baselines clearly struggle to perform the task.}
\label{tab:exp-fd1}
\vspace{-10pt}
\end{table}

Since FD-1 comes from an extremely simple generation process, people may expect our methods to achieve perfect performance on it (always rank positive triplets at rank 1 against all corresponding negative samples). However, it seems like that ISDEA fails to achieve perfect performance (MRR and Hits@$k$ all being 1.0) on this simple task. Indeed, there is no way to achieve such perfect performance on MRR, Hits@1 and Hits@2. The issue is that in the querying grand parent relations, there will be two equally good choices, e.g., $(X, \text{Mother}, \text{Fauna}), X \in \{\text{Marry}, \text{Hanna}\}$; $(X, \text{Grand}, \text{Fauna}), X \in \{\text{John}, \text{Marry}, \text{Hanna}, \text{Erie}\}$. But if we see Hits@4, ISDEA achieves almost 100\% accuracy. 

Another minor observation is that Neural LP and DRUM has exactly the same performance on FD-1. The reason is that Neural LP and DRUM has exactly the same framework except that the neural network architecture are slightly different. This observation is also found in \cite{teru2020inductive,zhu2021neural}, and this also happens in later real-world experiments.

\subsubsection{Real World Datasets \yangze{for over solely new nodes}}

\begin{table}[t!!!]
\centering
\vspace{-5pt}
\resizebox{0.7\linewidth}{!}{
\begin{tabular}{l|l|l|c|c|c|c|c}
    \hline
    \multicolumn{3}{c|}{Dataset} & Neural LP & DRUM & GraIL & NBFNet & ISDEA \\
    \hline
    \multirow{8}{*}{\rotatebox{90}{WN18RR}} & \multirow{2}{*}{v1} & Original & 82.50 & 82.30 & 84.00 & \textbf{94.90} & \underline{91.90} (01.20) \\
    \cline{3-8}
    & & Permuted &68.60 & 74.50 & \underline{82.20} & 63.00 & \textbf{91.90} (01.20)   \\
    \cline{2-8}
    & \multirow{2}{*}{v2} & Original & 83.90 & 84.70 & 81.60 & \textbf{96.00} & \underline{93.70} (00.40)  \\
    \cline{3-8}
    & & Permuted &  77.20 & \underline{83.70} & 81.60 & 83.30 & \textbf{93.70} (00.40) \\
    \cline{2-8}
    & \multirow{2}{*}{v3} & Original & 60.70 & 61.10 & 63.30 & \textbf{90.70} & \underline{87.70} (01.60) \\
    \cline{3-8}
    & & Permuted & 59.40 & 60.40 & 63.30 & \underline{71.60} & \textbf{87.70} (01.60)\\
    \cline{2-8}
    & \multirow{2}{*}{v4} & Original  & 75.20 & 74.60 & 76.30 & \textbf{89.00} & \underline{77.20} (01.70) \\
    \cline{3-8}
    & & Permuted & 62.80 & 69.80 & \underline{76.30} & 47.40 & \textbf{77.20} (01.70)  \\
    \hline
    \hline
    \multirow{8}{*}{\rotatebox{90}{FB237}} & \multirow{2}{*}{v1} & Original & 52.90 & 52.90 & 74.10 & \textbf{89.50} & \underline{80.10} (04.40)  \\
    \cline{3-8}
    & & Permuted & 42.40 & 42.20 & \underline{71.70} & 60.50 & \textbf{80.10} (04.40)  \\
    \cline{2-8}
    & \multirow{2}{*}{v2} & Original& 58.90 & 58.70 & 88.40 & \textbf{97.70} & \underline{89.10} (01.30)  \\
    \cline{3-8}
    & & Permuted & 47.80 & 51.00 & \underline{86.40} & 70.70 & \textbf{89.10} (01.30) \\
    \cline{2-8}
    & \multirow{2}{*}{v3} & Original& 52.90 & 52.90 & 88.70 & \textbf{98.00} & \underline{89.30} (00.40) \\
    \cline{3-8}
    & & Permuted & 44.30 & 40.70 & \underline{85.90} & 74.10 & \textbf{89.30} (00.40) \\
    \cline{2-8}
    & \multirow{2}{*}{v4} & Original & 55.90 & 55.90 & 89.30 & \textbf{98.70} & \underline{91.40} (00.80) \\
    \cline{3-8}
    & & Permuted & 37.20 & 37.50 & \underline{87.30} & 72.50 & \textbf{91.40} (00.80) \\
    \hline
    \hline
    \multirow{8}{*}{\rotatebox{90}{NELL995}} & \multirow{2}{*}{v1} & Original & 50.00 & 50.00 & 93.20 & \textbf{99.50} & \underline{97.50} (04.30) \\
    \cline{3-8}
    & & Permuted & 50.00 & 50.00 & 73.40 & \textbf{99.50} & \underline{97.50} (04.30) \\
    \cline{2-8}
    & \multirow{2}{*}{v2} & Original & 78.70 & 78.60 & \underline{96.30} & \textbf{97.80} & 91.20 (01.90) \\
    \cline{3-8}
    & & Permuted  & 38.40 & 42.50 & 89.90 & \textbf{97.80} & \underline{91.20} (01.90)  \\
    \cline{2-8}
    & \multirow{2}{*}{v3} & Original  & 82.70 & 82.70 & \underline{95.80} & \textbf{96.90} & 93.50 (01.10) \\
    \cline{3-8}
    & & Permuted & 39.70 & 44.10 & \underline{94.70} & \textbf{96.80} & 93.50 (01.10) \\
    \cline{2-8}
    & \multirow{2}{*}{v4} & Original & 80.60 & 80.60 & \underline{88.00} & \textbf{95.70} & 84.60 (01.20)  \\
    \cline{3-8}
    & & Permuted & 34.00 & 35.20 & 80.60 & \textbf{93.70} & \underline{84.60} (01.20)\\
    \hline
\end{tabular}
}
\vspace{5pt}
\caption{{\bf (Node) Hits@10 performance on inductive link prediction over solely new nodes on real-world {\ourgraphease}s.} ISDEA reaches close to state-of-the-art performance on almost all tasks, and is invariant to relation permutation on all tasks. For our model, we also report standard deviation in parentheses.}
\label{tab:exp-real-v1}
\vspace{-10pt}
\end{table}
We select 12 inductive \ourgraph completion benchmarks, 4 inductive splits of 3 datasets WN18RR, FB237 and NELL995 to test our proposal. In order to highlight the relation-invariance property of our proposal, we also perform a task where all relation IDs are randomly shuffled only in test.

As GraIL~\cite{teru2020inductive} and NBFNet~\cite{zhu2021neural}, we report (Node) Hits@10 for inductive link prediction over solely new nodes in \Cref{tab:exp-real-v1}. %
We can see that ISDEA results are always invariant to the permutation of relations in test, while all baselines become worse at least on one dataset if relations are permuted in test. Besides, ISDEA obtains second to the state-of-the-art score on the key metric Hits@10 on almost each benchmark dataset except the NELL995 dataset. %

While double exchangeability may not be the right assumption in link prediction over solely new nodes, it is clearly still beneficial for some tasks.
Our model currently treats all relations as exchangeable.
Further research is needed to better understand which relations are exchangeable and which are not for a given \ourgraphease. 
We also believe that using true pairwise representation can improve the performance of ISDEA.

One interesting observation is that besides our proposal, some baselines are also insensitive to relation shuffling on some datasets, e.g., NBFNet on NELL995. We suppose the reason is that inductive NELL995 inductive \ourgraphease completion tasks can be simply reduced to link prediction tasks where relation ID has barely no influence. To verify this guess, we force NBFNet relation embeddings to be all-one (forcing all relations to be the same), and run the experiments again, we can see that the performance is nearly the same as original on NELL-v2 and NELL-v3, and is still fine on NELL-v1 and NELL-v4 in \Cref{tab:exp-sparse} which reflects that the inductive \ourgraphease completion on NELL995 is nearly equivalent to link prediction.

\begin{table}[t!]
\centering
\begin{tabular}{l|c|c|c|c}
    \hline
    \multirow{2}{*}{NBFNet Configuration} & \multicolumn{4}{c}{NELL995 Dataset} \\
    \cline{2-5}
    & v1 & v2 & v3 & V4 \\
    \hline
    Original & 99.50 & 97.80 & 96.90 & 95.70 \\
    With Constant Relation Embeddings & 74.00 & 94.90 & 92.80 & 87.70 \\
    \hline
\end{tabular}
\vspace{5pt}
\caption{{\bf (Node) Hits@10 Performance without/with Constant Relation Embeddings.} Forcing NBFNet relation embeddings to be the same constant still perform well on some NELL995 datasets. This shows that some inductive \ourgraphease link prediction over solely new nodes tasks can be approximated by link predictions.}
% \vspace{-20pt}
\label{tab:exp-sparse}
\end{table}
