# Supplementary material for: Double Equivariance for Inductive Link Prediction for Both New Nodes and New Relation Types
Source: arXiv:2302.01313 source file (2025-01-14)
Supplement: Supplementary file 9 [file ingram_dataset.tex]

\subsubsection{\OurTask over datasets from InGram (Lee et al., 2023)}

\citet{ingram} proposed the NL-$k$, WK-$k$, and FB-$k$ benchmarks originally used to evaluate InGram's performance of reasoning over new nodes and new relation types at test time, where $k \in \{ 25, 50, 75, 100 \}$ means that, in the test graphs, approximately $k\%$ of triplets have unseen relations. For example, the test graph of WK-100 does not contain any training relations and thus induces a \ourtask task. Hence, we run our models (\OurModel and \OurOtherModel) against InGram on these benchmarks with results shown in~\Cref{tab:ingram-dataset}. We note that, however, due to the different experimental settings (as we discuss next), our results reported in~\Cref{tab:ingram-dataset} are not directly comparable to those reported in~\citet{ingram}, even though they are experimented on essentially the same datasets.

\paragraph{Difference to the original data split and evaluation in InGram~\citep{ingram}:} Different from~\citet{ingram}, which uses part of the test graph as the validation set to conduct model hyperparameter search, {\em our experiments consider a harder setting where the relations in test are not observed in the validation data}. Hence, to modify the NL-$k$, WK-$k$, and FB-$k$ datasets to our setting, we discard the original validation set and instead split the original training set into a new set of training and validation triplets with a ratio of 9:1. During training, the models perform self-supervised masking over the training set of triplets to create the training-time observable triplets and training-time target triplets. During validation, the entire set of the new training triplets is taken as the validation-time observable triplets, and the new validation triplets are the target triplets to predict. In addition, \citet{ingram} evaluate their model's node prediction performance against \textit{all} nodes in the graph. For efficiency reasons, we evaluate the model performance by sampling without replacement 50 negative nodes for the node prediction task and sampling with replacement 50 negative relation types for the relation prediction task.

\Cref{tab:ingram-dataset} shows the results, where we can see that \OurModel outperforms InGram on most datasets on the relation prediction task and has smaller standard deviation in general, and \OurOtherModel consistently outperforms InGram on all datasets for both relation prediction and node prediction tasks. Importantly, in the dataset FB-100 which follows our \ourtask setting with completely new nodes and new relation types in the test with the largest number of training and test relations ($134$ in train and $77$ in test)~\citep{ingram}, \OurModel achieves significant better results in the relation perdiction task, showcasing its ability for \ourtask.

\begin{table}[t]
% \vspace{-25pt}   % Reduce table head space to the top of the page
\centering
\captionof{table}{
{\bf Relation \& Node Hits@10 performance on \OurTask over NL-$k$, WK-$k$, and FB-$k$ of~\citet{ingram}.} We report standard deviations over 5 runs. %
A higher value means better \ourtask performance. 
The best values are shown in bold font, while the second-best values are underlined. 
{\bf \OurModel outperforms InGram on most datasets on the relation prediction task, and \OurOtherModel consistently outperforms InGram on all datasets for both relation prediction and node prediction tasks.}
}
%\vspace{5pt}
{
\subcaption{{\bf {\scriptsize Performance in \% on WK-$k$ datasets. Higher $\uparrow$ is better.}}}
\resizebox{1.0\linewidth}{!}{
\begin{tabular}{l r r r r c r r r r}
    & \multicolumn{4}{c}{Relation prediction $(i, ?, j)$} & & \multicolumn{4}{c}{Node prediction $(i, k, ?)$} \\
    
    \cmidrule{2-5} \cmidrule{7-10} 
    Models & WK-25 & WK-50 & WK-75 & WK-100 & & WK-25 & WK-50 & WK-75 & WK-100 \\
    \midrule
    
    InGram & 58.76{\scriptsize $\pm 13.91$} & {84.01}{\scriptsize $\pm 03.30$} & 80.19{\scriptsize $\pm 04.19$} & 58.20{\scriptsize $\pm 11.13$} & & {76.99}{\scriptsize $\pm 07.72$} & 70.93{\scriptsize $\pm 02.38$} & {78.85}{\scriptsize $\pm 04.65$} & 66.29{\scriptsize $\pm 03.70$} \\
    \midrule
    
    \OurOtherModel (Ours) & \underline{81.06}{\scriptsize $\pm 22.31$} & \textbf{94.85}{\scriptsize $\pm 00.85$} & \textbf{95.84}{\scriptsize $\pm 01.54$} & \underline{81.83}{\scriptsize $\pm 10.10$} & & \underline{87.91}{\scriptsize $\pm 05.68$} & \underline{82.58}{\scriptsize $\pm 01.70$} & \underline{89.10}{\scriptsize $\pm 02.15$} & \underline{79.69}{\scriptsize $\pm 03.07$} \\
    
    % \OurModel (Ours) & \underline{79.49}{\scriptsize $\pm 06.88$} & {81.25}{\scriptsize $\pm 07.02$} & \underline{84.92}{\scriptsize $\pm 06.86$} & \underline{79.70}{\scriptsize $\pm 07.68$} & & 58.28{\scriptsize $\pm 23.68$} & \underline{73.24}{\scriptsize $\pm 00.57$} & 76.19{\scriptsize $\pm 01.04$} & \underline{71.76}{\scriptsize $\pm 01.85$} \\

    \update{\OurNewModel (Ours)} & \update{\textbf{96.25}{\scriptsize $\pm 00.86$}} & \update{\underline{93.10}{\scriptsize $\pm 02.55$}} & \update{\underline{95.66}{\scriptsize $\pm 00.82$}} & \update{\textbf{95.00}{\scriptsize $\pm 00.15$}} & & \update{\textbf{94.41}{\scriptsize $\pm 01.61$}} & \update{\textbf{90.34}{\scriptsize $\pm 01.71$}} & \update{\textbf{91.98}{\scriptsize $\pm 01.61$}} & \update{\textbf{91.22}{\scriptsize $\pm 00.45$}}
\end{tabular}
\label{tab:ingram-dataset-WK}
}
\vspace{5pt}
\subcaption{{\bf {\scriptsize Performance in \% on FB-$k$ datasets. Higher $\uparrow$ is better.}}}
\resizebox{1.0\linewidth}{!}{
\begin{tabular}{l r r r r c r r r r}
    & \multicolumn{4}{c}{Relation prediction $(i, ?, j)$} & & \multicolumn{4}{c}{Node prediction $(i, k, ?)$} \\
    
    \cmidrule{2-5} \cmidrule{7-10} 
    Models & FB-25 & FB-50 & FB-75 & FB-100 & & FB-25 & FB-50 & FB-75 & FB-100 \\
    \midrule
    
    InGram & 68.26{\scriptsize $\pm 08.27$} & 50.41{\scriptsize $\pm 08.79$} & 79.51{\scriptsize $\pm 02.69$} & 40.46{\scriptsize $\pm 12.21$} & & \underline{86.79}{\scriptsize $\pm 00.70$} & {73.32}{\scriptsize $\pm 06.64$} & {86.57}{\scriptsize $\pm 00.69$} & 71.72{\scriptsize $\pm 06.93$} \\
    \midrule
    
    \OurOtherModel (Ours) & \underline{82.89}{\scriptsize $\pm 03.58$} & \underline{76.65}{\scriptsize $\pm 04.05$} & \underline{89.70}{\scriptsize $\pm 01.14$} & \underline{46.88}{\scriptsize $\pm 15.76$} & & \textbf{92.39}{\scriptsize $\pm 00.30$} & \underline{81.08}{\scriptsize $\pm 06.98$} & \textbf{92.14}{\scriptsize $\pm 00.43$} & \underline{77.54}{\scriptsize $\pm 06.36$} \\
    
    % \OurModel (Ours) & \textbf{83.63}{\scriptsize $\pm 05.66$} & \textbf{78.70}{\scriptsize $\pm 05.90$} & \underline{81.27}{\scriptsize $\pm 07.24$} & \textbf{85.41}{\scriptsize $\pm 04.43$} & & 75.93{\scriptsize $\pm 00.49$} & 69.90{\scriptsize $\pm 00.81$} & 73.45{\scriptsize $\pm 01.17$} & \textbf{79.70}{\scriptsize $\pm 00.81$} \\

    \update{\OurNewModel (Ours)} & \update{\textbf{96.68}{\scriptsize $\pm 00.15$}} & \update{\textbf{93.55}{\scriptsize $\pm 00.77$}} & \update{\textbf{96.86}{\scriptsize $\pm 00.58$}} & \update{\textbf{97.55}{\scriptsize $\pm 00.33$}} & & \update{85.01{\scriptsize $\pm 00.92$}} & \update{\textbf{84.40}{\scriptsize $\pm 00.38$}} & \update{\underline{86.62}{\scriptsize $\pm 00.31$}} & \update{\textbf{91.28}{\scriptsize $\pm 00.19$}}
\end{tabular}
\label{tab:ingram-dataset-FB}
}
\vspace{5pt}
\subcaption{{\bf {\scriptsize Performance in \% on NL-$k$ datasets. Higher $\uparrow$ is better.}}}
\resizebox{1.0\linewidth}{!}{
\begin{tabular}{l r r r r c r r r r}
    & \multicolumn{4}{c}{Relation prediction $(i, ?, j)$} & & \multicolumn{4}{c}{Node prediction $(i, k, ?)$} \\
    
    \cmidrule{2-5} \cmidrule{7-10} 
    Models & NL-25 & NL-50 & NL-75 & NL-100 & & NL-25 & NL-50 & NL-75 & NL-100 \\
    \midrule
    
    InGram & 64.54{\scriptsize $\pm 16.86$} & 64.54{\scriptsize $\pm 12.56$} & {80.16}{\scriptsize $\pm 04.43$} & 70.84{\scriptsize $\pm 08.52$} & & \underline{89.95}{\scriptsize $\pm 02.01$} & \underline{92.74}{\scriptsize $\pm 00.52$} & \underline{95.40}{\scriptsize $\pm 01.38$} & {88.20}{\scriptsize $\pm 01.92$} \\
    \midrule
    
    \OurOtherModel (Ours) & \underline{83.58}{\scriptsize $\pm 17.57$} & \underline{91.32}{\scriptsize $\pm 05.60$} & \underline{96.01}{\scriptsize $\pm 01.23$} & \underline{87.52}{\scriptsize $\pm 10.39$} & & \textbf{95.03}{\scriptsize $\pm 00.32$} & \textbf{96.02}{\scriptsize $\pm 00.34$} & \textbf{97.94}{\scriptsize $\pm 00.34$} & \textbf{93.80}{\scriptsize $\pm 01.38$} \\
    
    % \OurModel (Ours) & \underline{69.49}{\scriptsize $\pm 05.71$} & \underline{76.23}{\scriptsize $\pm 06.92$} & 76.03{\scriptsize $\pm 03.31$} & \underline{80.84}{\scriptsize $\pm 07.35$} & & 73.74{\scriptsize $\pm 03.35$} & 75.76{\scriptsize $\pm 03.52$} & 77.27{\scriptsize $\pm 03.80$} & 72.81{\scriptsize $\pm 04.41$} \\
    \update{\OurNewModel (Ours)} & \update{\textbf{92.04}{\scriptsize $\pm 02.67$}} & \update{\textbf{93.78}{\scriptsize $\pm 01.37$}} & \update{\textbf{96.57}{\scriptsize $\pm 01.85$}} & \update{\textbf{99.72}{\scriptsize $\pm 00.15$}} & & \update{{82.20}{\scriptsize $\pm 04.36$}} & \update{83.35{\scriptsize $\pm 00.40$}} & \update{90.94{\scriptsize $\pm 00.85$}} & \update{\underline{90.06}{\scriptsize $\pm 00.49$}}
\end{tabular}
\label{tab:ingram-dataset-NL}
}
% \vspace{-15pt}  % Reduce table bottom space to the text
}
\label{tab:ingram-dataset}
\end{table}
