# Supplementary material for: Double Equivariance for Inductive Link Prediction for Both New Nodes and New Relation Types
Source: arXiv:2302.01313 source file (2025-01-14)
Supplement: Supplementary file 10 [file limitation.tex]

\subsubsection{Expressivity Limitation Case Study with FD-2 for \OurModel}
\label{subsubsec:limit}
We now provide a FD-2 variant where we show that \ourequiv representation is not expressive enough to solve a specific task. It is a simple 2-depth tree structure as shown in \Cref{fig:example-limit}.
We denote node representations given by arbitrary \ourequiv representation as $H_{v, r}$ where $v \in [1, 7]$ and $r \in [1, 4]$. We can easily notice that $e_4$ and $e_7$ are symmetric, $e_5$ and $e_6$ are symmetric (simply flipping blue and orange colors), thus we will expect $H_{4, 1} = H_{7, 2}, H_{4, 2} = H_{7, 1}, H_{5, 1} = H_{6, 2}, H_{5, 2} = H_{6, 1}$.

\begin{figure}[h]
\centering
\includegraphics[width=0.3\linewidth]{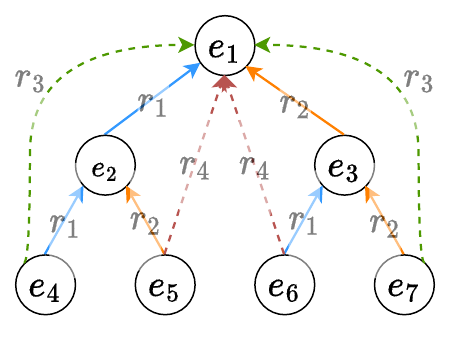}
\caption{
{\bf Expressivity Limitation:} Relation $r_1$ and $r_2$ are always observed, while $r_3$ and $r_4$ are always querying. $r_3$ implies that relation types on the path are same, while $r_4$ implies that relation types on the path are different..}
\label{fig:example-limit}
\end{figure}

Since there is no $r_3$ and $r_4$ in observation, they are freely exchangeable with each other, thus we will also expect 
\begin{equation*}
\begin{gathered}
H_{1, 3} = H_{1, 4}, \\
H_{4, 3} = H_{4, 4} = H_{7, 4} = H_{7, 3}, \\
H_{5, 3} = H_{5, 4} = H_{6, 4} = H_{6, 3}. \\
\end{gathered}
\end{equation*}

After getting all those representations, we can now focus on querying triplet representations (dashed green and red) by concatenating head and tail node representations w.r.t. relation types:
\begin{equation*}
\begin{gathered}
\trifunc{\Gamma} \left( \left( e_1, r_4, e_4 \right), \adj \right) = H_{1, 4} \mathbin\Vert H_{4, 4}, \\
\trifunc{\Gamma} \left( \left( e_1, r_3, e_5 \right), \adj \right) = H_{1, 3} \mathbin\Vert H_{5, 3}, \\
\trifunc{\Gamma} \left( \left( e_1, r_3, e_6 \right), \adj \right) = H_{1, 3} \mathbin\Vert H_{6, 3} ,\\
\trifunc{\Gamma} \left( \left( e_1, r_4, e_7 \right), \adj \right) = H_{1, 4} \mathbin\Vert H_{7, 4}. \\
\end{gathered}
\end{equation*}

We can notice that
\begin{equation*}
\begin{gathered}
\overbrace{H_{1, 4} \mathbin\Vert H_{4, 4}}^{\trifunc{\Gamma} \left( \left( e_1, r_4, e_4 \right), \adj \right)} = \overbrace{H_{1, 4} \mathbin\Vert H_{7, 4}}^{\trifunc{\Gamma} \left( \left( e_1, r_4, e_7 \right), \adj \right)}
= \overbrace{H_{1, 3} \mathbin\Vert H_{7, 3}}^{\trifunc{\Gamma} \left( \left( e_1, r_3, e_7 \right), \adj \right)} = \overbrace{H_{1, 3} \mathbin\Vert H_{4, 3}}^{\trifunc{\Gamma} \left( \left( e_1, r_3, e_4 \right), \adj \right)}, \\
\overbrace{H_{1, 4} \mathbin\Vert H_{5, 4}}^{\trifunc{\Gamma} \left( \left( e_1, r_4, e_5 \right), \adj \right)} = \overbrace{H_{1, 4} \mathbin\Vert H_{6, 4}}^{\trifunc{\Gamma} \left( \left( e_1, r_4, e_6 \right), \adj \right)}
= \overbrace{H_{1, 3} \mathbin\Vert H_{6, 3}}^{\trifunc{\Gamma} \left( \left( e_1, r_3, e_6 \right), \adj \right)} = \overbrace{H_{1, 3} \mathbin\Vert H_{5, 3}}^{\trifunc{\Gamma} \left( \left( e_1, r_3, e_5 \right), \adj \right)}. \\
\end{gathered}
\end{equation*}

Suppose the score of $\left( e_u, r_c, e_v \right)$ utilizing such representation is $s_{u, c, v}$, we will have
\begin{equation*}
\begin{gathered}
s_{4, 4, 1} = s_{7, 4, 1} = s_{7, 3, 1} = s_{4, 3, 1}, \\
s_{5, 4, 1} = s_{6, 4, 1} = s_{6, 3, 1} = s_{5, 3, 1}. \\
\end{gathered}
\end{equation*}

If a model can distinguish $r_3$ and $r_4$, it should at least rank node $e_7$ higher than $e_6$ given head node $e_1$ and relation $r_3$ since this is a positive triplet in training.
Then, we will have $s_{7, 3, 1} > s_{6, 3, 1}$, since we already knew that $s_{7, 3, 1} = s_{7, 4, 1}, s_{6, 3, 1} = s_{6, 4, 1}$, we will also have $s_{7, 4, 1} > s_{6, 4, 1}$.
This means that we rank node $e_7$ higher than node $e_6$  given head node $e_1$ and relation $r_4$, however, this is incorrect since $\left( e_7, r_4, e_1) \right)$ is negative while $\left( e_6, r_4, e_1 \right)$ is positive.
In summary, if we use \ourequiv representation for triplet scoring in this specific example, there is no way for it to correctly rank $r_3$ and $r_4$ in the same time.
This shows that \ourequiv representation (even the most expressive) can face challenges for \ourtask on \ourgraph.
