# Supplementary material for: Double Equivariance for Inductive Link Prediction for Both New Nodes and New Relation Types
Source: arXiv:2302.01313 source file (2025-01-14)
Supplement: Supplementary file 14 [file synthetic_FD2.tex]

\subsubsection{A Synthetic Case Study for \OurModel}
\label{subsec:limit}

\begin{figure}[ht]
\centering
\includegraphics[width=.5\linewidth]{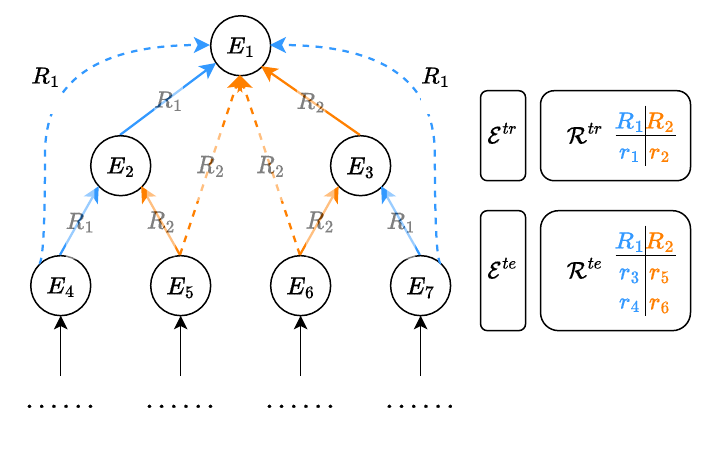}
\caption{
{\bf Synthetic Example of FD-2:} Training and test has their own node and relation type sets: $\cV\suptr \cap \cV\supte = \emptyset$ and $\cR\suptr \cap \cR\supte = \emptyset$.}
\label{fig:example-fd2}
\end{figure}

To further understand the expressive power and limitations of our proposed sturctural double equivariant model \OurModel, we create {\bf FD-2} to empirically justify the expressivity of our proposal on tasks over both new nodes and new relation types. On FD-2, training has 127 nodes and 2 relations, while test has 254 nodes and 4 relations (more nodes and more relations).

FD-2 is constructed by only a single rule, $\left( E_1, R_1, E_3 \right) \land \left( E_3, R_2, E_2 \right) \Rightarrow \left( E_1, R_1, E_3 \right)$ where $E_1, E_2, E_3$ and $R_1, R_2$ are all variables.
As illustrated in \Cref{fig:example-fd2}, The training data has only two relation types $\{r_1, r_2\}$, while test data has four relation types $\{r_3, r_4, r_5, r_6\}$ which are all different from training relations.
For all relation types, only $r_1, r_3, r_4$ can be used for $R_1$ assignments, and only $r_2, r_5, r_6$ can be use for $R_2$ assignments.
Besides, training and test also have distinct node sets.

Each graph (training or test) is consisted by one or more tree-like structures as left side of \Cref{fig:example-fd2}.
In each tree-like structure, all solid edges are used as observations, and will form a complete binary tree; 
while all dashed edges are used as training, validation or test samples which are built by applying the only rule over all observed edges.
In training, we have only one tree-like structure; while in test, we have two disconnected tree-like structures. A more detailed generation algorithm for a graph given depths of all tree-like structures is provided in \Cref{alg:synth-fd2}.

Since the structure of FD-2 does not satisfy the requirement of the spanning tree algorithm used in InGram~\citep{ingram}, we are not able to apply InGram and \OurOtherModel on FD-2. So we provide the results on FD-2 in \Cref{tab:exp-fd2-relation} with all remaining baselines and \OurModel. We can see that \OurModel clearly perform better than other baselines, especially in the relation prediction task, and shows capability to perform accurately on the \ourtask over both new nodes and new relation types, while methods like NBFNet and RMPI are not able to correctly perdict this task, even for node prediction.

\begin{table}[t!]
\centering
\centering
\captionof{table}{
{\bf Relation \& Node performance on \OurTask over FD2.} We report standard deviations over 5 runs. %
A higher value means better \ourtask performance. 
The best values are shown in bold font, while the second-best values are underlined. 
\OurModel  consistently achieve better results than the baselines, especially in the Relation perdiction task. NA* due to the fact that FD2 does not satisfy the spanning tree algorithm used in InGram~\citep{ingram}.
}
\resizebox{\linewidth}{!}{
\begin{tabular}{l r r r r c r r r r}
    & \multicolumn{4}{c}{Relation prediction $(i, ?, j)$} & & \multicolumn{4}{c}{Node prediction $(i, k, ?)$} \\
    
    \cmidrule{2-5} \cmidrule{7-10} 
    Models & MRR & Hits@1 & Hits@2 & Hits@4 & & MRR & Hits@1 & Hits@2 & Hits@4\\
    \midrule
    GAT & 7.61{\scriptsize $\pm 00.71$} & 0.77{\scriptsize $\pm 00.39$} & 2.78{\scriptsize $\pm 00.80$} & 5.85{\scriptsize $\pm 00.95$} & & 84.62{\scriptsize $\pm 02.64$} & 71.61{\scriptsize $\pm 04.94$} & \underline{93.51}{\scriptsize $\pm 01.03$} & 99.72{\scriptsize $\pm 00.27$}  \\
    GIN & 8.44{\scriptsize $\pm 00.40$} & 1.29{\scriptsize $\pm 00.37$} & 3.51{\scriptsize $\pm 00.58$} & \underline{7.18}{\scriptsize $\pm 01.01$} & & 73.99{\scriptsize $\pm 09.60$} & 65.73{\scriptsize $\pm 06.58$} & 76.69{\scriptsize $\pm 12.44$} & 81.45{\scriptsize $\pm 15.80$} \\
    GraphConv & 7.88{\scriptsize $\pm 00.45$} & 0.81{\scriptsize $\pm 00.29$} & 2.62{\scriptsize $\pm 00.61$} & 6.98{\scriptsize $\pm 01.09$} & & \underline{85.95}{\scriptsize $\pm 00.77$} & \underline{74.52}{\scriptsize $\pm 01.81$} & 92.66{\scriptsize $\pm 01.02$} & \textbf{99.84}{\scriptsize $\pm 00.15$}\\
    RMPI & \underline{9.09}{\scriptsize $\pm 03.18$} & \underline{1.94}{\scriptsize $\pm 01.88$} & \underline{3.95}{\scriptsize $\pm 04.43$} & 7.10{\scriptsize $\pm 05.58$} & & 21.16{\scriptsize $\pm 05.85$} & 9.84{\scriptsize $\pm 05.04$} & 16.74{\scriptsize $\pm 06.50$} & 27.98{\scriptsize $\pm 09.96$} \\
    NBFNet & 6.39{\scriptsize $\pm 02.19$} & 1.50{\scriptsize $\pm 02.49$} &1.79{\scriptsize $\pm 02.39$} & 2.91{\scriptsize $\pm 02.22$}&  & 21.95{\scriptsize $\pm 04.14$} & 14.44{\scriptsize $\pm 04.34$}  & 18.61{\scriptsize $\pm 04.29$} & 26.47{\scriptsize $\pm 04.24$} \\
    InGram &  N/A* & N/A* &N/A* & N/A*&  &  N/A* & N/A* &N/A* & N/A*\\
    \midrule
    
    \OurOtherModel (Ours) & N/A* & N/A* &N/A* & N/A*&  &  N/A* & N/A* &N/A* & N/A* \\
    
    \OurModel (Ours) & \textbf{44.39}{\scriptsize $\pm 12.17$} & \textbf{32.82}{\scriptsize $\pm 12.69$} & \textbf{38.71}{\scriptsize $\pm 13.60$} & \textbf{50.73}{\scriptsize $\pm 14.04$} & & \textbf{90.98}{\scriptsize $\pm 03.55$} & \textbf{83.59}{\scriptsize $\pm 06.22$} & \textbf{95.69}{\scriptsize $\pm 02.34$} & \underline{99.72}{\scriptsize $\pm 00.27$} \\ \\
    % \update{\OurNewModel (Ours)} & 
\end{tabular}
}
\vspace{5pt}
%\vspace{-20pt}
\label{tab:exp-fd2-relation}
\end{table}

% \begin{table}[t!]
% \centering
% %
% \resizebox{0.6\linewidth}{!}{
% \begin{tabular}{l|cccc}
%     \hline
%     \multirow{2}{*}{Model} & \multicolumn{4}{c}{FD-2} \\
%     \cline{2-5}
%     & MRR$\uparrow$ & Hits@1$\uparrow$ & Hits@2$\uparrow$ & Hits@4$\uparrow$ \\
%     \hline
% GAT & 11.80 & ~~1.80 & ~~5.20 & 12.10 \\
% GIN & 12.30 & ~~1.60 & ~~4.80 & 11.10 \\
% GraphConv & 13.40 & ~~2.60 & ~~5.60 & 14.50 \\
% NBFNet* & 13.50 & ~~4.70 & ~~8.10 & 15.70 \\
% \hline
% ISDEA & \textbf{68.30} & \textbf{52.40} & \textbf{68.10} & \textbf{87.90} \\
% \hline
% \end{tabular}
% }
% \vspace{5pt}
% \caption{\textbf{Node Inductive \ourtask over both new nodes and new relation types performance on Family Diagrams 2.} Existing baselines clearly struggle to perform the task.\yangze{change description}}
% %\vspace{-20pt}
% \label{tab:exp-fd2-node}
% \end{table}

%\vspace{-20pt}
\begin{algorithm}
\caption{{\bf Synthesis Algorithm for FD-2.} This is triplet generation code for a single graph (either training and test). It will provide observation and query triplets. For training, query triplets are further divided into training and validation triplets; For test, query triplets directly become test triplets.}
\label{alg:synth-fd2}
\begin{algorithmic}[1]
\Require Tree depth $\{D_1, \ldots, D_M\}$, Node Labeling ``$\text{Names}^\text{nd}$'', Relation Type Labeling ``$\text{Names}^\text{rl}$''.
\Ensure Observation triplets $\cS$, Query triplets $\cQ$
\State $\cS = \emptyset$
\State $\cQ = \emptyset$
\State $n \leftarrow 0$
\For{$m \leftarrow 1, \ldots, M$}
    \For{$d \leftarrow 1, \ldots, D_m$}
        \For{$v \leftarrow 2^d - 1, \ldots, 2^{d + 1} - 2$}
            \State $u_1 \leftarrow \lceil \sfrac{(v - 2)}{2} \rceil$
            \State $u_2 \leftarrow \lceil \sfrac{(u_1 - 2)}{2} \rceil$
            \If{$v \text{ mod } 2 = 0$}
                \Comment{For relation type variable $R_2$.}
                \If{$u_1 \geq 0$}
                    \State $\cS$.add$\big(\,(\text{Names}^\text{nd}[n + v], \text{Names}^\text{rl}[2m - 1], \text{Names}^\text{nd}[n + u_1])\,\big)$
                \EndIf
                \If{$u_2 \geq 0$}
                    \State $\cQ$.add$\big(\,(\text{Names}^\text{nd}[n + v], \text{Names}^\text{rl}[2m - 1], \text{Names}^\text{nd}[n + u_2])\,\big)$
                \EndIf
            \Else
                \Comment{For relation type variable $R_1$.}
                \If{$u_1 \geq 0$}
                    \State $\cS$.add$\big(\,(\text{Names}^\text{nd}[n + v], \text{Names}^\text{rl}[2m - 2], \text{Names}^\text{nd}[n + u_1])\,\big)$
                \EndIf
                \If{$u_2 \geq 0$}
                    \State $\cQ$.add$\big(\,(\text{Names}^\text{nd}[n + v], \text{Names}^\text{rl}[2m - 2], \text{Names}^\text{nd}[n + u_2])\,\big)$
                \EndIf
            \EndIf
        \EndFor
        \State $n \leftarrow n + 2^d$
    \EndFor
\EndFor
\end{algorithmic}
\end{algorithm}
%\vspace{-20pt}

\subsubsection{Expressivity Limitation Case Study with FD-2 for \OurModel}
\label{subsubsec:limit}
We now provide a FD-2 variant where we show that \ourequiv representation is not expressive enough to solve a specific task. It is a simple 2-depth tree structure as shown in \Cref{fig:example-limit}.
We denote node representations given by arbitrary \ourequiv representation as $H_{v, r}$ where $v \in [1, 7]$ and $r \in [1, 4]$. We can easily notice that $e_4$ and $e_7$ are symmetric, $e_5$ and $e_6$ are symmetric (simply flipping blue and orange colors), thus we will expect $H_{4, 1} = H_{7, 2}, H_{4, 2} = H_{7, 1}, H_{5, 1} = H_{6, 2}, H_{5, 2} = H_{6, 1}$.

\begin{figure}[h]
\centering
\includegraphics[width=0.3\linewidth]{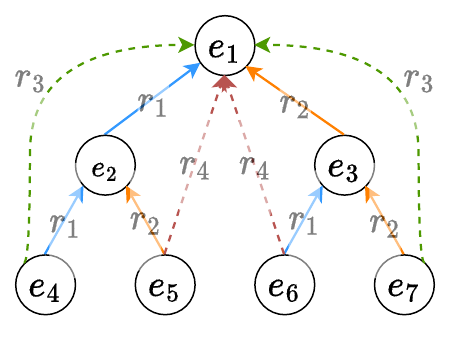}
\caption{
{\bf Expressivity Limitation:} Relation $r_1$ and $r_2$ are always observed, while $r_3$ and $r_4$ are always querying. $r_3$ implies that relation types on the path are same, while $r_4$ implies that relation types on the path are different..}
\label{fig:example-limit}
\end{figure}

Since there is no $r_3$ and $r_4$ in observation, they are freely exchangeable with each other, thus we will also expect 
\begin{equation*}
\begin{gathered}
H_{1, 3} = H_{1, 4}, \\
H_{4, 3} = H_{4, 4} = H_{7, 4} = H_{7, 3}, \\
H_{5, 3} = H_{5, 4} = H_{6, 4} = H_{6, 3}. \\
\end{gathered}
\end{equation*}

After getting all those representations, we can now focus on querying triplet representations (dashed green and red) by concatenating head and tail node representations w.r.t. relation types:
\begin{equation*}
\begin{gathered}
\trifunc{\Gamma} \left( \left( e_1, r_4, e_4 \right), \adj \right) = H_{1, 4} \mathbin\Vert H_{4, 4}, \\
\trifunc{\Gamma} \left( \left( e_1, r_3, e_5 \right), \adj \right) = H_{1, 3} \mathbin\Vert H_{5, 3}, \\
\trifunc{\Gamma} \left( \left( e_1, r_3, e_6 \right), \adj \right) = H_{1, 3} \mathbin\Vert H_{6, 3} ,\\
\trifunc{\Gamma} \left( \left( e_1, r_4, e_7 \right), \adj \right) = H_{1, 4} \mathbin\Vert H_{7, 4}. \\
\end{gathered}
\end{equation*}

We can notice that
\begin{equation*}
\begin{gathered}
\overbrace{H_{1, 4} \mathbin\Vert H_{4, 4}}^{\trifunc{\Gamma} \left( \left( e_1, r_4, e_4 \right), \adj \right)} = \overbrace{H_{1, 4} \mathbin\Vert H_{7, 4}}^{\trifunc{\Gamma} \left( \left( e_1, r_4, e_7 \right), \adj \right)}
= \overbrace{H_{1, 3} \mathbin\Vert H_{7, 3}}^{\trifunc{\Gamma} \left( \left( e_1, r_3, e_7 \right), \adj \right)} = \overbrace{H_{1, 3} \mathbin\Vert H_{4, 3}}^{\trifunc{\Gamma} \left( \left( e_1, r_3, e_4 \right), \adj \right)}, \\
\overbrace{H_{1, 4} \mathbin\Vert H_{5, 4}}^{\trifunc{\Gamma} \left( \left( e_1, r_4, e_5 \right), \adj \right)} = \overbrace{H_{1, 4} \mathbin\Vert H_{6, 4}}^{\trifunc{\Gamma} \left( \left( e_1, r_4, e_6 \right), \adj \right)}
= \overbrace{H_{1, 3} \mathbin\Vert H_{6, 3}}^{\trifunc{\Gamma} \left( \left( e_1, r_3, e_6 \right), \adj \right)} = \overbrace{H_{1, 3} \mathbin\Vert H_{5, 3}}^{\trifunc{\Gamma} \left( \left( e_1, r_3, e_5 \right), \adj \right)}. \\
\end{gathered}
\end{equation*}

Suppose the score of $\left( e_u, r_c, e_v \right)$ utilizing such representation is $s_{u, c, v}$, we will have
\begin{equation*}
\begin{gathered}
s_{4, 4, 1} = s_{7, 4, 1} = s_{7, 3, 1} = s_{4, 3, 1}, \\
s_{5, 4, 1} = s_{6, 4, 1} = s_{6, 3, 1} = s_{5, 3, 1}. \\
\end{gathered}
\end{equation*}

If a model can distinguish $r_3$ and $r_4$, it should at least rank node $e_7$ higher than $e_6$ given head node $e_1$ and relation $r_3$ since this is a positive triplet in training.
Then, we will have $s_{7, 3, 1} > s_{6, 3, 1}$, since we already knew that $s_{7, 3, 1} = s_{7, 4, 1}, s_{6, 3, 1} = s_{6, 4, 1}$, we will also have $s_{7, 4, 1} > s_{6, 4, 1}$.
This means that we rank node $e_7$ higher than node $e_6$  given head node $e_1$ and relation $r_4$, however, this is incorrect since $\left( e_7, r_4, e_1) \right)$ is negative while $\left( e_6, r_4, e_1 \right)$ is positive.
In summary, if we use \ourequiv representation for triplet scoring in this specific example, there is no way for it to correctly rank $r_3$ and $r_4$ in the same time.
This shows that \ourequiv representation (even the most expressive) can face challenges for \ourtask on \ourgraph.
