# Supplementary material for: Double Equivariance for Inductive Link Prediction for Both New Nodes and New Relation Types
Source: arXiv:2302.01313 source file (2025-01-14)
Supplement: Supplementary file 15 [file appdx-additional-example.tex]

\section{Additional Example for \OurTask}
\label{appd:add-example}

\begin{wrapfigure}{r}{0.55\textwidth}
\centering
\includegraphics[width=\linewidth]{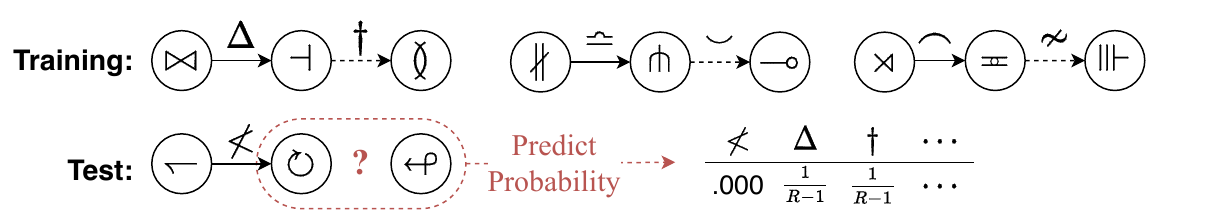}
\caption{
{\bf Alien \ourgraph:}
The task is to predict the missing relation ``?'' in red.
Training only tells us that relations do not repeat in a path.}
\label{fig:example-guess}
\end{wrapfigure}
This example depicts an even harder scenario than the example in 
\Cref{fig:example-link}, obtained from a fictional alien civilization.
Knowing nothing about alien languages, we note that in training, all adjacent relations are different. Minimally, we could predict the missing relation in red in test data is not ``$\nless$''. By introducing equivariance in relations, it is possible for a model to predict relation types uniformly over the set of other ($R\!-\!1$) relations except for the existing relation ``$\nless$'', which is all we know about the aliens.  
